# Supplementary material for: Analyzing Neural Jacobian Methods in Applications of Visual Servoing and Kinematic Control
Source: arXiv:2106.06083 source file (2021-06-10)
Supplement: Supplementary file 1 [file appendix.tex]

\section*{Appendix}
\addcontentsline{toc}{section}{Appendices}
\section{Experiment Details}

\begin{table}[]
\centering
{\small
\begin{tabular}{c|c|c|c|}
\cline{2-4}
\textbf{}         & \textbf{Single  Point (Simulation)} & \textbf{Multi-Point (Simulation)} & \multicolumn{1}{l|}{\textbf{Single Point (Kinova)}} \\ \hline
\multicolumn{1}{|l|}{\# of Training Epochs} & 30                                  & 40                                & 45                                                  \\ \hline
\multicolumn{1}{|c|}{\# Hidden Layers}      & 2                                   & 4                                 & 1                                                   \\ \hline
\multicolumn{1}{|c|}{Hidden Layer Size}     & \multicolumn{3}{c|}{100}                                                                                                      \\ \hline
\multicolumn{1}{|c|}{Activation Function}   & \multicolumn{3}{c|}{Relu}                                                                                                     \\ \hline
\end{tabular}
}
\caption{Neural network hyperparameters for each experiment. }
\label{tab:networkparams}
\end{table}

\begin{table}[]
\begin{tabular}{|c|c|c|c|}
\hline
\textbf{Single Point Distances} & \textbf{Counts} & \textbf{Multi-point Distances} & \textbf{Counts} \\ \hline
0.0 - 0.5                       & 106             & 0.0 - 1.0                      & 96              \\ \hline
0.5 - 1.0                       & 414             & 1.0 - 2.0                      & 393             \\ \hline
1.0 - 1.5                       & 455             & 2.0 - 3.0                      & 464             \\ \hline
1.5 - 2.0                       & 125             & 3.0 - 4.0                      & 147             \\ \hline
\end{tabular}
\caption{Trajectory counts for simulation experiments by initial distances to target}
\end{table}

In this section, we provide additional details on our experimental step-up. We list our neural network hyperparameters in Table~\ref{tab:networkparams}. We used the Adam optimizer for all experiments with $\beta_{1}=0.9$, $\beta_{2}=0.999$, and learning rate $\alpha=0.001$. These were the default parameters in the deep learning framework we implemented our methods with \cite{paszke2019pytorch}. In all our experiments we used a mini-batch size of 32 for training all neural methods.

We collected trajectories as training data for each experiment. We ran an Ornstein and Uhlenbeck process \cite{uhlenbeck1930brownianmotion} with the following parameters: $\sigma=1.00$, $\mu=0.00$, $\theta=0.15$, $\theta$ here is not the same as model parameters. In our single point simulation, we used a training dataset of 100,000 (1000 trajectories of 100 time-steps each), and for the multi-point environment we used a training dataset of 200,000 (2000 trajectories of 100 times-steps). We re-used each random seeds training dataset for all models in our experiments. The one exception is the Neural Jacobian models which collected additional trajectories before training because each datum required sub-sequent steps to formulate a training example. 

For evaluation in both simulators, we generated 110 random targets for each of the 10 random seeds for a total of 1100 targets used for reported results. The targets were generated by uniform sampling in the joint angles and transforming them with the Kinova kinematics. This does not correspond with uniform sampling of the Cartesian work-space because of the transformations from the kinematic equations. We allowed each model 200 time-steps to reach the target which corresponded to 10 seconds of simulated time. In our experiments we set the gain value $\lambda=1.0$ which we found worked well for all methods.
 
 On the Kinova, we collected 10,000 training examples (100 trajectories of 100 time-steps) with the same Ornstein and Uhlenbeck process parameters. Unlike the simulator experiments, we re-used the same 10,000 samples for each random seed, meaning the random seed mostly affected initialization for the neural network parameters. We generated 25 random targets for each seed from the Kinova's kinematics bounded between $[-2.0, 2.0]$ for the first control joint and $[-1.5, 1.5]$ of the second joint. We only worked with 2 Joints of the Kinova, and discuss details of this in the next section. Targets were reused between all models considered. During evaluation, we used a gain $\lambda=0.9$ for for evaluation, but collected data with $\lambda = 1.0$.
\section{Environment Details}

\begin{table}[]
\centering
\begin{tabular}{c|c|c|c|c|c|c|}
\cline{2-7}
\textbf{}                                            & \textit{\textbf{$x$}} & \textit{\textbf{$\cos(q)$}} & \textit{\textbf{$\sin(q)$}} & \textit{\textbf{$\dot{q}$}} & \textit{\textbf{$x^{*}$}} & \textit{\textbf{$s$}} \\ \hline
\multicolumn{1}{|c|}{\textit{\textbf{Single Point}}} & 3                     & 7                           & 7                           & 7                           & 3                         & 27                    \\ \hline
\multicolumn{1}{|c|}{\textit{\textbf{Multi Point}}}  & 12                    & 7                           & 7                           & 7                           & 12                        & 45                    \\ \hline
\multicolumn{1}{|c|}{\textit{\textbf{Kinova}}}       & 2                     & 2                           & 2                           & 2                           & 2                         & 10                    \\ \hline
\end{tabular}
\caption{Dimensions of different aspects of the robot state $s$ for each environment. This includes end-effector location $x$, joint angles $q$, joint velocities $\dot{q}$, and target location $x^{*}$, where $s$ is the sum of these dimensions. Commands sent to the environments were joint velocities $\dot{q}$.}
\label{tab:statedimensions}
\end{table}
We describe the details for our simulated and robotic environments in this section. All our environments are designed similarly to a reinforcement learning gym \cite{brockman2016OpenAIGYM} where the actions are joint velocities $\dot{q}$ and we receive the robot state as a vector $s$. Each environment consists of the same robotic information, only differing in the dimensions of each feature. We list these dimensions for each environment in Table~\ref{tab:statedimensions}.

In both simulated and robotic environments, we utilize the Kinova's kinematics equations for generating the location of targets. As mentioned in the background section, we used the Denavit-Hartenberg (DH) parameters for the Kinova's kinematics. The DH matrix is as follows:
\begin{equation}
 ^{i-1}T_{i} =
\begin{pmatrix}
 \cos(q_{i}) & -\cos(\alpha_{i})\sin(q_{i}) & \sin(\alpha_{i})\sin(q_{i}) & a_{i}\cos(q_{i})\\
 \sin(q_{i}) & \cos(\alpha_{i})\cos(q_{i}) & -\sin(\alpha_{i})\cos(q_{i}) & a_{i}\sin(q_{i})\\
 0 & \sin(\alpha_{i}) & \cos(\alpha_{i}) & d_{i}\\
 0 & 0 & 0 & 1 
\end{pmatrix}.
\end{equation}
For each transformation $^{i-1}T_{i}$ of the Kinova, the values can be found in Table~\ref{tab:kinovadhvalues}. 

\begin{figure}[ht]
\begin{subfigure}{.5\textwidth}
  \centering
  % include first image
  \includegraphics[width=.7\linewidth]{./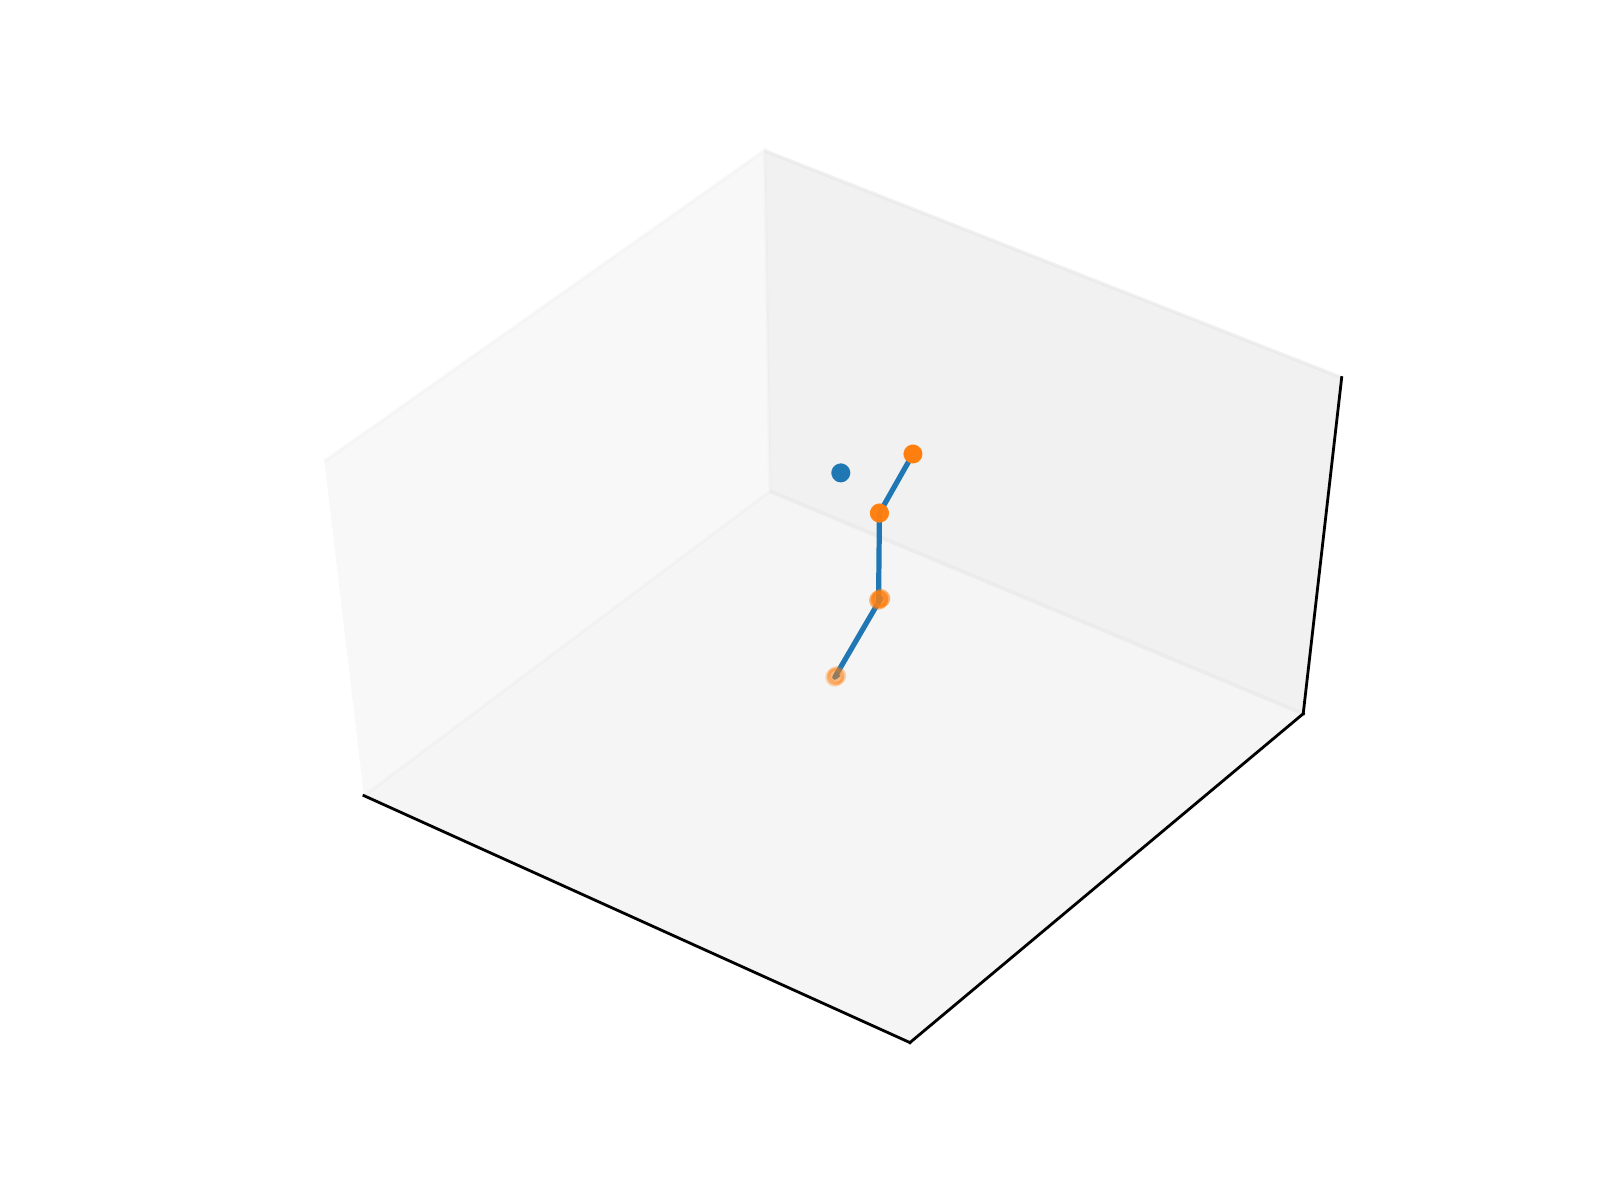}  
  \caption{Point to Point Environment}
  \label{fig:1ptsimulator}
\end{subfigure}
\begin{subfigure}{.5\textwidth}
  \centering
  % include second image
  \includegraphics[width=.7\linewidth]{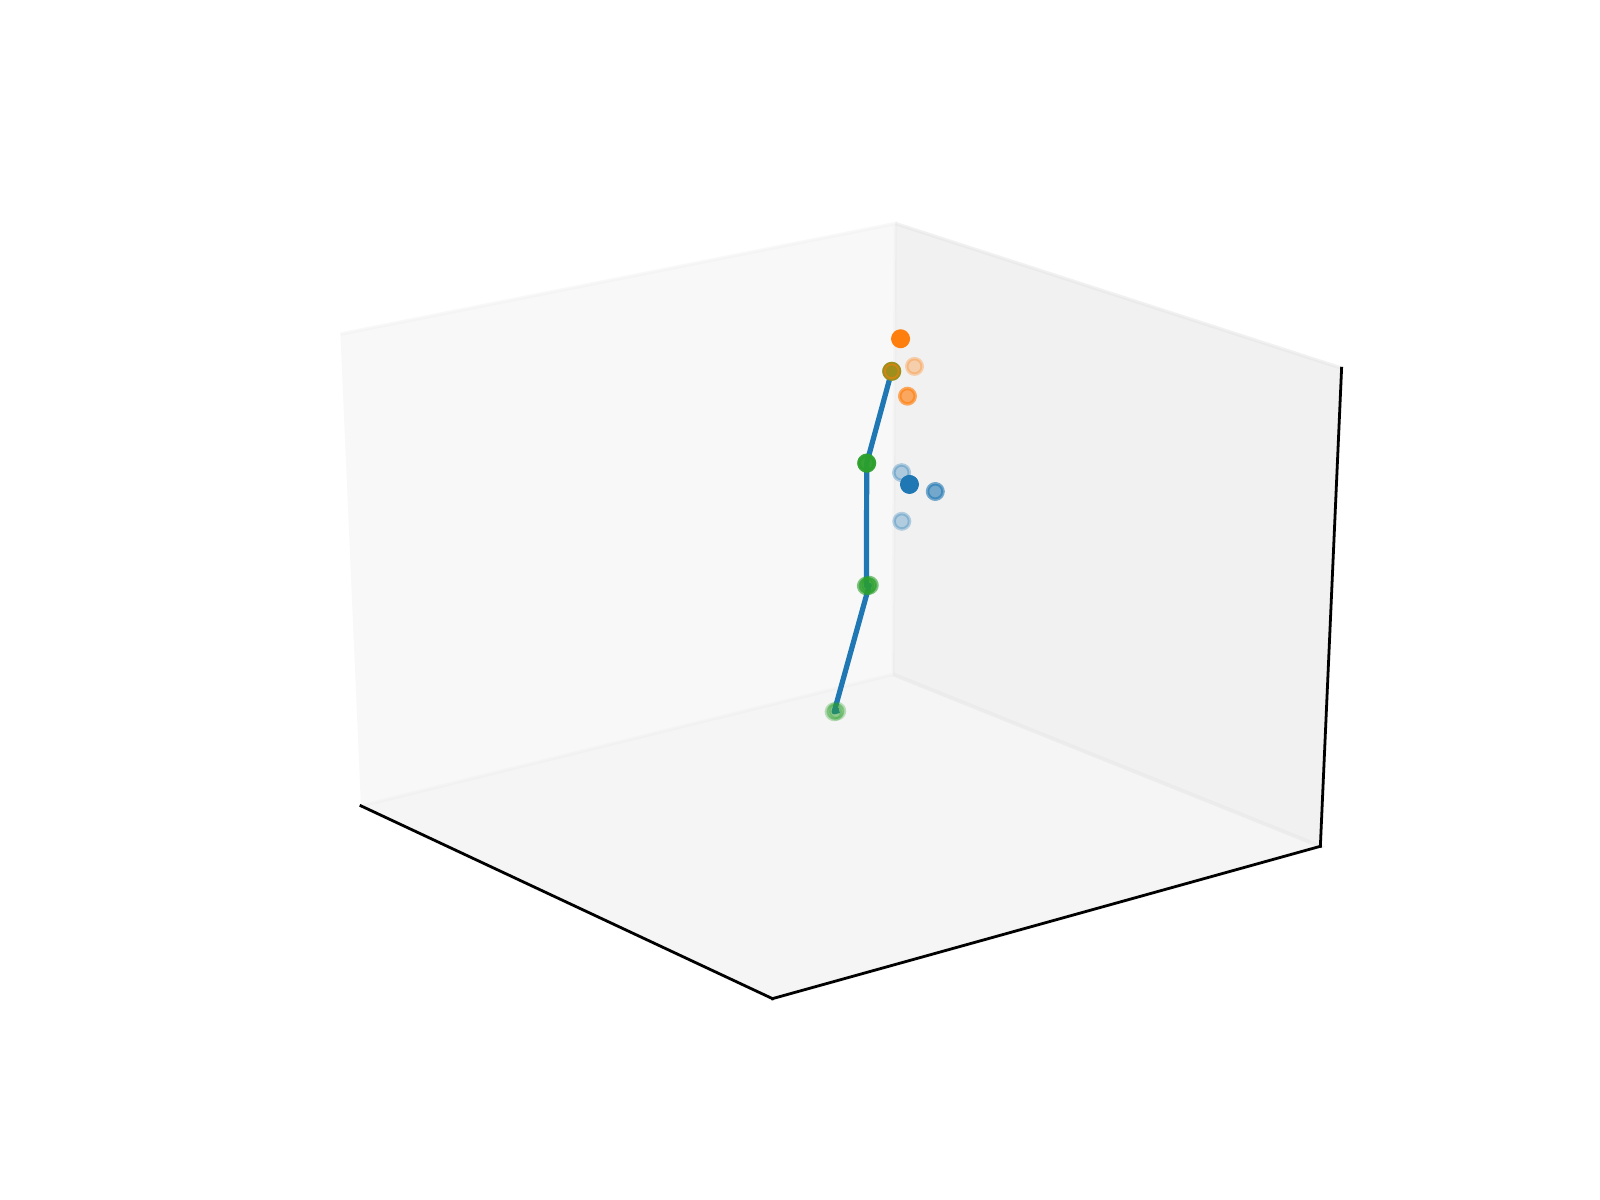}  
  \caption{Position and Orientation Environment}
  \label{fig:4ptsimulator}
\end{subfigure}
\caption{Visualization of kinematic simulators. The objective in both simulators is to align robot points (orange) to match exactly with corresponding target points (blue) }
\label{fig:simulators}
\end{figure}

\paragraph{Simulator Details} Our simulator environments are visualized in Figure~\ref{fig:simulators}, and were implemented with the DH parameter values in Table~\ref{tab:kinovadhvalues}. They only differ in the number of points we wish to move to a target position. In the single point case, we only translate a single homogeneous vector $p=[0,0,0,1]$ with the kinematics equations to represent the end-effector. In the multi-point case we include 3 additional vectors, where each is a scaled unit-vectors of the orientation for the x, y, and z axis. We found using one-tenth of a unit vector the best for visualizing the points representing orientation (e.g. $p_{z}=[0, 0, .1, 1]$ as opposed to $p_{z}=[0, 0, 1, 1]$). When joint velocities are sent, the current joint values are updated as $q_{t+1} = q_{t} + \Delta t \dot{q_{t}}$, where $\Delta t=0.05 \text{(seconds)}$ represents our simulated time. The position of the robot is then updated and a new state vector is sent with the updated information to our controller.

\begin{table}[]
\centering
\begin{tabular}{|c|c|c|c|c|}
\hline
\textbf{i}    & \textbf{$\alpha_{i}$ (radians)} & \textbf{$a_{i}$(m)} & \textbf{$d_{i}$(m)} & \textbf{$q_{i}$ (radians)} \\ \hline
0 (from base) & $\pi$                           & 0.0                 & 0.0                 & 0                               \\ \hline
1             & $\pi / 2$                       & 0.0                 & -(0.1564 + 0.1284)  & $q_{1}$                         \\ \hline
2             & $\pi / 2$                       & 0.0                 & -(0.0054 + 0.0064)  & $q_{2} + \pi$                   \\ \hline
3             & $\pi / 2$                       & 0.0                 & -(0.2104 + 0.2104)  & $q_{3} + \pi$                   \\ \hline
4             & $\pi / 2$                       & 0.0                 & -(0.0064 + 0.0064)  & $q_{4} + \pi$                   \\ \hline
5             & $\pi / 2$                       & 0.0                 & -(0.2084 + 0.1059)  & $q_{5} + \pi$                   \\ \hline
6             & $\pi / 2$                       & 0.0                 & 0.0                 & $q_{6} + \pi$                   \\ \hline
7             & $\pi$                           & 0.0                 & -(0.1059 + 0.0615)  & $q_{7} + \pi$                   \\ \hline
\end{tabular}
\caption{Table of DH parameter values for the Kinova robot \cite{kinova}. We utilize these numbers for calculating the target location, position of our simulators, and for calculating the true Jacobian.}
\label{tab:kinovadhvalues}
\end{table}

\paragraph{Kinova Details}
\begin{figure}
    \centering
    \includegraphics[width=.3\linewidth]{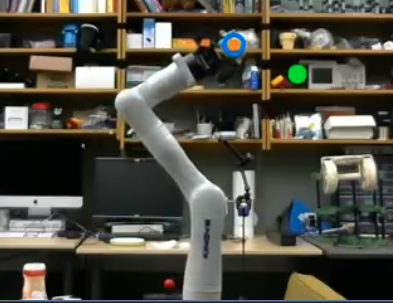}
    \caption{Image of the Kinova Gen 3 light robot used for experiments. Visualization of the tool tip (blue orange circle) and target position (green) in image are to illustrate fundamental idea of the control task. In experiments we work in robot coordinate system.}
    \label{fig:Kinova}
\end{figure}

For our Kinova experiments, we derived the DH parameters for a 2 degree-of-freedom (DOF) planar manipulator. The kinematic transformations can be found in \citet[Chapter 3]{craig1989IntroRobotics} for this planar case. This required transforming the Kinova's coordinate system to align with our planar forward kinematics equations. Specifically, we converted from the Kinova's z-x plane to a x-y coordinate frame, by subtracting an offset of 0.7052 from the Z axis and treated it as our X coordinates while treating the Kinova x coordinate as our y axis. We then interpreted the Kinova's 4th link of length 0.3143 meters as the first link in our 2-DOF robot,  and the Kinova's 6th joint of length 0.1774 meters as the second link. We interacted with the Kinova using the publicly available the Kinova Robotic Operating System (ROS) bindings \cite{ros2018ROS,kinovakortex}. The all features of the robot's state was sensory information from the Kinova. Similarly, joint velocity commands were sent through the ROS bindings. We operated our the Kinova at approximately 20 Hz which corresponded to about 10 seconds for real-time evaluation on the robot per trajectory. 
\section{Baseline Methods}
In this section, we describe the details of each of the baseline methods we compared against. This included the true Jacobian, finite difference method~\cite{jagersand96visualservoing}, the Broyden method~ \cite{jagersand96visualservoing}, and the Local Linear method \cite{farahmand2007globaluvs}. As the Broyden method and finite difference method are closely related, they are described together.

\subsection{True Robotic Jacobian}

Here we include relevant equations that describe the true Jacobian for the 2-DOF environment we mapped to the Kinova. With two planar rotation joints the position of the end-effector can be described by the following equations:
\begin{equation}
    x = 
        \begin{bmatrix}
         L_{1} cos(q_{1}) + L_{2} cos(q_{1} + q_{2})\\L_{1}sin(q_{1}) + L_{2} sin(q_{1} + q_{2})
        \end{bmatrix}
\end{equation}.

Using the equation for robotic motion in the main paper, when we  differentiate with respect to time, we get the following Jacobian: 
\begin{equation}
 \dot{x} =
        \begin{pmatrix}
         -L_{1}sin(q_{1}) - L_{2} sin(q_{1} + q_{2}) &
         - L_{2} sin(q_{1} + q_{2})
         \\
         L_{1} cos(q_{1}) + L_{2} cos(q_{1} + q_{2}) &
         L_{2} cos(q_{1} + q_{2})
        \end{pmatrix}
        \begin{pmatrix}
            \dot{q_{1}} \\  \dot{q_{2}}
        \end{pmatrix} 
\end{equation}
Here, $L_{1}$ and $L_{2}$ our the lengths of the robot links. We exclude writing $J^k{-1}$, but note that it can be found analytically using the fact $J$ is a 2-by-2 matrix. For our simulators, we found that analytically writing the Jacobian would be fairly complex for the 7 DOF manipulator, and instead we used a backpropagation library to handle calculating the Jacobian \cite{jax2018github}.

\subsection{k Nearest Neighbor Local Linear Jacobian Estimation}
Previous research on Jacobian approximation has utilized the observation that the Jacobian is a hyperplane at the instantaneous point of evaluation \cite{farahmand2007globaluvs}. This work considered directly fitting such a hyper-plane utilizing the assumption that the equations of robot motion can be approximated as finite differences $\Delta x \approx J(q_{t}) \Delta q$ for time step $t$ in a trajectory, leading to the following objective: 
\begin{equation}
    \min_{J} \sum^{k}_{i=1}\sum^{k}_{j=1}|| \Delta x_{ij} - J\Delta q_{ij} ||_{2}^{2},
\end{equation}
where $\Delta x_{ij}$ and $\Delta q_{ij}$ are the finite difference between the k-nearest neighbor (k-NN) points to the current angles $q_{t}$ we want to calculate the Jacobian. This objective function is then optimized online when controlling the robot, and can be anlytically solved by differentiating with respect to the Jacobian J. This method requires storing all the interactions with the robot to select the k-NN neighbors to be optimized over. In our experiments we used $k=50$ for evaluation based on previous works experimental results \cite{farahmand2007globaluvs}.

\subsection{Broyden Jacobian Estimation}

One classic approach to estimating the Jacobian is by making small, independent movements of each joint from some initial pose \cite{ramirez2018libraryUVS}. In a 2-DOF planar reaching environment, this matrix is found as follows:   
\begin{equation}
    J \approx \hat{J}=
    \begin{pmatrix}
        \frac{x^{t} - x^{0}}{q^{t}_{1} - q^{0}_{1}} & \frac{x'^{t} - x^{0}}{ q^{t}_{2} - q^{0}_{2}}\\[\jot]
        \frac{y^{t} - y^{0}}{q^{t}_{1} - q^{0}_{1}} & \frac{y'^{t} - y^{0}}{ q^{t}_{2} - q^{0}_{2}}\\[\jot]
    \end{pmatrix}.
\end{equation}
Here, $t$ is the position after some amount of movement. Note that, for each columns approximation we assume the same initial position $(x^{0}, y^{0})$. We only include the coordinates for a 2-dimensional point, but the matrix is similar for 3D points as well. For each column of this matrix, we move the joints sufficiently far such that the change in position is non-negligible. To improve the estimate of this Jacobian we can then make Broyden updates of the Jacobian as follows:
\begin{equation}
 \hat{J}_{k+1} = \hat{J}_{k} + \alpha \frac{(\Delta e - \hat{J}_{k}\Delta q) \Delta q^{T}}{||\Delta q||_{2}^{2}}.
\end{equation}
Here $\Delta$ is for changes from the last tracked measurements, and $e = x^{*} - x$. A limitation of the Broyden update is it requires the change in joint angles $\Delta q$ be sufficiently large. In our experiments for the Broyden method, we only take the update if $||\Delta q||_{2}^{2} \geq 0.01$ and used $\alpha=0.1$ when updating the approximation $\hat{J}_{k}$.  
\section{Multitask Jacobian Parameter Comparisons}

In this section we include additional results when we investigated tuning the weighting term $\beta$ for the Multitask Neural Jacobian. Our experimental set-up was the same as described previously for the simulators. We only consider comparing the Multitask Neural Jacobian against each other. When $\beta=0.0$ this is the same as the original Neural Jacobian. 

Decreases in the Euclidean distance (meters) to the target are visualized in Figure~\ref{fig:betatuningeuclideandist}. This plot suggests that increasing $\beta$ seems to help in the multi-point environment for the closer targets but overall differences are relatively minute. We also include the percentages of successes, which was calculated the same way for our other experiments, in Table~\ref{tab:tuningbetasuccesses}. These results show similar results reported in our main paper, where the main benefits of the Multitask Neural Jacobian seem more evident in the multi-point environment. For the single point case,  even for smaller $\beta$ negatively, impact performance.

\begin{figure}[ht]
\begin{subfigure}{.5\textwidth}
  \centering
  % include first image
  \includegraphics[width=\linewidth]{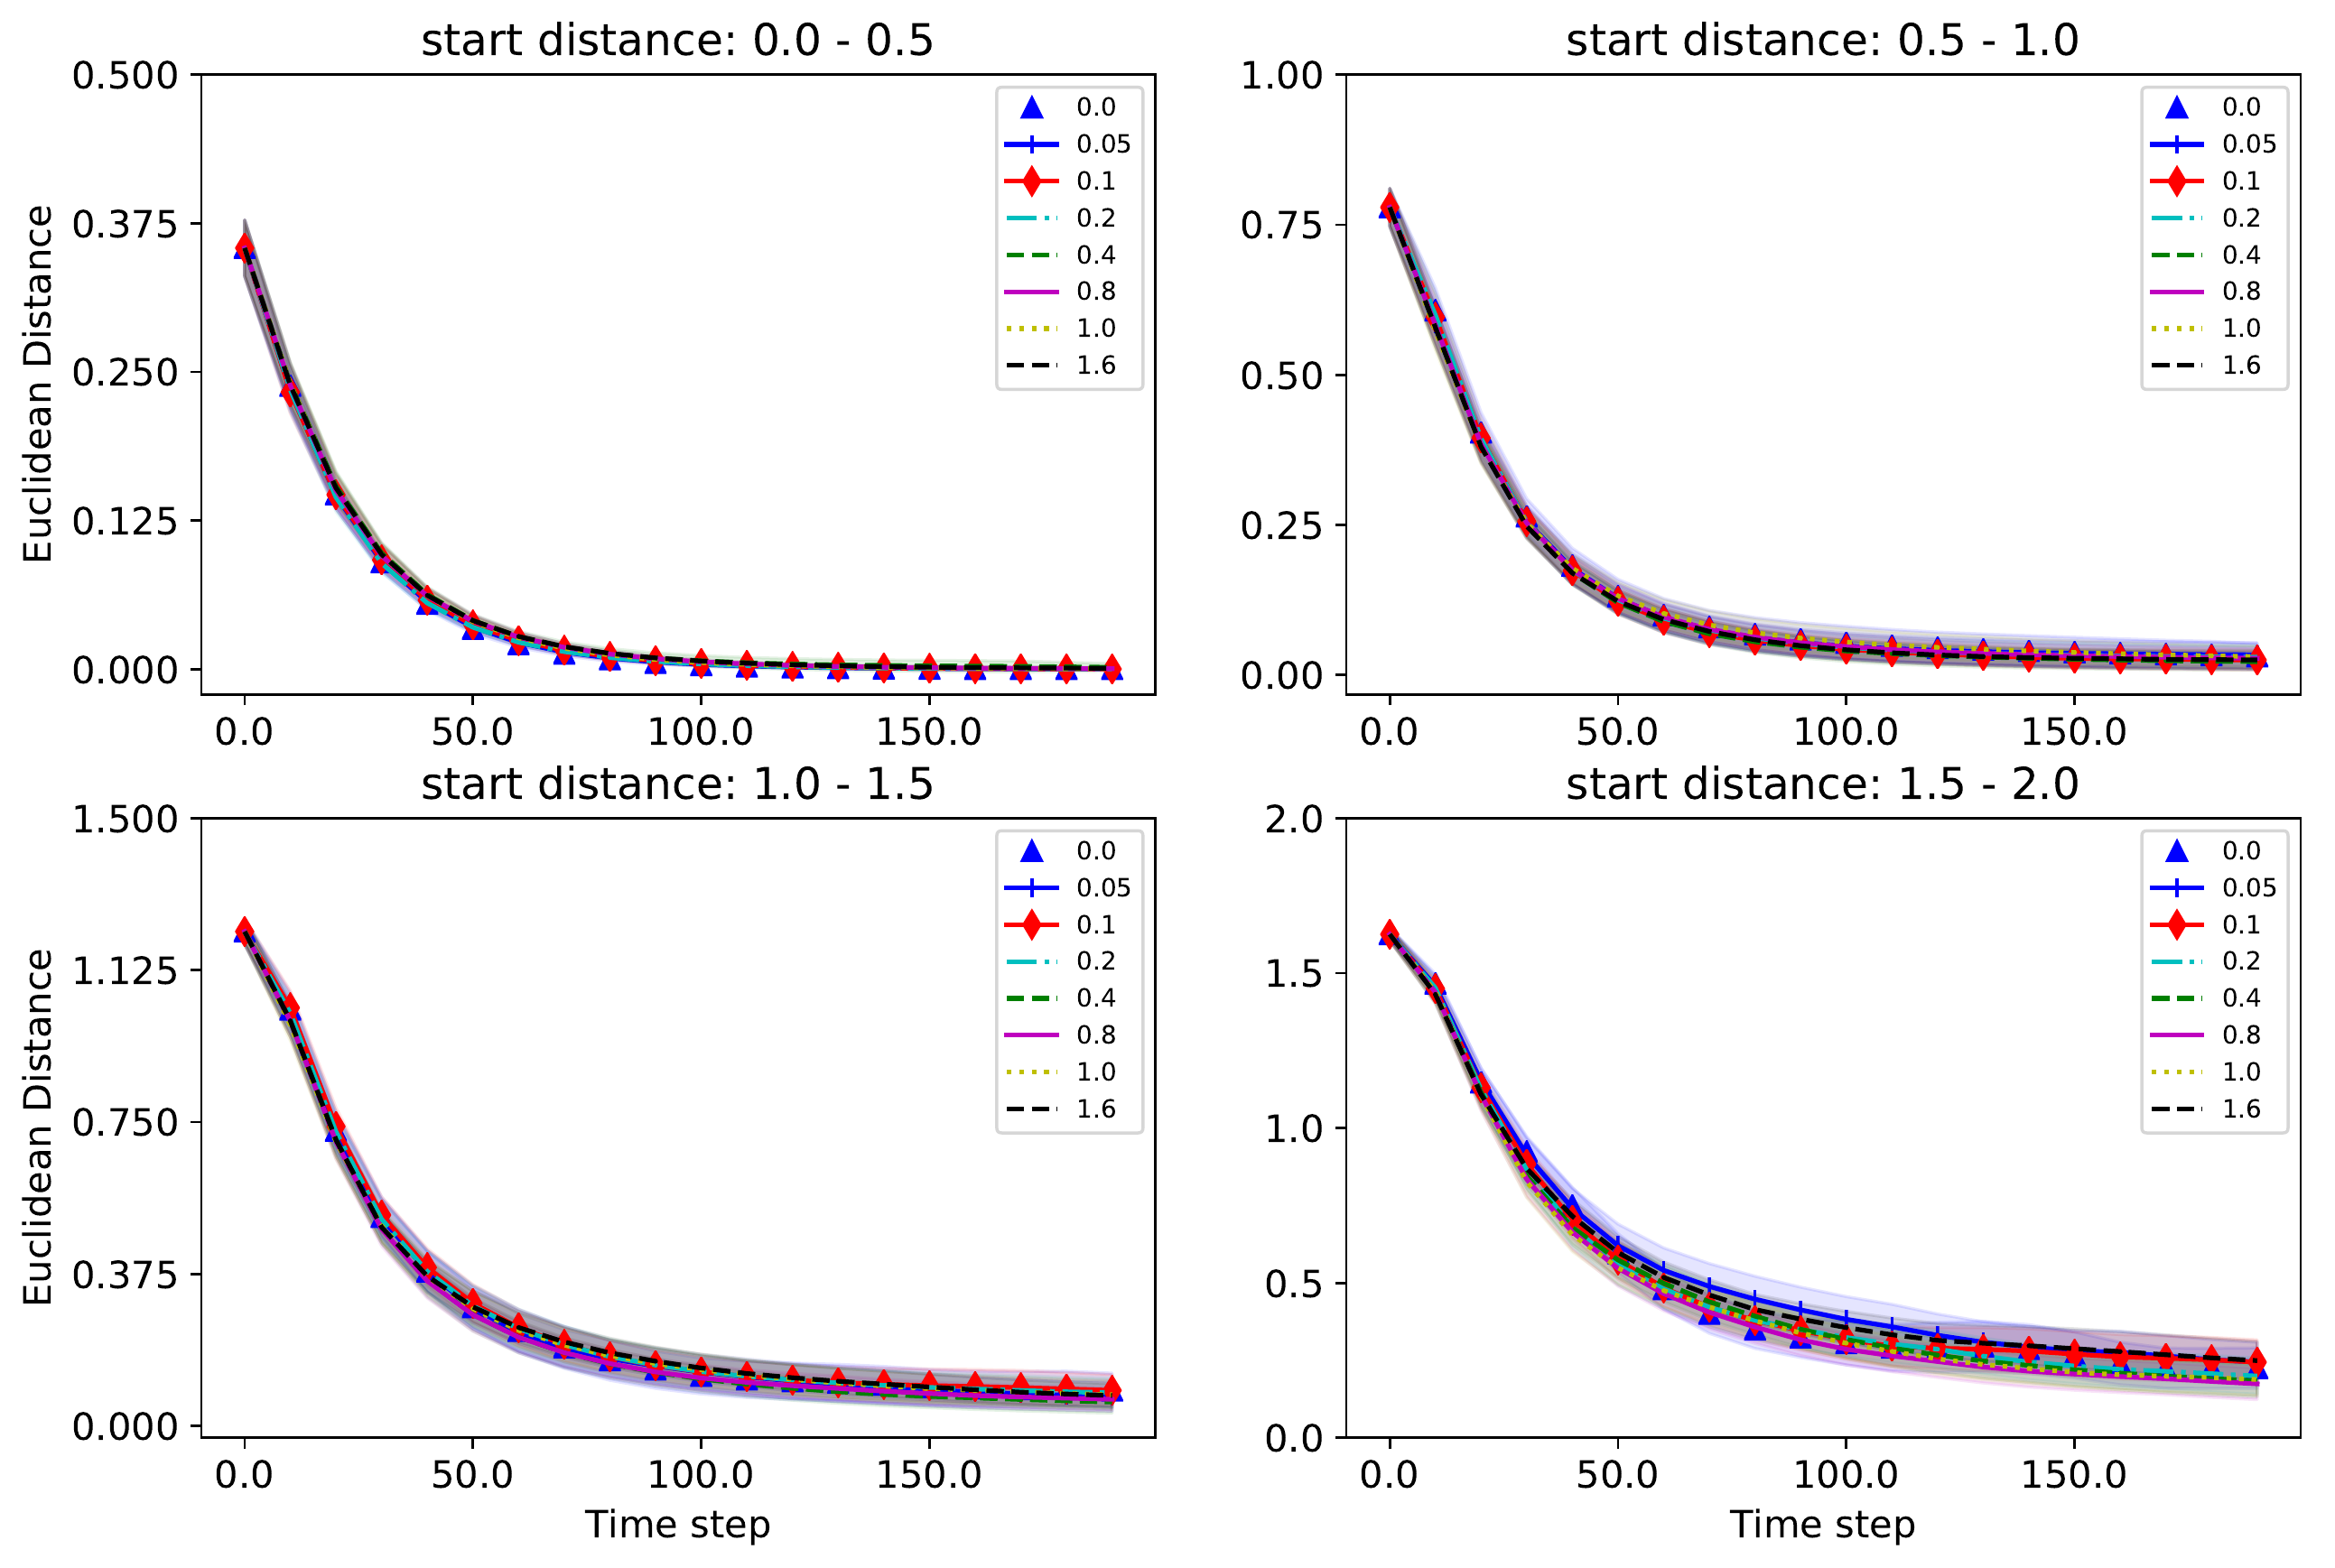}  
  \caption{Single Point Alignment}
  \label{fig:betatuningeuclideandistsinglepoint}
\end{subfigure}
\begin{subfigure}{.5\textwidth}
  \centering
  % include second image
  \includegraphics[width=\linewidth]{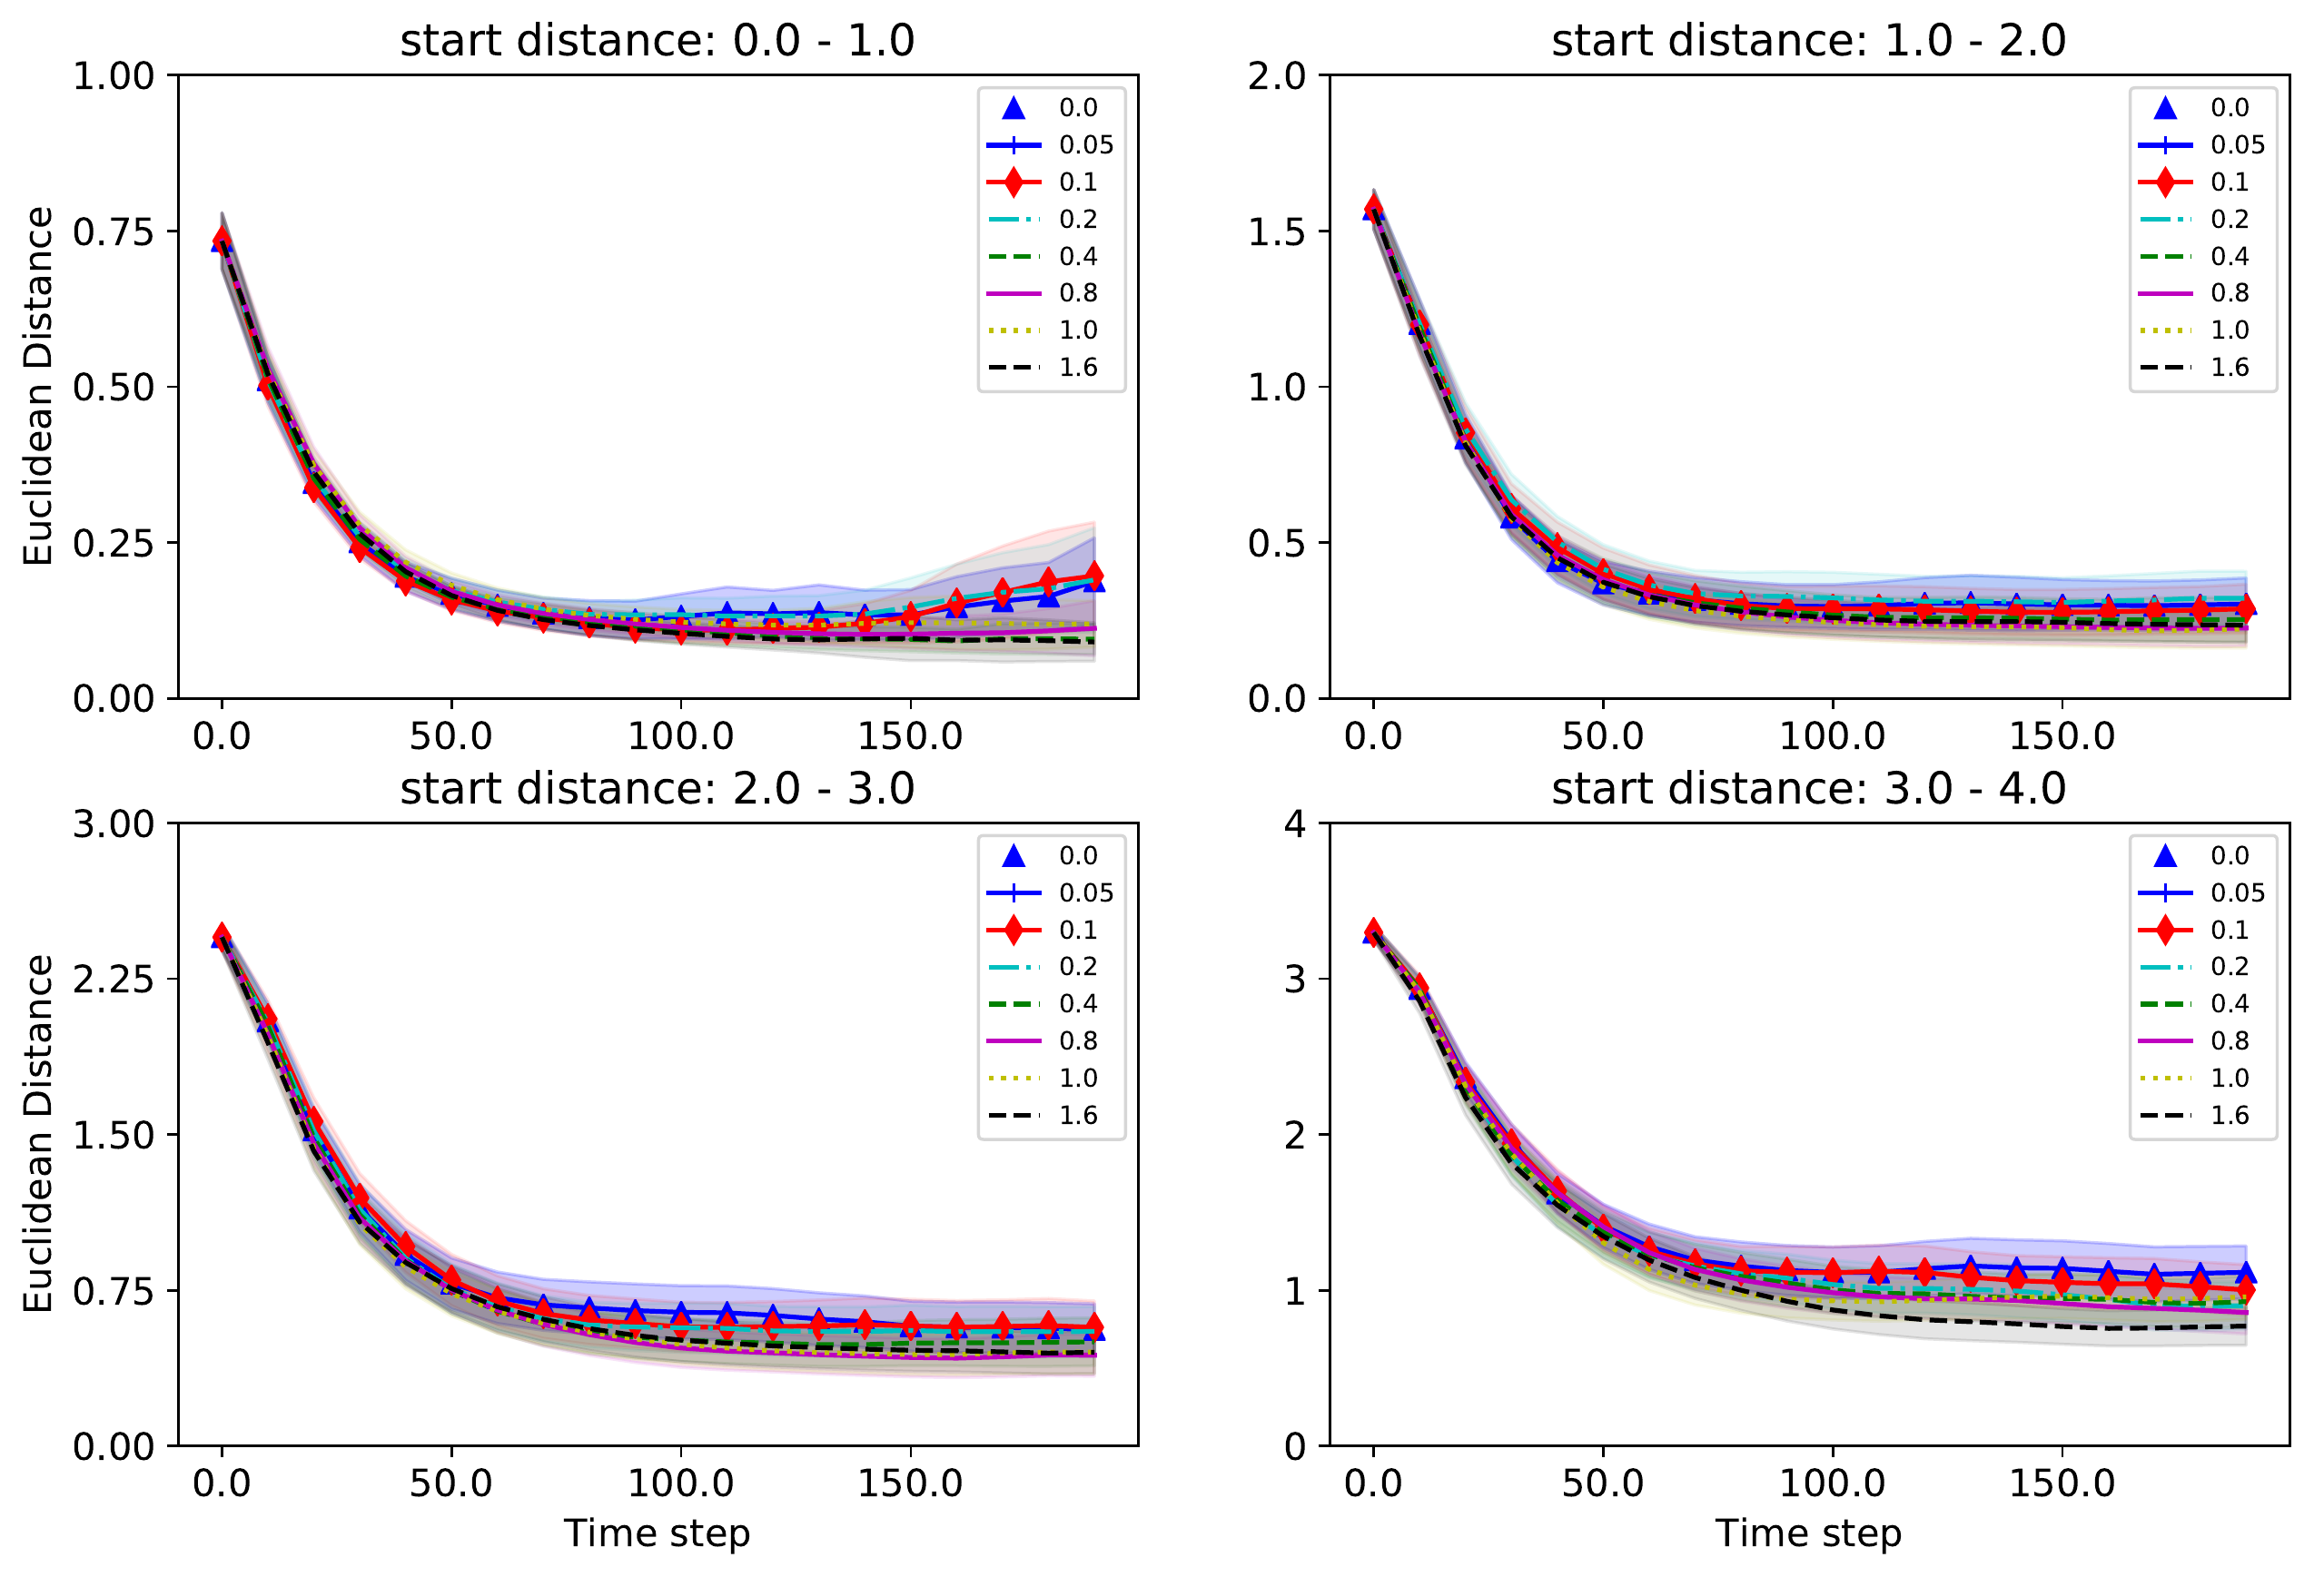}  
  \caption{Multi-point alignment}
  \label{fig:betatuningeuclideandistMultipoint}
\end{subfigure}

\caption{Euclidean distance (meters) to target with varying the weighting term in the Multitask Neural Jacobian. Plotted are the average performances across trajectories separate by initial starting distances. The filled area is the standard error of the mean. For the multi-point case distance is the sum of each point's distance to their respective targets.}
\label{fig:betatuningeuclideandist}
\end{figure}

\begin{table}[]
\centering
\setlength{\tabcolsep}{3 pt}

{\small
\begin{tabular}{c|c|c|c|c|c|c|c|c|c|c|c|}
\cline{2-12}
\multicolumn{1}{l|}{\textbf{}}         & \multicolumn{11}{c|}{\textbf{Initial Euclidean Distance (meters)}}                                                                                                                                                      \\ \cline{2-12} 
\multicolumn{1}{l|}{}                  & \multicolumn{5}{c|}{\textbf{Single Point}}                                                           &           & \multicolumn{5}{c|}{\textbf{Multiple Points}}                                                        \\ \hline
\multicolumn{1}{|c|}{\textbf{$\beta$}} & \textbf{0.0 - 0.5} & \textbf{0.5 - 1.0} & \textbf{1.0 - 1.5} & \textbf{1.5 - 2.0} & \textbf{Overall} &           & \textbf{0.0 - 1.0} & \textbf{1.0 - 2.0} & \textbf{2.0 - 3.0} & \textbf{3.0 - 4.0} & \textbf{Overall} \\ \hline
\multicolumn{1}{|c|}{\textbf{0.0}}     & \textbf{98.96}     & 85.53              & \textbf{74.75}     & 41.84              & \textbf{77.40}   & \textbf{} & 58.56              & 40.19              & 22.63              & 9.09               & 30.23            \\ \hline
\multicolumn{1}{|c|}{\textbf{0.05}}    & 98.94              & 83.26              & 74.64              & 37.60              & 76.02            & \textbf{} & 58.56              & 40.19              & 22.63              & 9.09               & 30.23            \\ \hline
\multicolumn{1}{|c|}{\textbf{0.1}}     & 98.92              & \textbf{86.03}     & 69.66              & \textbf{45.18}     & 75.86            & \textbf{} & 61.21              & 40.58              & 24.20              & 10.19              & 31.41            \\ \hline
\multicolumn{1}{|c|}{\textbf{0.2}}     & 98.97              & 84.97              & 69.86              & 42.94              & 75.30            & \textbf{} & 57.47              & 35.84              & 22.81              & \textbf{10.74}     & 28.88            \\ \hline
\multicolumn{1}{|c|}{\textbf{0.4}}     & 98.00              & 85.58              & 73.23              & 42.48              & 76.77            & \textbf{} & 66.53              & 43.54              & 25.70              & 10.73              & \textbf{33.64}   \\ \hline
\multicolumn{1}{|c|}{\textbf{0.8}}     & 98.82              & 84.78              & 71.07              & 43.08              & 75.72            & \textbf{} & 63.96              & 42.56              & \textbf{26.42}     & 7.40               & 32.92            \\ \hline
\multicolumn{1}{|c|}{\textbf{1.0}}     & 98.82              & 83.38              & 70.53              & 39.07              & 74.52            & \textbf{} & 63.10              & \textbf{44.91}     & 25.78              & 5.58               & 33.17            \\ \hline
\multicolumn{1}{|c|}{\textbf{1.6}}     & 98.44              & 84.70              & 65.85              & 35.82              & 72.67            & \textbf{} & \textbf{69.80}     & 39.61              & 25.29              & 9.04               & 32.12            \\ \hline
\end{tabular}
}
\caption{Percentage of successfully reaching targets for different values of $\beta$ in Multitask Neural Jacobian method. We use the average success percentages for thresholds from 0.0m - 0.1m from target for single-point  and the AUC for 0.0m - 0.25m for multi-point. In bold are the best performance for each distance. In multi-point setting the distance is the sum of distances for all points to their respective targets.}
\label{tab:tuningbetasuccesses}
\end{table}
\subsection{Jacobian Conditioning of Environments}

\begin{table}[]
\begin{tabular}{c|c|c|c|c|}
\cline{2-5}
                                                         & \multicolumn{2}{c|}{Single Point} & \multicolumn{2}{c|}{Multiple Points} \\ \cline{2-5} 
                                                         & mean       & standard deviation   & mean           & standard deviation  \\ \hline
\multicolumn{1}{|c|}{\textbf{Broyden}}                   & 11.658     & 25.373               & 6.070931e+14   & 5.305740e+15        \\ \hline
\multicolumn{1}{|c|}{\textbf{Finite Difference}}         & 15.933     & 0.000                & 3.785613e+16   & 1.600000e+01        \\ \hline
\multicolumn{1}{|c|}{\textbf{KNN Local Linear}}          & 141.677    & 40410.916            & 1.846220e+02   & 3.844440e+02        \\ \hline
\multicolumn{1}{|c|}{\textbf{Multitask Neural Jacobian}} & 3.290      & 1.795                & 1.085200e+01   & 3.987000e+00        \\ \hline
\multicolumn{1}{|c|}{\textbf{Neural Jacobian}}           & 5.101      & 4.067                & 1.520790e+02   & 1.313760e+02        \\ \hline
\multicolumn{1}{|c|}{\textbf{Neural Kinematics}}         & 5.428      & 4.463                & 2.007880e+02   & 1.743080e+02        \\ \hline
\multicolumn{1}{|c|}{\textbf{True Jacobian}}             & 5.025      & 4.456                & 1.877426e+08   & 1.278614e+08        \\ \hline
\end{tabular}
\caption{The average Jacobian condition number for each environment by algorithm. We found that between methods that there was not a significant difference, but between environment the conditioning was much more notable.}
\label{tab:jacobiancond}
\end{table}

In this experiment we looked at the matrix condition number for the Jacobians at each step of control for all algorithms and for each step of control. The condition number gives us an idea of how close to singularities, or linear dependence our matrices are \cite{heath1996scientificcomputing}. Closer to 1 suggest better conditioned matrices that are robust to noise. For this analysis we averaged across all Jacobian calculations in our experiments. These included each step of a trajectory across all collected trajectories. We note this does not give a complete picture of conditioning between algorithms, and is primarily to illustate the challenges between the single point and multi point experiments.  The results are included in Table~\ref{tab:jacobiancond}. Between algorithms we observed some noticeable differences between average Jacobian conditioning for different approximations in the single point case. Across environments, the much large magnitudes of condition numbers in the multi-point environment demonstrates the difficulty of this task, where all algorithms are much more poorly conditioned for the task, including the true Jacobian. 
\subsection{Sensitivity of Number of Neighbours}

In this section we provide results from tuning the number of neighbours in our KNN Neural Jacobian method. We only conducted the experiment on the multi-point environment using the same trajectories in our control experiments. The hyperparameters are almost entirely the same as our other multi-point experiments. One exception is that we use 50 epochs to train over as opposed to the 40 in the original experiment. We increased the number of epochs to allow sufficient time for the model to converge, even if the best performance on the validation set occurred much earlier. We tried values 2, 4, 8, 16, 32, 64 for the neighborhood. We did not try a higher number of neighbors as our current results suggest the number of neighbors is not that sensitive, and with our implementation we stored the dataset in memory so the cost was too much. 
We also tuned over the number of neighbors in the local linear baseline. We include the percentage of successful controls to the target point and the Condition number. We also plotted the Jacobian error, but our results were generally consistent with previous work with the Local linear method. An interesting exception was our results with eight neighbors. We found that our Jacobian estimates exploded. We conjecture that this is because when the number of neighbors is small 

\begin{figure}[ht]
\begin{subfigure}{.5\textwidth}
  \centering
  % include first image
  \includegraphics[width=\linewidth]{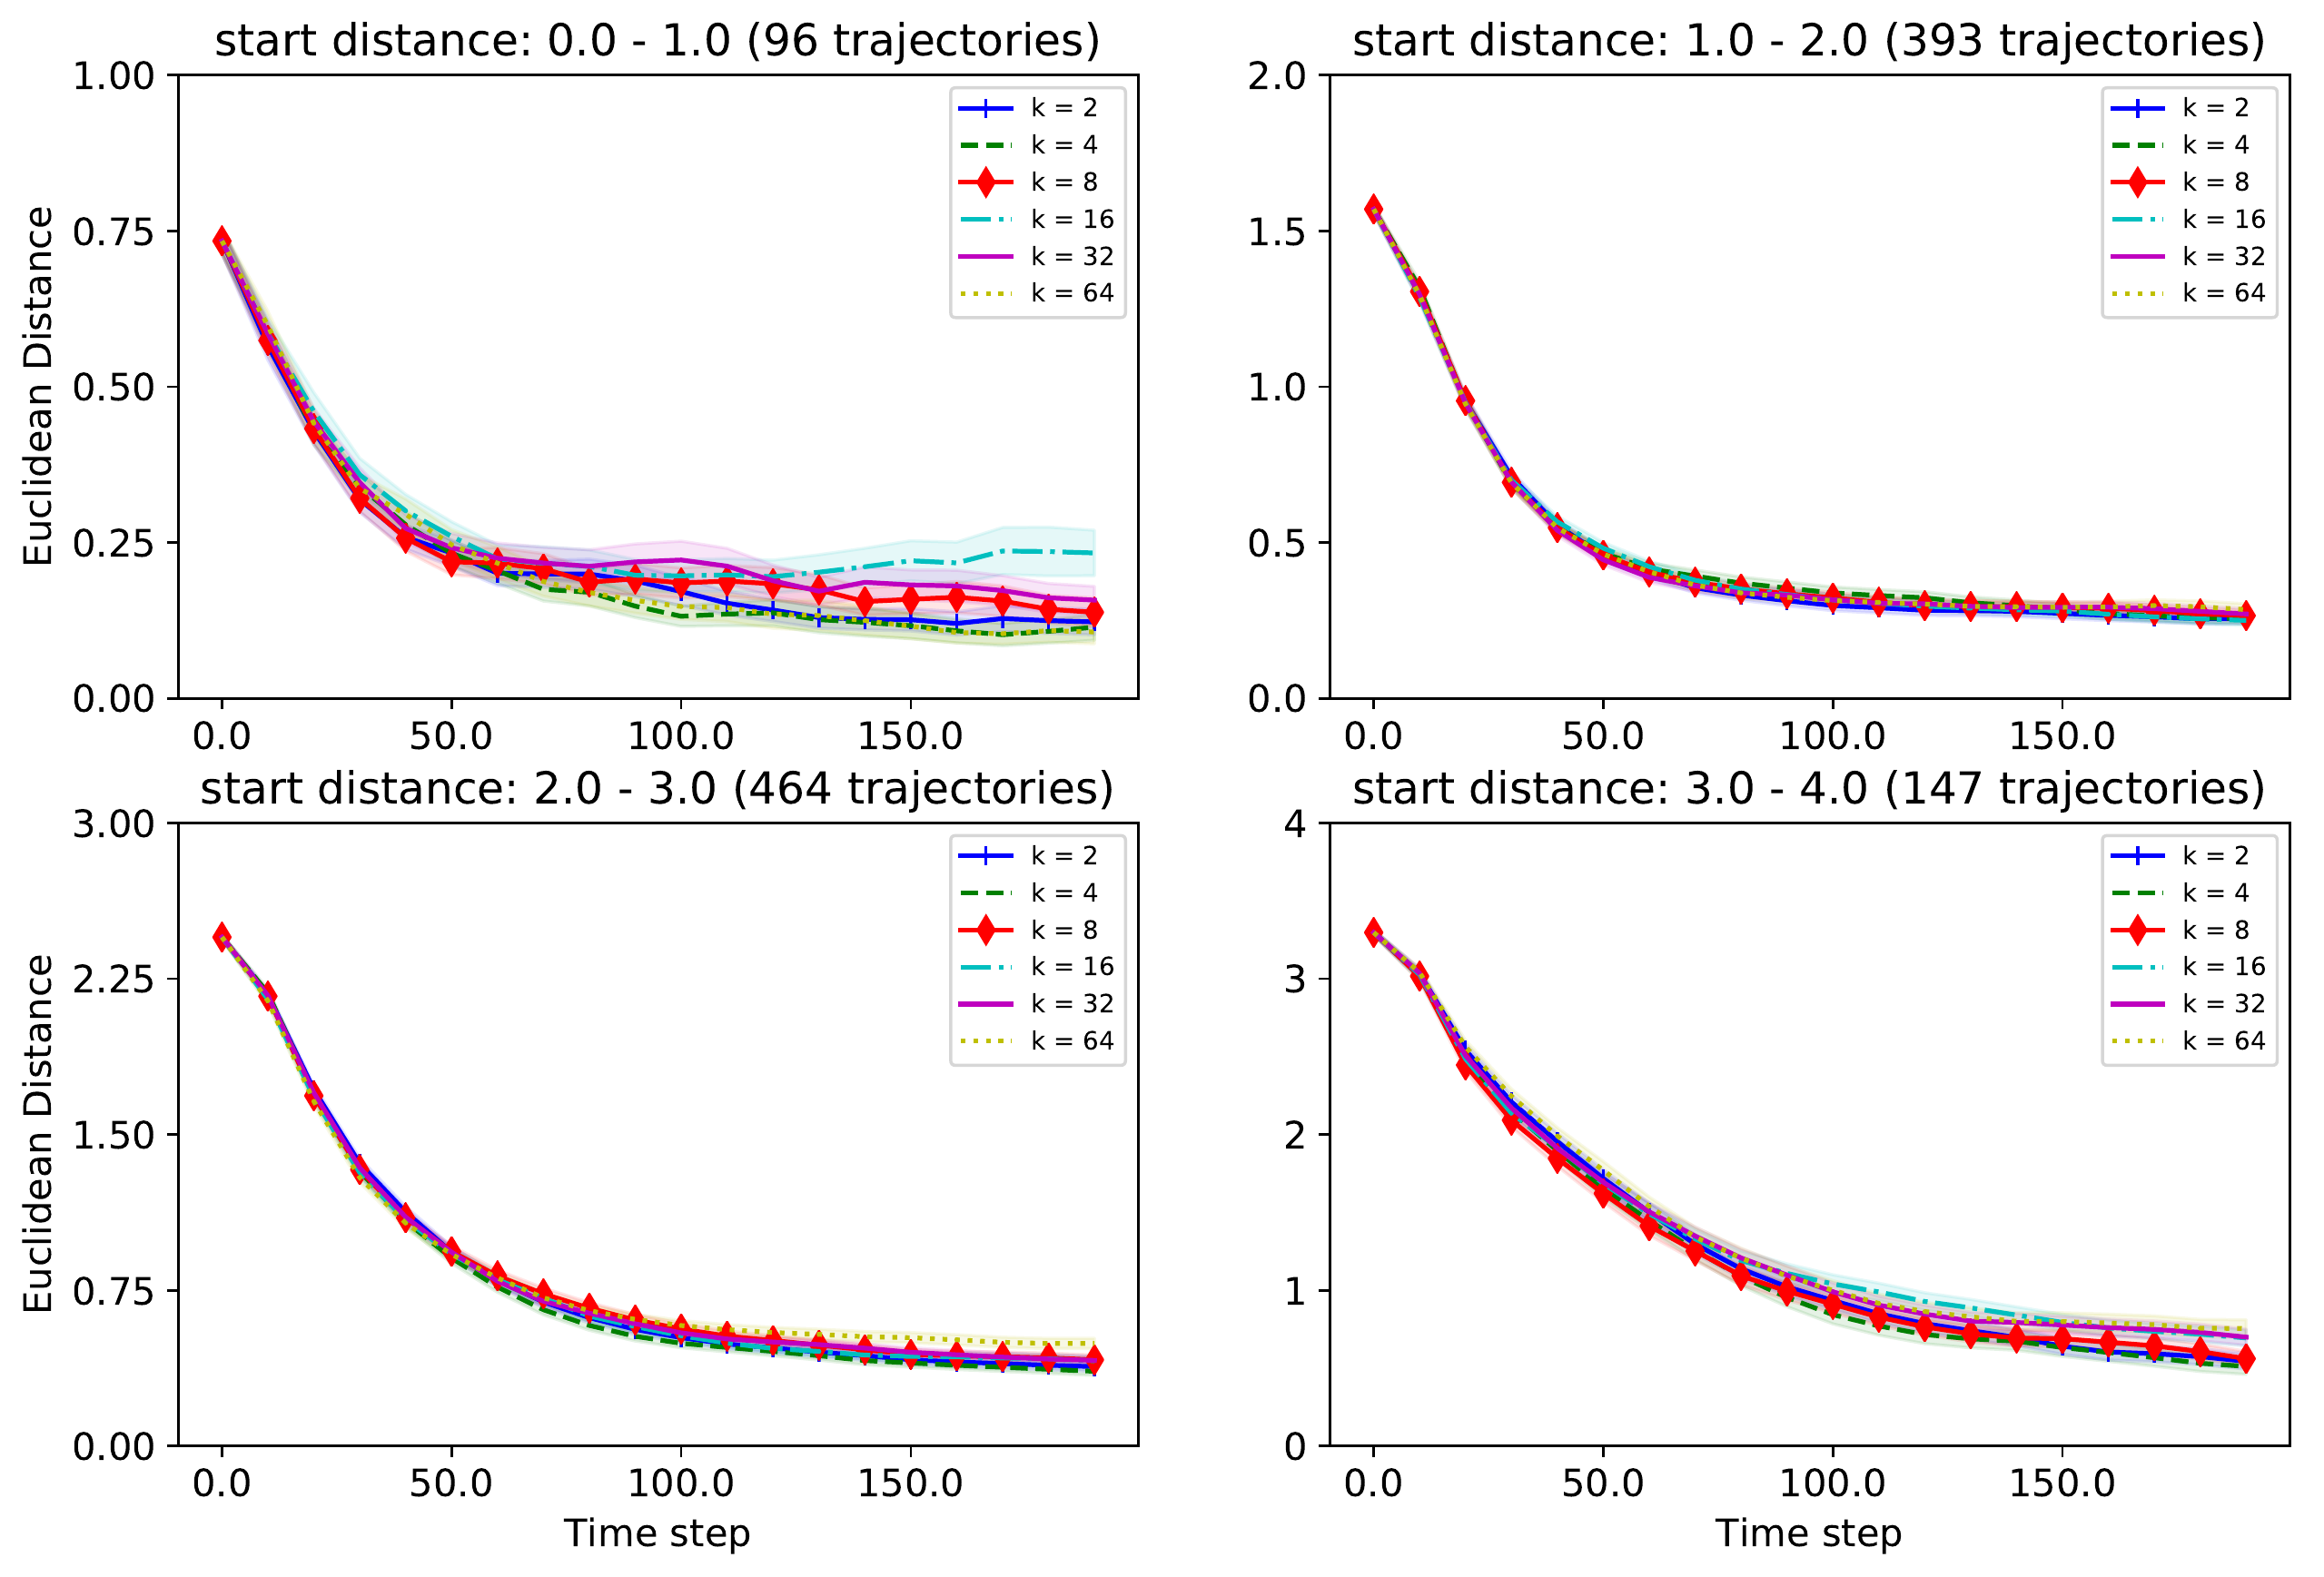}  
  \caption{Vanilla KNN Neural Jacobian}
  \label{fig:betatuningeuclideandistsinglepoint}
\end{subfigure}
\begin{subfigure}{.5\textwidth}
  \centering
  % include second image
  \includegraphics[width=\linewidth]{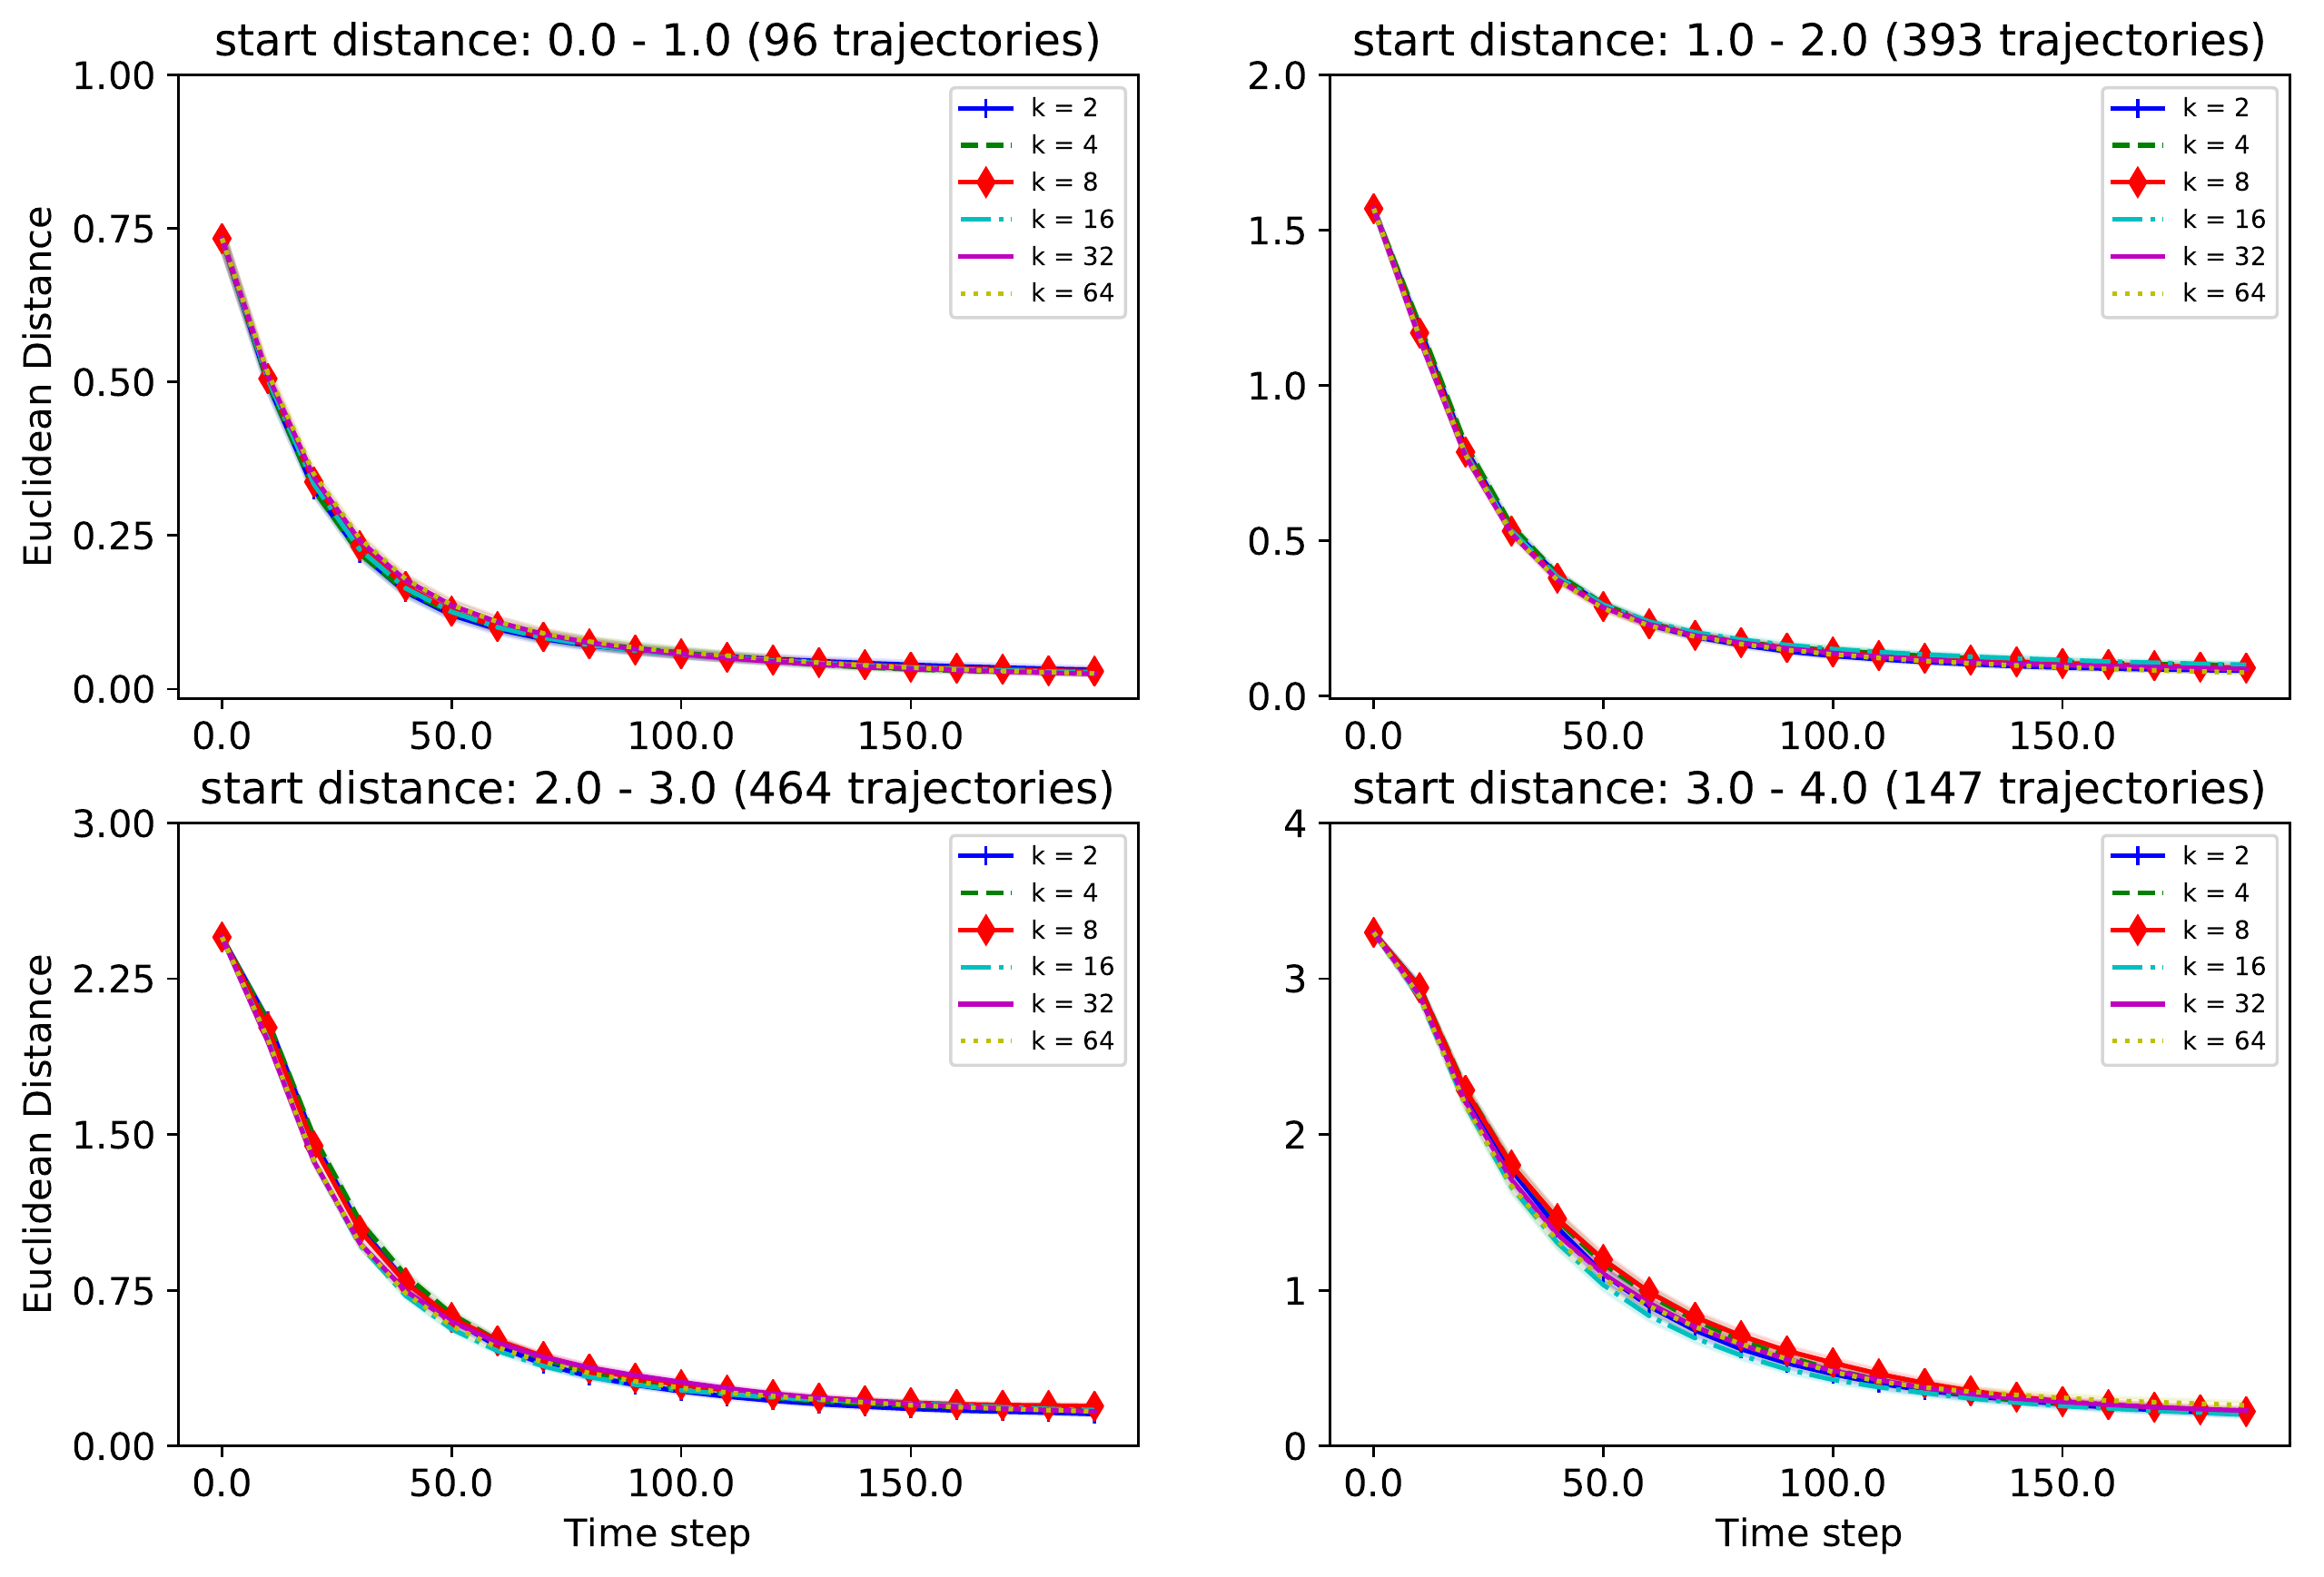}  
  \caption{Multitask KNN Neural Jacobian}
  \label{fig:betatuningeuclideandistMultipoint}
\end{subfigure}

\caption{Performance of different neighborhood sizes for the KNN Neural Jacobian method on the Multiple Point environment.}
\label{fig:knnsensitivityeuclideandist}
\end{figure}

\begin{table}[]
\centering
\setlength{\tabcolsep}{3 pt}

{\small
\begin{tabular}{|c|c|c|c|c|c|c|c|c|c|c|c|}
\hline
           & \multicolumn{5}{c|}{\textbf{KNN Neural Jacobian}}                                                         &           & \multicolumn{5}{c|}{\textbf{Multitask KNN Neural Jacobian}}                                               \\ \hline
\textbf{K} & \textbf{0.0 - 1.0 m} & \textbf{1.0 - 2.0 m} & \textbf{2.0 - 3.0 m} & \textbf{3.0 - 4.0} & \textbf{Overal} & \textbf{} & \textbf{0.0 - 1.0 m} & \textbf{1.0 - 2.0 m} & \textbf{2.0 - 3.0 m} & \textbf{3.0 - 4.0} & \textbf{Overal} \\ \hline
2          & 68.02                & 49.51                & 39.61                & 26.00              & 43.81           &           & 88.30                & 74.29                & 59.30                & 41.70              & 64.83           \\ \hline
4          & 70.94                & 49.26                & 38.87                & 25.25              & 43.56           &           & 89.93                & 70.75                & 56.10                & 38.32              & 61.91           \\ \hline
8          & 65.42                & 47.70                & 37.56                & 24.14              & 41.82           &           & 88.83                & 72.61                & 55.33                & 40.81              & 62.49           \\ \hline
16         & 57.03                & 50.19                & 34.64                & 15.75              & 39.63           &           & 89.55                & 72.09                & 57.20                & 46.54              & 63.92           \\ \hline
32         & 59.88                & 50.21                & 34.42                & 20.46              & 40.42           &           & 90.51                & 74.19                & 58.65                & 42.51              & 64.82           \\ \hline
64         & 71.27                & 48.54                & 32.60                & 18.19              & 39.75           &           & 90.32                & 77.42                & 60.52                & 41.28              & 66.59           \\ \hline
\end{tabular}
}
\label{tab:knnsensitivity}
\caption{Success percentages averaged from 0.0 - 0.25 with increments of 0.001 steps.}
\end{table}
