# Supplementary material for: Analyzing Neural Jacobian Methods in Applications of Visual Servoing and Kinematic Control
Source: arXiv:2106.06083 source file (2021-06-10)
Supplement: Supplementary file 2 [file jacobian_histogram.tex]

\begin{figure}[ht]
\begin{subfigure}{.5\textwidth}
  \centering
  % include first image
  \includegraphics[width=\linewidth]{diagrams/pt_to_pt_sim_diagrams/pt_to_pt_jacobian_hist.pdf}  
  \caption{Single Point Alignment}
  \label{fig:frobenius_single_histogram}
\end{subfigure}
\begin{subfigure}{.5\textwidth}
  \centering
  % include second image
  \includegraphics[width=\linewidth]{diagrams/multi_point_diagrams/multi_pt_jacobian_hist.pdf}  
  \caption{Multi-point alignment}
  \label{fig:frobenius_multi_histogram}
\end{subfigure}
\caption{Frobenius distance of approximated Jacobians compared to the true Kinematics Jacobian over trajectories. Plots are of mean performance with standard-error of the mean.}
\label{fig:frobenius_histograms}
\end{figure}

Technically, the Frobenius distance between the true Jacobian and approximated Jacobians are not dependent on time of the trajectory being only functions of the joint angles. To see better see the distribution of Frobenius distance between Jacobian approximations, we plot histograms to see the variance of our approximations. These are available in Figure~\ref{fig:frobenius_histograms}. The Neural Kinematics model seems to be quite peaked in it's predictions for varying joint angles. The Neural Jacobian seems accurate as we move to the more complex environments, but in the single point environment is closer in approximation compared to the local linear models.
