# Supplementary material for: Analyzing Neural Jacobian Methods in Applications of Visual Servoing and Kinematic Control
Source: arXiv:2106.06083 source file (2021-06-10)
Supplement: Supplementary file 3 [file InvJacDets.tex]

\section{Inverse Jacobian Derivation for Reacher}

Here we include the equations that describe the inverse Jacobian controller used for the Kinova environment. With two planar rotation joints the position of the end-effector can be described by the following equations:
\begin{equation}
    x_{e} = 
    \begin{bmatrix}
        x\\[\jot]
        y\\[\jot]
    \end{bmatrix}
        =
        \begin{bmatrix}
         L_{1} cos(q_{1}) + L_{2} cos(q_{1} + q_{2})\\L_{1}sin(q_{1}) + L_{2} sin(q_{1} + q_{2})
        \end{bmatrix}
\end{equation}.

Using the equation in the main paper by taking the derivative with respect to time we end up with the following controller: 
\begin{equation}
 \frac{\partial x_{e}}{\partial t} =
        \begin{pmatrix}
         -L_{1}sin(q_{1}) - L_{2} sin(q_{1} + q_{2}) &
         - L_{2} sin(q_{1} + q_{2})
         
         \\
         L_{1} cos(q_{1}) + L_{2} cos(q_{1} + q_{2}) &
         L_{2} cos(q_{1} + q_{2})
        \end{pmatrix}
        \begin{pmatrix}
            \dot{q_{1}} \\  \dot{q_{2}}
        \end{pmatrix}.
\end{equation}
We exclude writing $J^{-1}$, but note that it can be found analytically using the fact $J$ is a 2-by-2 matrix.

\begin{equation}
    \min_{q} ||x^{*} - f(q)||^{2}_{2}
\end{equation}
