# Supplementary material for: Analyzing Neural Jacobian Methods in Applications of Visual Servoing and Kinematic Control
Source: arXiv:2106.06083 source file (2021-06-10)
Supplement: Supplementary file 4 [file jacobian_conditioning_of_environment.tex]

\subsection{Jacobian Conditioning of Environments}

\begin{table}[]
\begin{tabular}{c|c|c|c|c|}
\cline{2-5}
                                                         & \multicolumn{2}{c|}{Single Point} & \multicolumn{2}{c|}{Multiple Points} \\ \cline{2-5} 
                                                         & mean       & standard deviation   & mean           & standard deviation  \\ \hline
\multicolumn{1}{|c|}{\textbf{Broyden}}                   & 11.658     & 25.373               & 6.070931e+14   & 5.305740e+15        \\ \hline
\multicolumn{1}{|c|}{\textbf{Finite Difference}}         & 15.933     & 0.000                & 3.785613e+16   & 1.600000e+01        \\ \hline
\multicolumn{1}{|c|}{\textbf{KNN Local Linear}}          & 141.677    & 40410.916            & 1.846220e+02   & 3.844440e+02        \\ \hline
\multicolumn{1}{|c|}{\textbf{Multitask Neural Jacobian}} & 3.290      & 1.795                & 1.085200e+01   & 3.987000e+00        \\ \hline
\multicolumn{1}{|c|}{\textbf{Neural Jacobian}}           & 5.101      & 4.067                & 1.520790e+02   & 1.313760e+02        \\ \hline
\multicolumn{1}{|c|}{\textbf{Neural Kinematics}}         & 5.428      & 4.463                & 2.007880e+02   & 1.743080e+02        \\ \hline
\multicolumn{1}{|c|}{\textbf{True Jacobian}}             & 5.025      & 4.456                & 1.877426e+08   & 1.278614e+08        \\ \hline
\end{tabular}
\caption{The average Jacobian condition number for each environment by algorithm. We found that between methods that there was not a significant difference, but between environment the conditioning was much more notable.}
\label{tab:jacobiancond}
\end{table}

In this experiment we looked at the matrix condition number for the Jacobians at each step of control for all algorithms and for each step of control. The condition number gives us an idea of how close to singularities, or linear dependence our matrices are \cite{heath1996scientificcomputing}. Closer to 1 suggest better conditioned matrices that are robust to noise. For this analysis we averaged across all Jacobian calculations in our experiments. These included each step of a trajectory across all collected trajectories. We note this does not give a complete picture of conditioning between algorithms, and is primarily to illustate the challenges between the single point and multi point experiments.  The results are included in Table~\ref{tab:jacobiancond}. Between algorithms we observed some noticeable differences between average Jacobian conditioning for different approximations in the single point case. Across environments, the much large magnitudes of condition numbers in the multi-point environment demonstrates the difficulty of this task, where all algorithms are much more poorly conditioned for the task, including the true Jacobian.
