# Supplementary material for: Analyzing Neural Jacobian Methods in Applications of Visual Servoing and Kinematic Control
Source: arXiv:2106.06083 source file (2021-06-10)
Supplement: Supplementary file 5 [file knn_tuning_experiment.tex]

\subsection{Sensitivity of Number of Neighbours}

In this section we provide results from tuning the number of neighbours in our KNN Neural Jacobian method. We only conducted the experiment on the multi-point environment using the same trajectories in our control experiments. The hyperparameters are almost entirely the same as our other multi-point experiments. One exception is that we use 50 epochs to train over as opposed to the 40 in the original experiment. We increased the number of epochs to allow sufficient time for the model to converge, even if the best performance on the validation set occurred much earlier. We tried values 2, 4, 8, 16, 32, 64 for the neighborhood. We did not try a higher number of neighbors as our current results suggest the number of neighbors is not that sensitive, and with our implementation we stored the dataset in memory so the cost was too much. 
We also tuned over the number of neighbors in the local linear baseline. We include the percentage of successful controls to the target point and the Condition number. We also plotted the Jacobian error, but our results were generally consistent with previous work with the Local linear method. An interesting exception was our results with eight neighbors. We found that our Jacobian estimates exploded. We conjecture that this is because when the number of neighbors is small 

\begin{figure}[ht]
\begin{subfigure}{.5\textwidth}
  \centering
  % include first image
  \includegraphics[width=\linewidth]{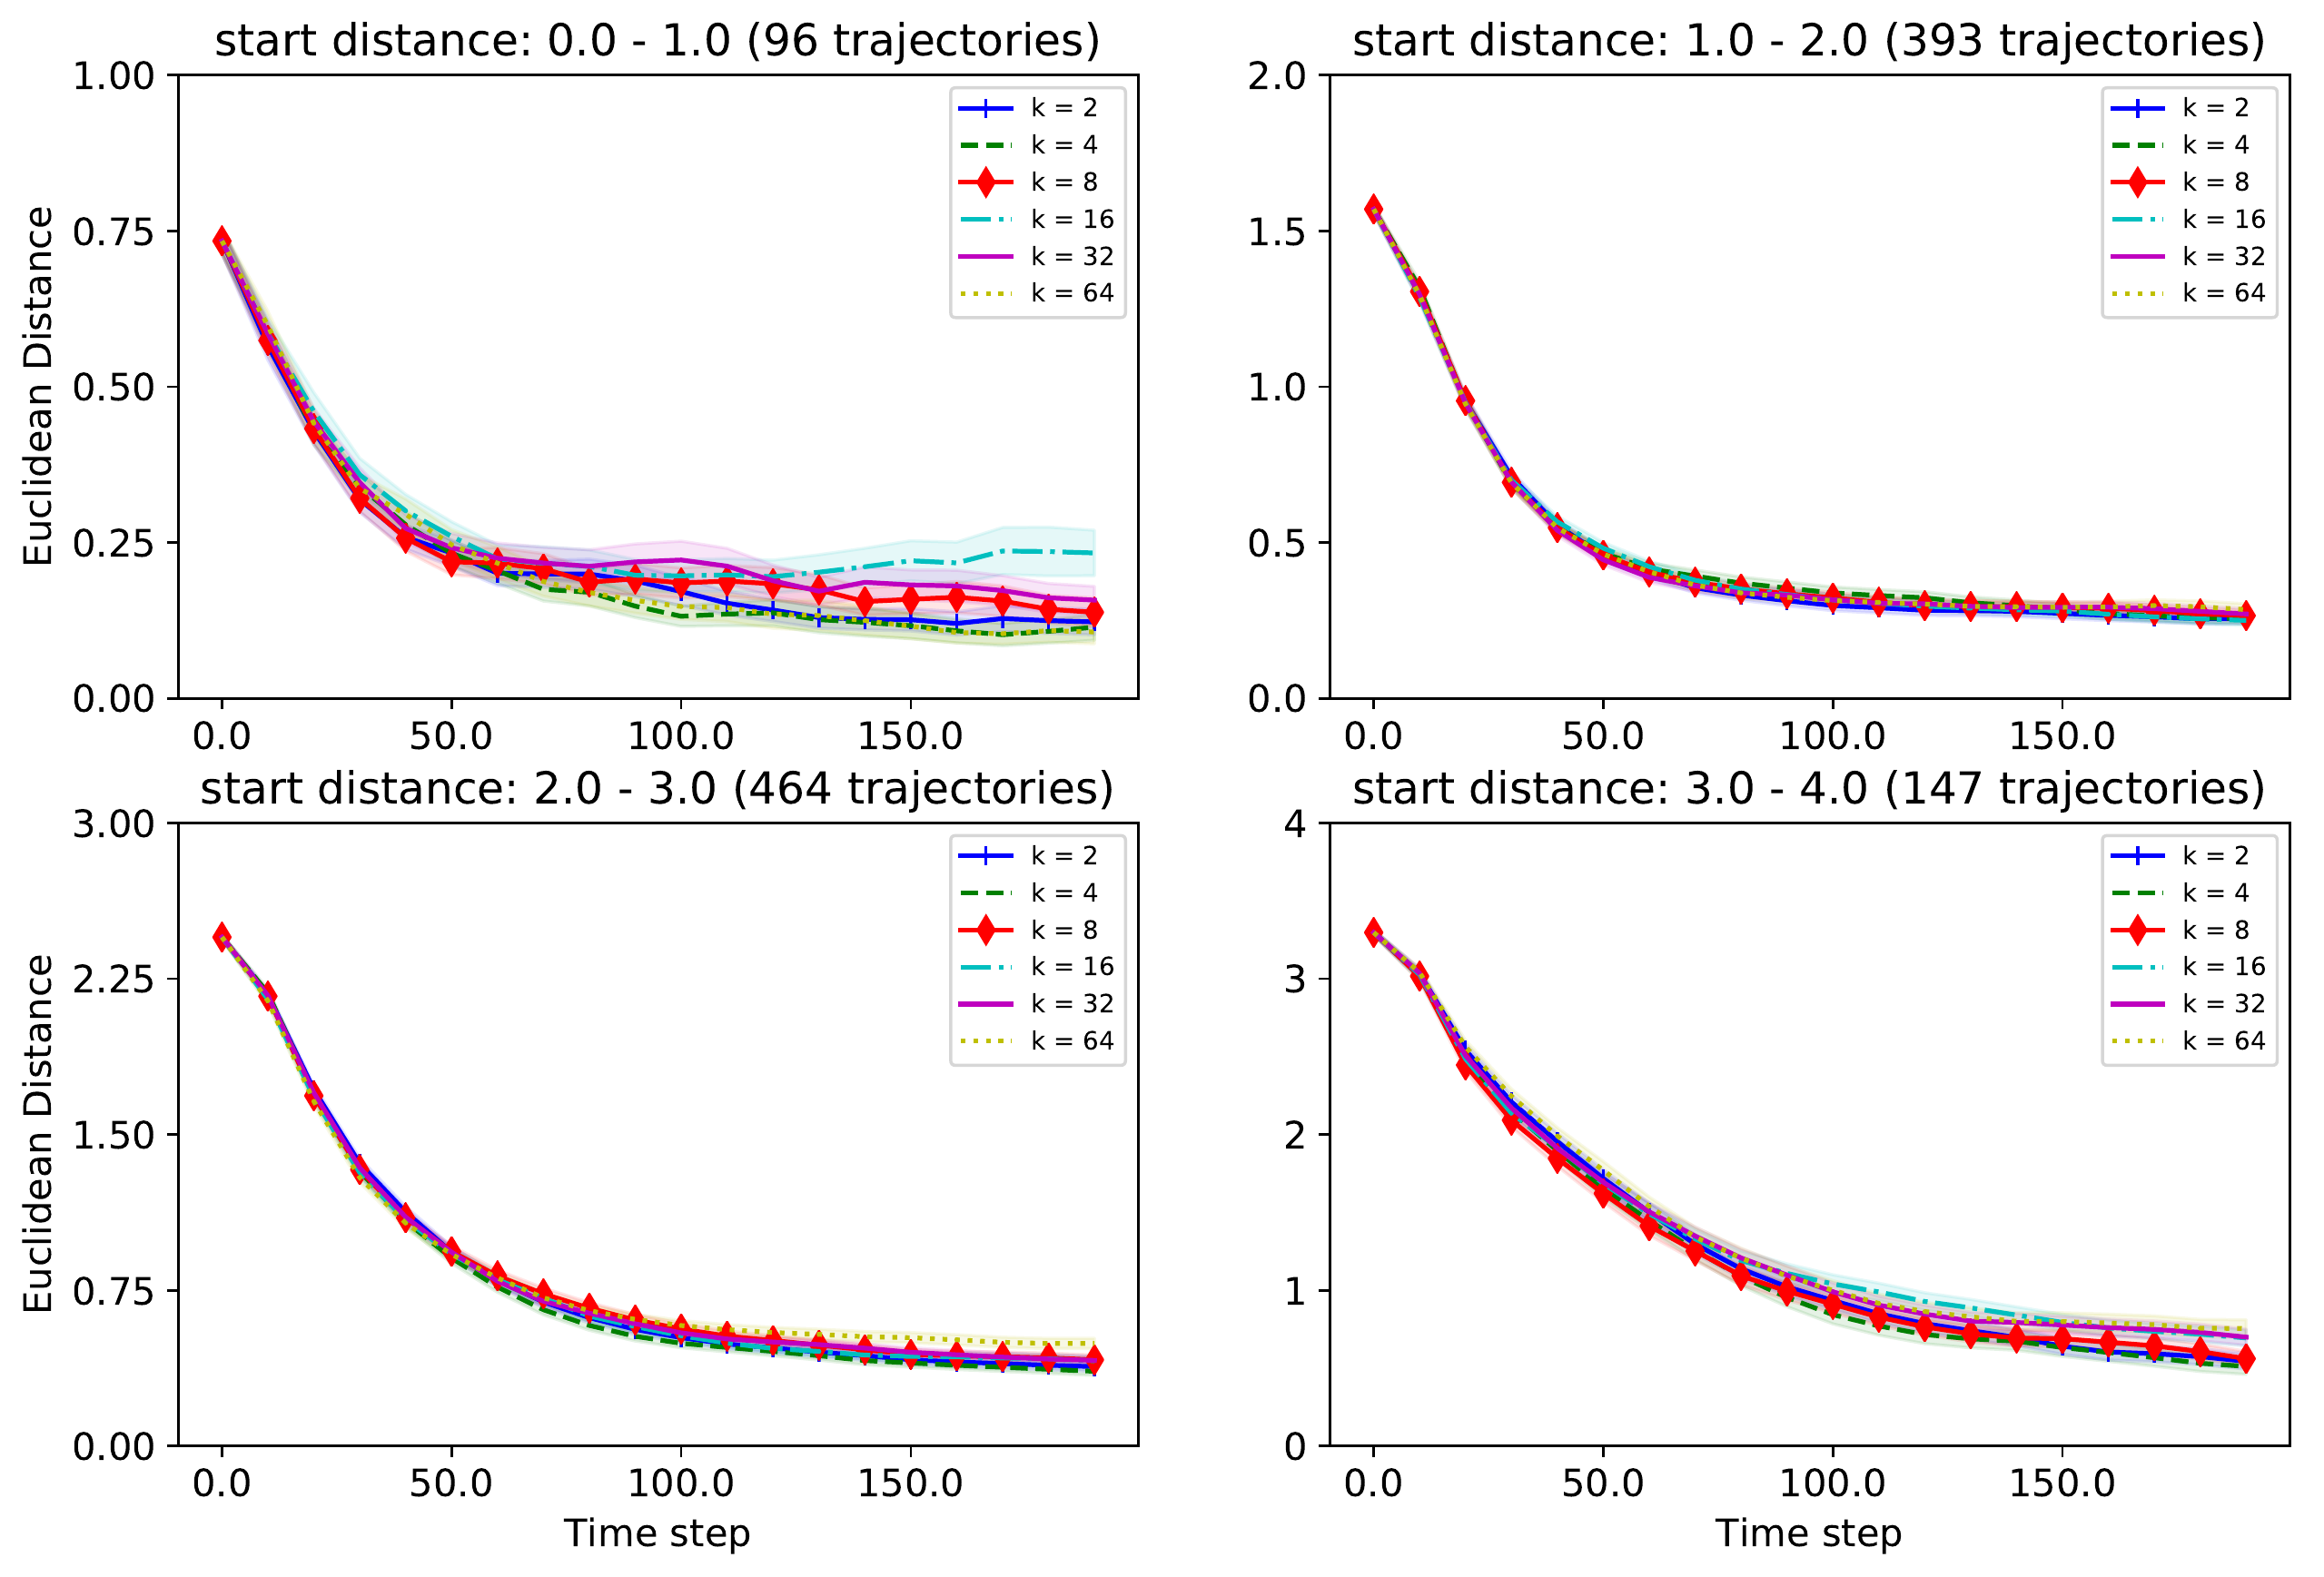}  
  \caption{Vanilla KNN Neural Jacobian}
  \label{fig:betatuningeuclideandistsinglepoint}
\end{subfigure}
\begin{subfigure}{.5\textwidth}
  \centering
  % include second image
  \includegraphics[width=\linewidth]{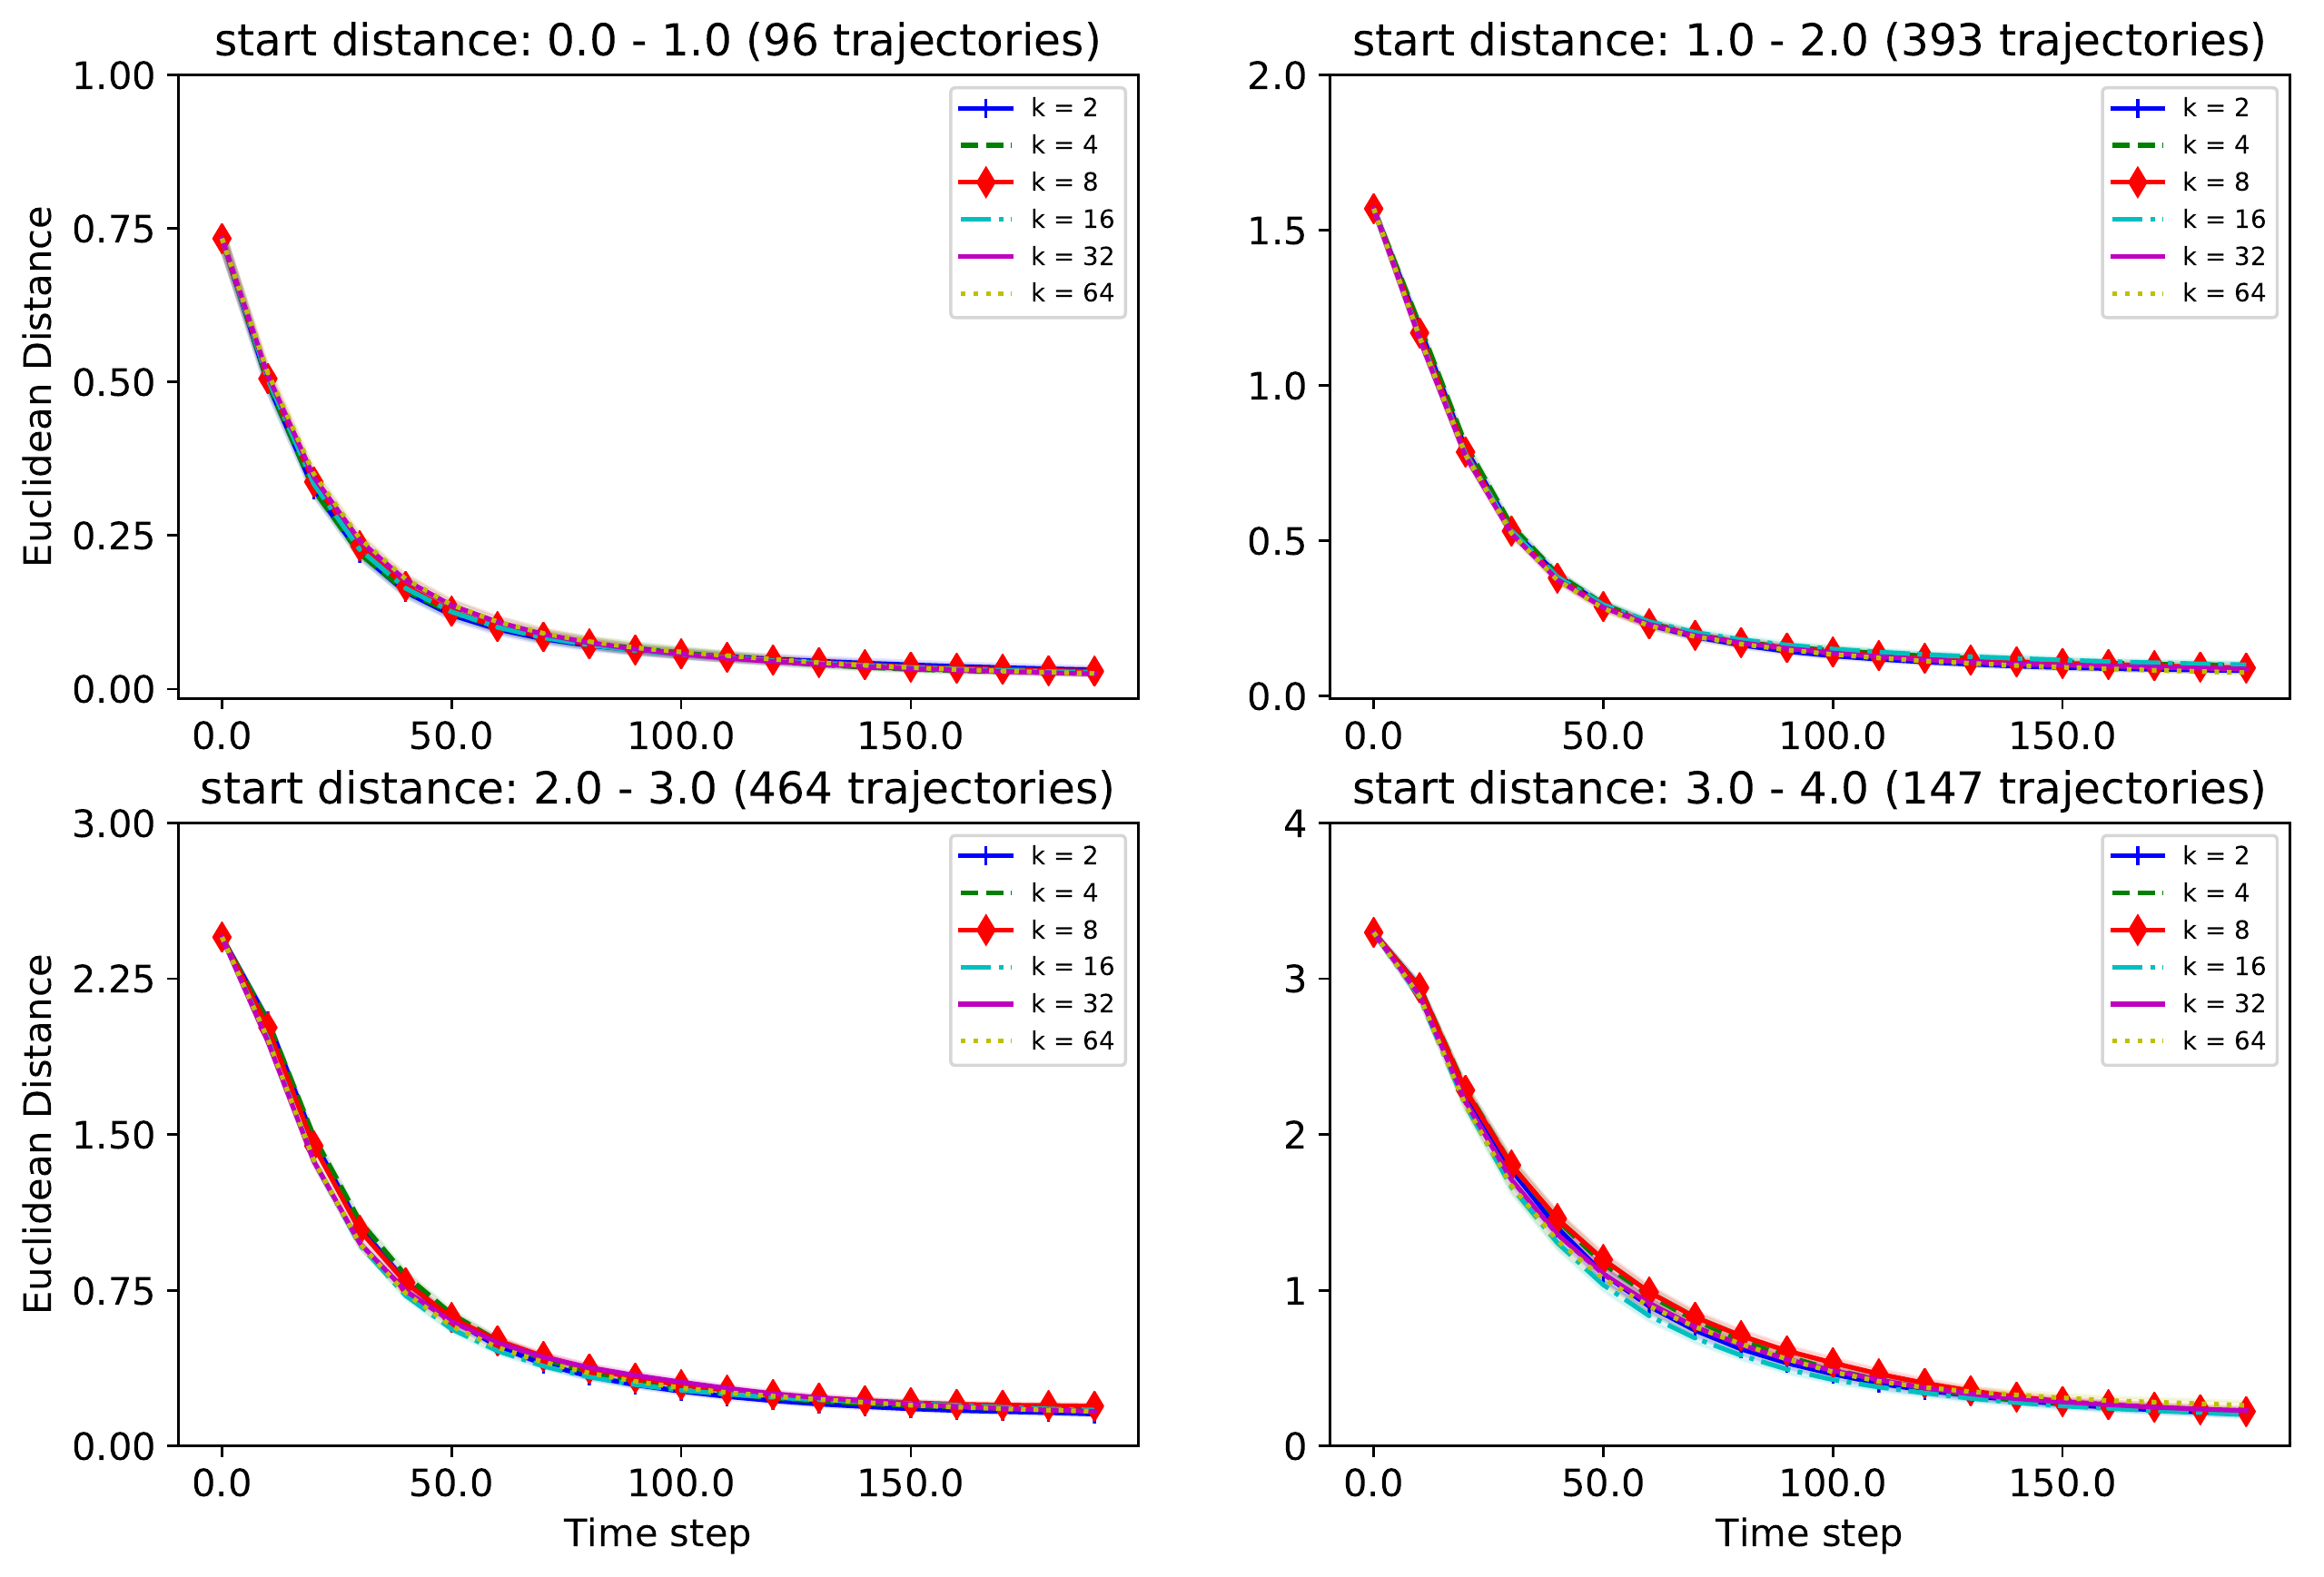}  
  \caption{Multitask KNN Neural Jacobian}
  \label{fig:betatuningeuclideandistMultipoint}
\end{subfigure}

\caption{Performance of different neighborhood sizes for the KNN Neural Jacobian method on the Multiple Point environment.}
\label{fig:knnsensitivityeuclideandist}
\end{figure}

\begin{table}[]
\centering
\setlength{\tabcolsep}{3 pt}

{\small
\begin{tabular}{|c|c|c|c|c|c|c|c|c|c|c|c|}
\hline
           & \multicolumn{5}{c|}{\textbf{KNN Neural Jacobian}}                                                         &           & \multicolumn{5}{c|}{\textbf{Multitask KNN Neural Jacobian}}                                               \\ \hline
\textbf{K} & \textbf{0.0 - 1.0 m} & \textbf{1.0 - 2.0 m} & \textbf{2.0 - 3.0 m} & \textbf{3.0 - 4.0} & \textbf{Overal} & \textbf{} & \textbf{0.0 - 1.0 m} & \textbf{1.0 - 2.0 m} & \textbf{2.0 - 3.0 m} & \textbf{3.0 - 4.0} & \textbf{Overal} \\ \hline
2          & 68.02                & 49.51                & 39.61                & 26.00              & 43.81           &           & 88.30                & 74.29                & 59.30                & 41.70              & 64.83           \\ \hline
4          & 70.94                & 49.26                & 38.87                & 25.25              & 43.56           &           & 89.93                & 70.75                & 56.10                & 38.32              & 61.91           \\ \hline
8          & 65.42                & 47.70                & 37.56                & 24.14              & 41.82           &           & 88.83                & 72.61                & 55.33                & 40.81              & 62.49           \\ \hline
16         & 57.03                & 50.19                & 34.64                & 15.75              & 39.63           &           & 89.55                & 72.09                & 57.20                & 46.54              & 63.92           \\ \hline
32         & 59.88                & 50.21                & 34.42                & 20.46              & 40.42           &           & 90.51                & 74.19                & 58.65                & 42.51              & 64.82           \\ \hline
64         & 71.27                & 48.54                & 32.60                & 18.19              & 39.75           &           & 90.32                & 77.42                & 60.52                & 41.28              & 66.59           \\ \hline
\end{tabular}
}
\label{tab:knnsensitivity}
\caption{Success percentages averaged from 0.0 - 0.25 with increments of 0.001 steps.}
\end{table}
