# Supplementary material for: Analyzing Neural Jacobian Methods in Applications of Visual Servoing and Kinematic Control
Source: arXiv:2106.06083 source file (2021-06-10)
Supplement: Supplementary file 6 [file multi_task_tuning.tex]

\section{Multitask Jacobian Parameter Comparisons}

In this section we include additional results when we investigated tuning the weighting term $\beta$ for the Multitask Neural Jacobian. Our experimental set-up was the same as described previously for the simulators. We only consider comparing the Multitask Neural Jacobian against each other. When $\beta=0.0$ this is the same as the original Neural Jacobian. 

Decreases in the Euclidean distance (meters) to the target are visualized in Figure~\ref{fig:betatuningeuclideandist}. This plot suggests that increasing $\beta$ seems to help in the multi-point environment for the closer targets but overall differences are relatively minute. We also include the percentages of successes, which was calculated the same way for our other experiments, in Table~\ref{tab:tuningbetasuccesses}. These results show similar results reported in our main paper, where the main benefits of the Multitask Neural Jacobian seem more evident in the multi-point environment. For the single point case,  even for smaller $\beta$ negatively, impact performance.

\begin{figure}[ht]
\begin{subfigure}{.5\textwidth}
  \centering
  % include first image
  \includegraphics[width=\linewidth]{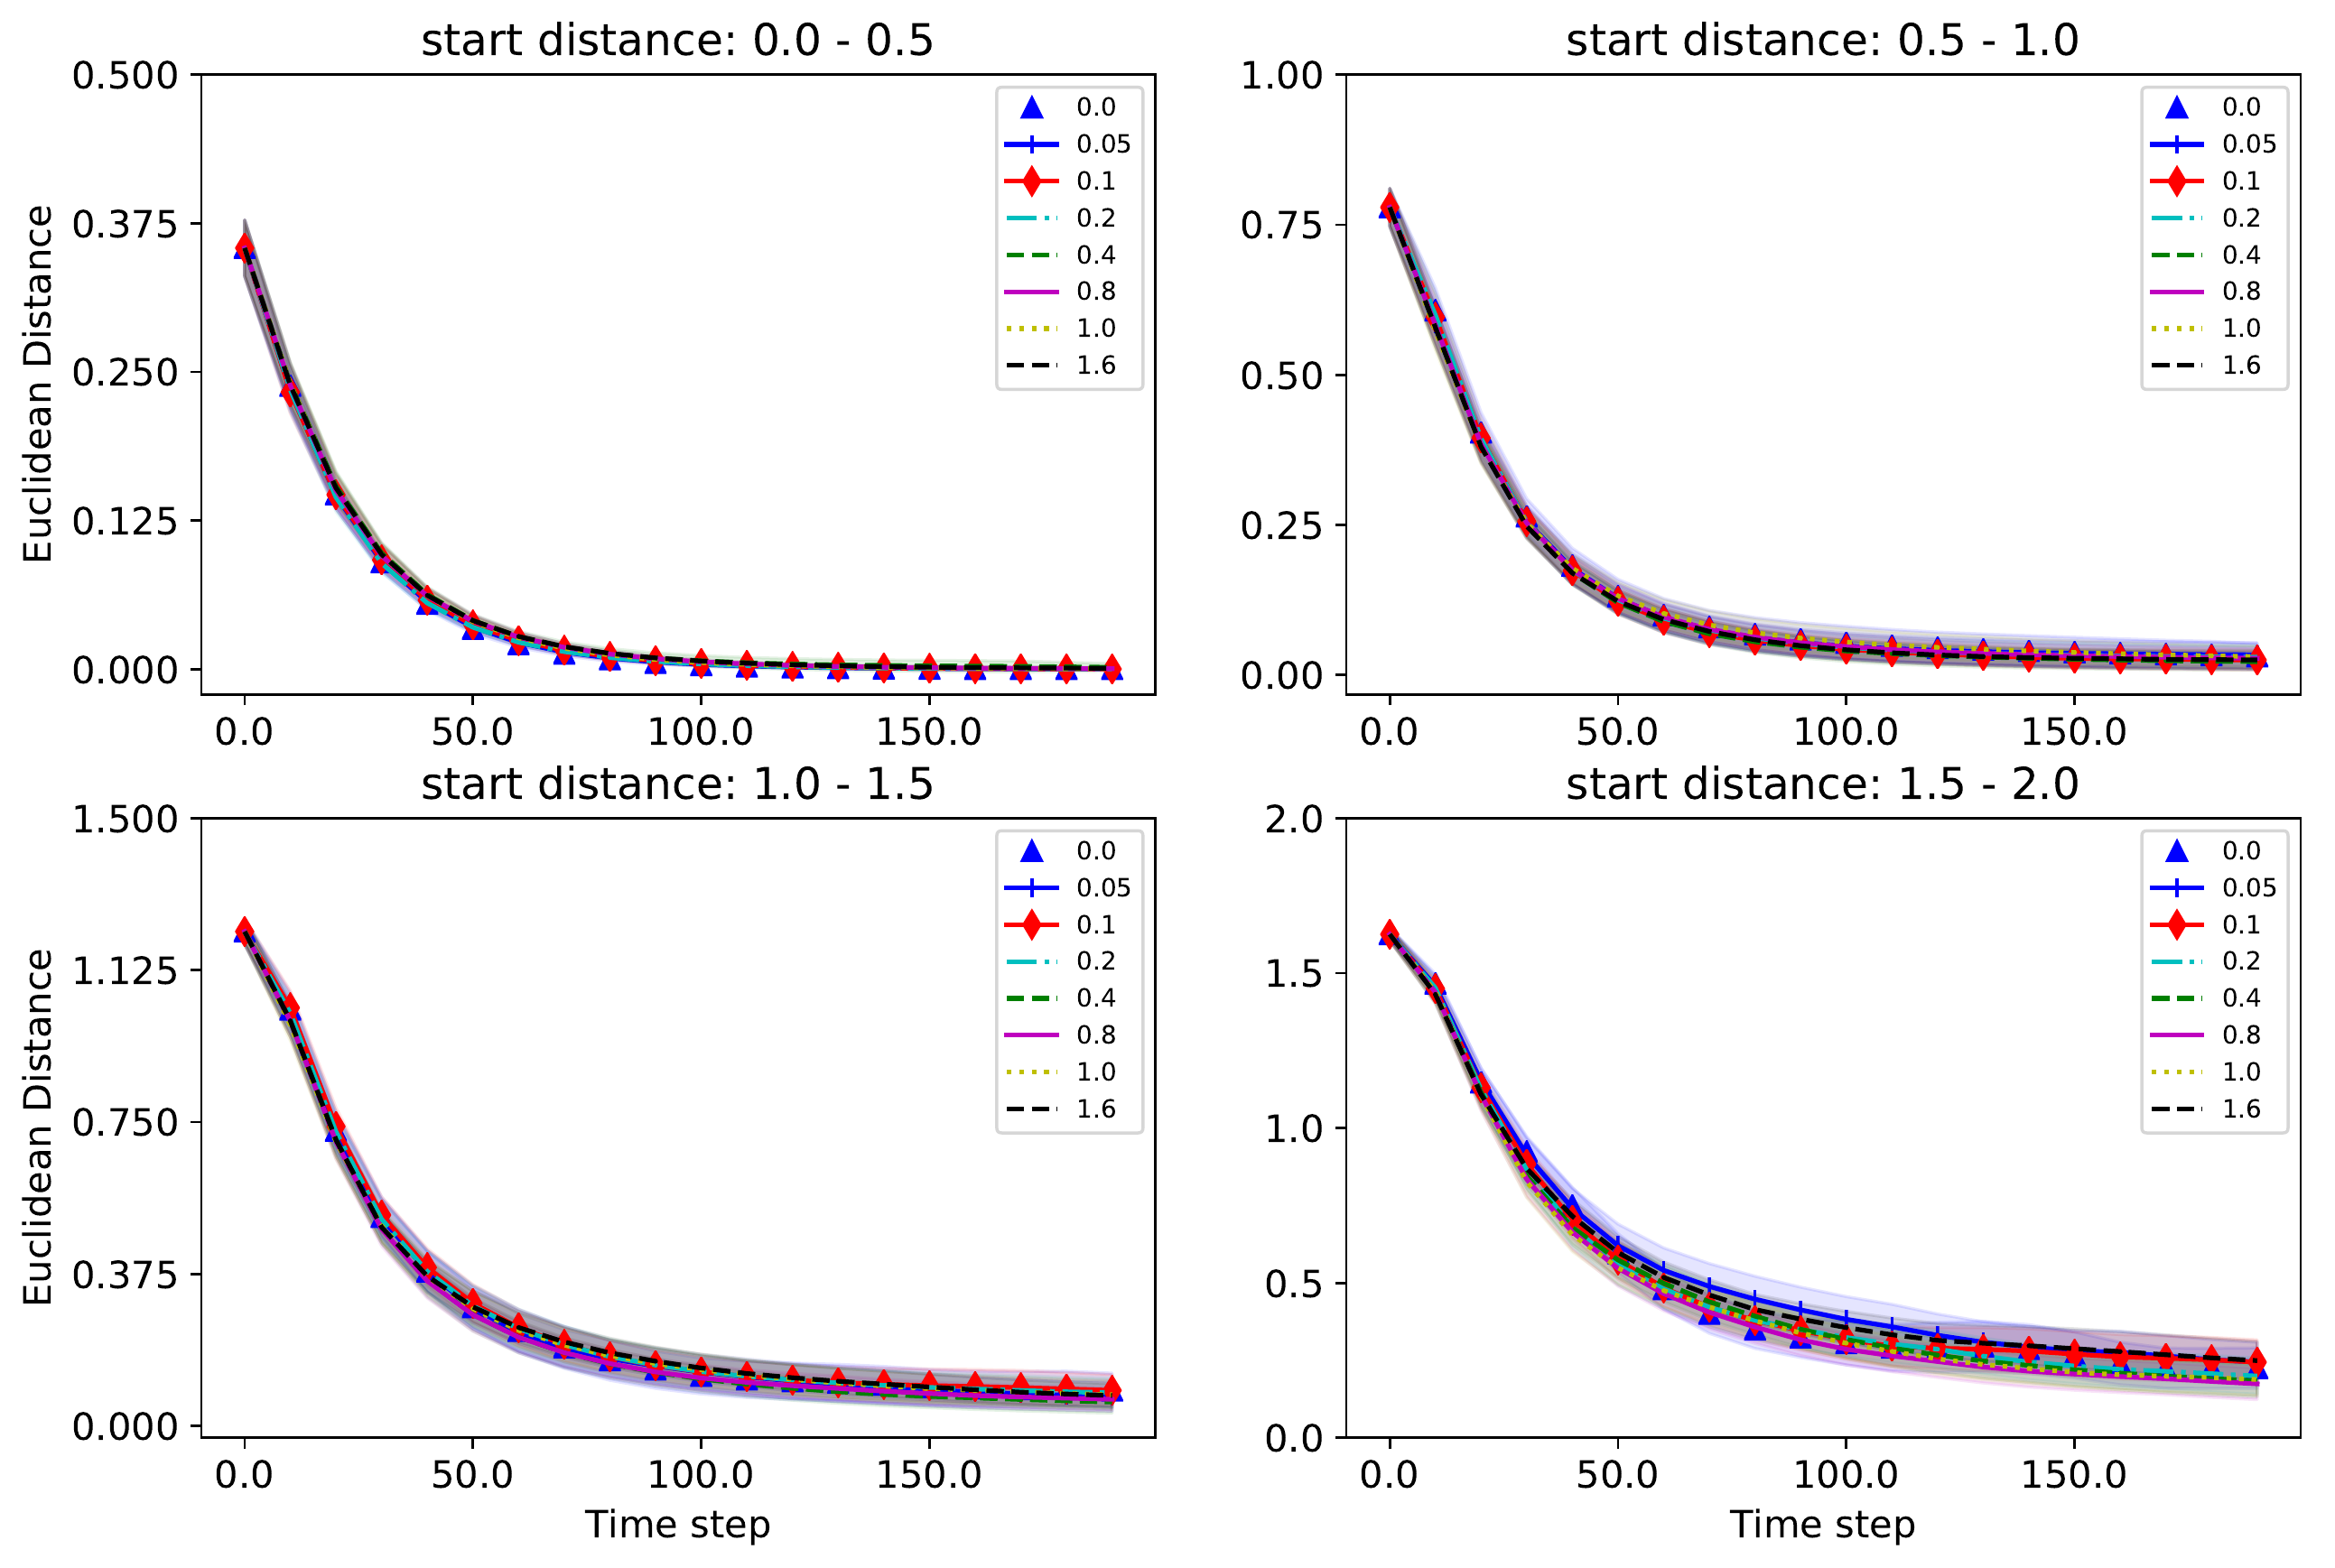}  
  \caption{Single Point Alignment}
  \label{fig:betatuningeuclideandistsinglepoint}
\end{subfigure}
\begin{subfigure}{.5\textwidth}
  \centering
  % include second image
  \includegraphics[width=\linewidth]{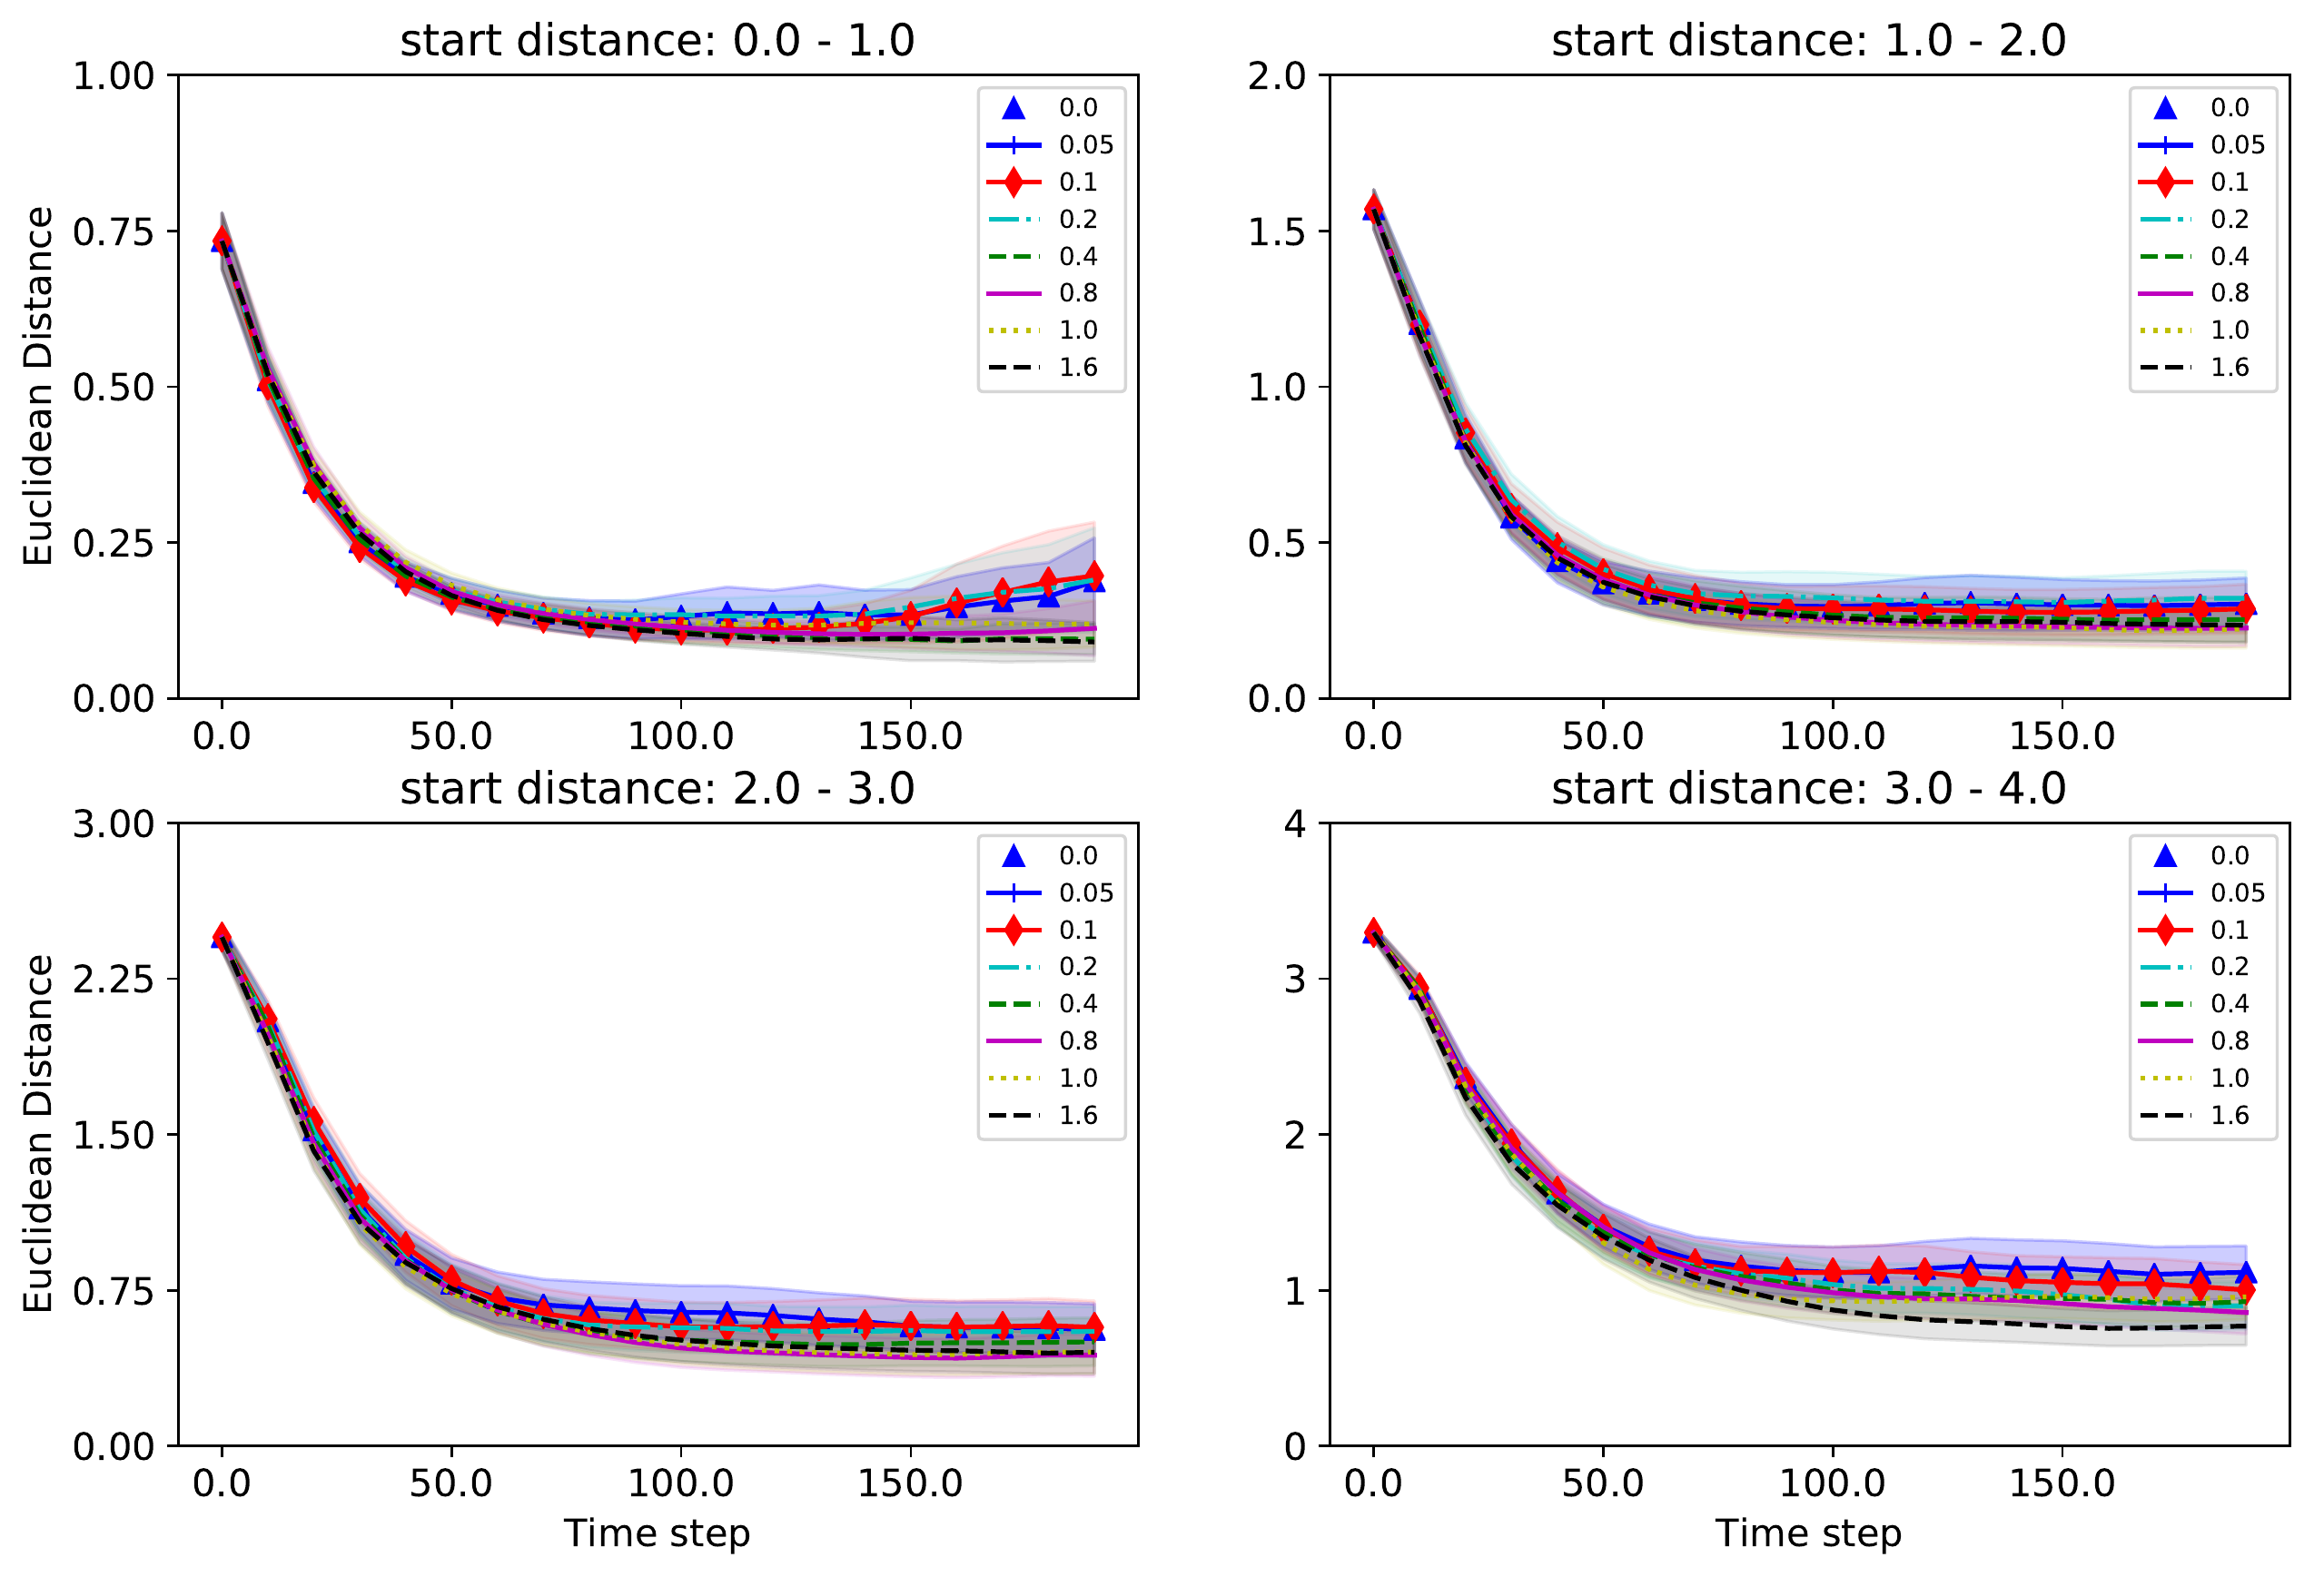}  
  \caption{Multi-point alignment}
  \label{fig:betatuningeuclideandistMultipoint}
\end{subfigure}

\caption{Euclidean distance (meters) to target with varying the weighting term in the Multitask Neural Jacobian. Plotted are the average performances across trajectories separate by initial starting distances. The filled area is the standard error of the mean. For the multi-point case distance is the sum of each point's distance to their respective targets.}
\label{fig:betatuningeuclideandist}
\end{figure}

\begin{table}[]
\centering
\setlength{\tabcolsep}{3 pt}

{\small
\begin{tabular}{c|c|c|c|c|c|c|c|c|c|c|c|}
\cline{2-12}
\multicolumn{1}{l|}{\textbf{}}         & \multicolumn{11}{c|}{\textbf{Initial Euclidean Distance (meters)}}                                                                                                                                                      \\ \cline{2-12} 
\multicolumn{1}{l|}{}                  & \multicolumn{5}{c|}{\textbf{Single Point}}                                                           &           & \multicolumn{5}{c|}{\textbf{Multiple Points}}                                                        \\ \hline
\multicolumn{1}{|c|}{\textbf{$\beta$}} & \textbf{0.0 - 0.5} & \textbf{0.5 - 1.0} & \textbf{1.0 - 1.5} & \textbf{1.5 - 2.0} & \textbf{Overall} &           & \textbf{0.0 - 1.0} & \textbf{1.0 - 2.0} & \textbf{2.0 - 3.0} & \textbf{3.0 - 4.0} & \textbf{Overall} \\ \hline
\multicolumn{1}{|c|}{\textbf{0.0}}     & \textbf{98.96}     & 85.53              & \textbf{74.75}     & 41.84              & \textbf{77.40}   & \textbf{} & 58.56              & 40.19              & 22.63              & 9.09               & 30.23            \\ \hline
\multicolumn{1}{|c|}{\textbf{0.05}}    & 98.94              & 83.26              & 74.64              & 37.60              & 76.02            & \textbf{} & 58.56              & 40.19              & 22.63              & 9.09               & 30.23            \\ \hline
\multicolumn{1}{|c|}{\textbf{0.1}}     & 98.92              & \textbf{86.03}     & 69.66              & \textbf{45.18}     & 75.86            & \textbf{} & 61.21              & 40.58              & 24.20              & 10.19              & 31.41            \\ \hline
\multicolumn{1}{|c|}{\textbf{0.2}}     & 98.97              & 84.97              & 69.86              & 42.94              & 75.30            & \textbf{} & 57.47              & 35.84              & 22.81              & \textbf{10.74}     & 28.88            \\ \hline
\multicolumn{1}{|c|}{\textbf{0.4}}     & 98.00              & 85.58              & 73.23              & 42.48              & 76.77            & \textbf{} & 66.53              & 43.54              & 25.70              & 10.73              & \textbf{33.64}   \\ \hline
\multicolumn{1}{|c|}{\textbf{0.8}}     & 98.82              & 84.78              & 71.07              & 43.08              & 75.72            & \textbf{} & 63.96              & 42.56              & \textbf{26.42}     & 7.40               & 32.92            \\ \hline
\multicolumn{1}{|c|}{\textbf{1.0}}     & 98.82              & 83.38              & 70.53              & 39.07              & 74.52            & \textbf{} & 63.10              & \textbf{44.91}     & 25.78              & 5.58               & 33.17            \\ \hline
\multicolumn{1}{|c|}{\textbf{1.6}}     & 98.44              & 84.70              & 65.85              & 35.82              & 72.67            & \textbf{} & \textbf{69.80}     & 39.61              & 25.29              & 9.04               & 32.12            \\ \hline
\end{tabular}
}
\caption{Percentage of successfully reaching targets for different values of $\beta$ in Multitask Neural Jacobian method. We use the average success percentages for thresholds from 0.0m - 0.1m from target for single-point  and the AUC for 0.0m - 0.25m for multi-point. In bold are the best performance for each distance. In multi-point setting the distance is the sum of distances for all points to their respective targets.}
\label{tab:tuningbetasuccesses}
\end{table}
