# Supplementary material for: Analyzing Neural Jacobian Methods in Applications of Visual Servoing and Kinematic Control
Source: arXiv:2106.06083 source file (2021-06-10)
Supplement: Supplementary file 7 [file additional_experiments.tex]

\section{Multitask Jacobian Parameter Comparisons}

In this section we include additional results when we investigated tuning the weighting term $\beta$ for the Multitask Neural Jacobian. Our experimental set-up was the same as described previously for the simulators. We only consider comparing the Multitask Neural Jacobian against each other. When $\beta=0.0$ this is the same as the original Neural Jacobian. 

Decreases in the Euclidean distance (meters) to the target are visualized in Figure~\ref{fig:betatuningeuclideandist}. This plot suggests that increasing $\beta$ seems to help in the multi-point environment for the closer targets but overall differences are relatively minute. We also include the percentages of successes, which was calculated the same way for our other experiments, in Table~\ref{tab:tuningbetasuccesses}. These results show similar results reported in our main paper, where the main benefits of the Multitask Neural Jacobian seem more evident in the multi-point environment. For the single point case,  even for smaller $\beta$ negatively, impact performance.

\begin{figure}[ht]
\begin{subfigure}{.5\textwidth}
  \centering
  % include first image
  \includegraphics[width=\linewidth]{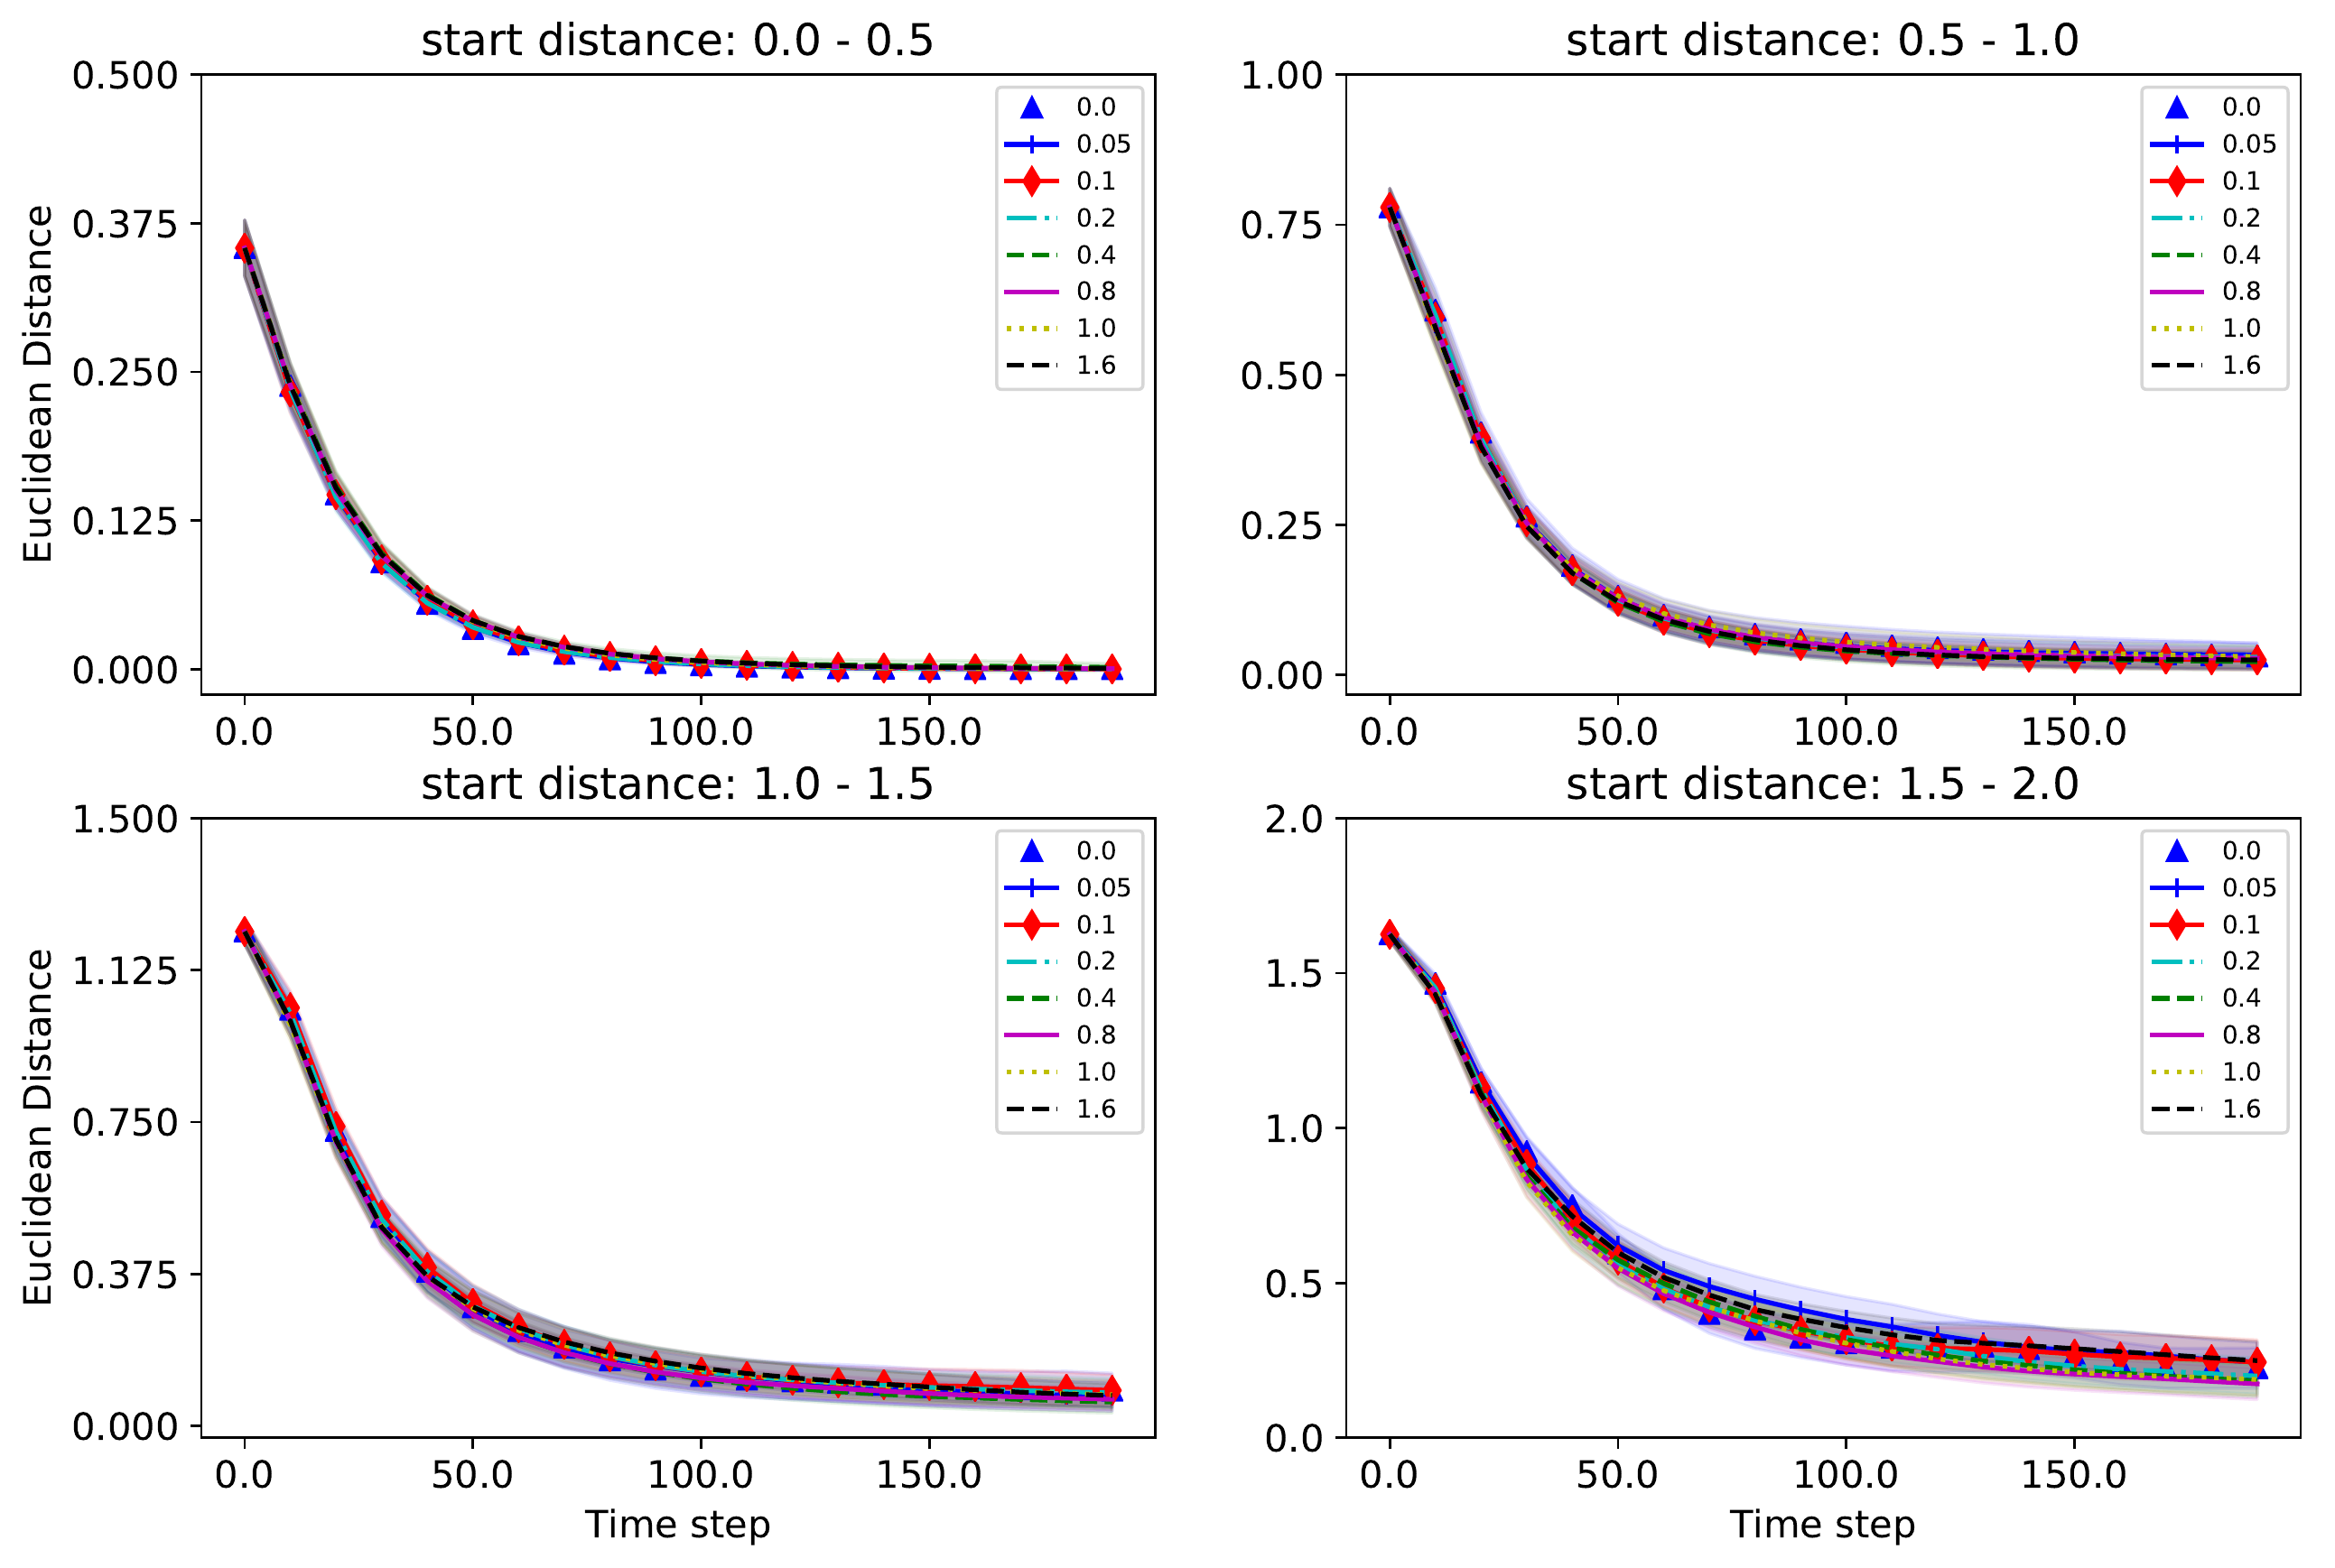}  
  \caption{Single Point Alignment}
  \label{fig:betatuningeuclideandistsinglepoint}
\end{subfigure}
\begin{subfigure}{.5\textwidth}
  \centering
  % include second image
  \includegraphics[width=\linewidth]{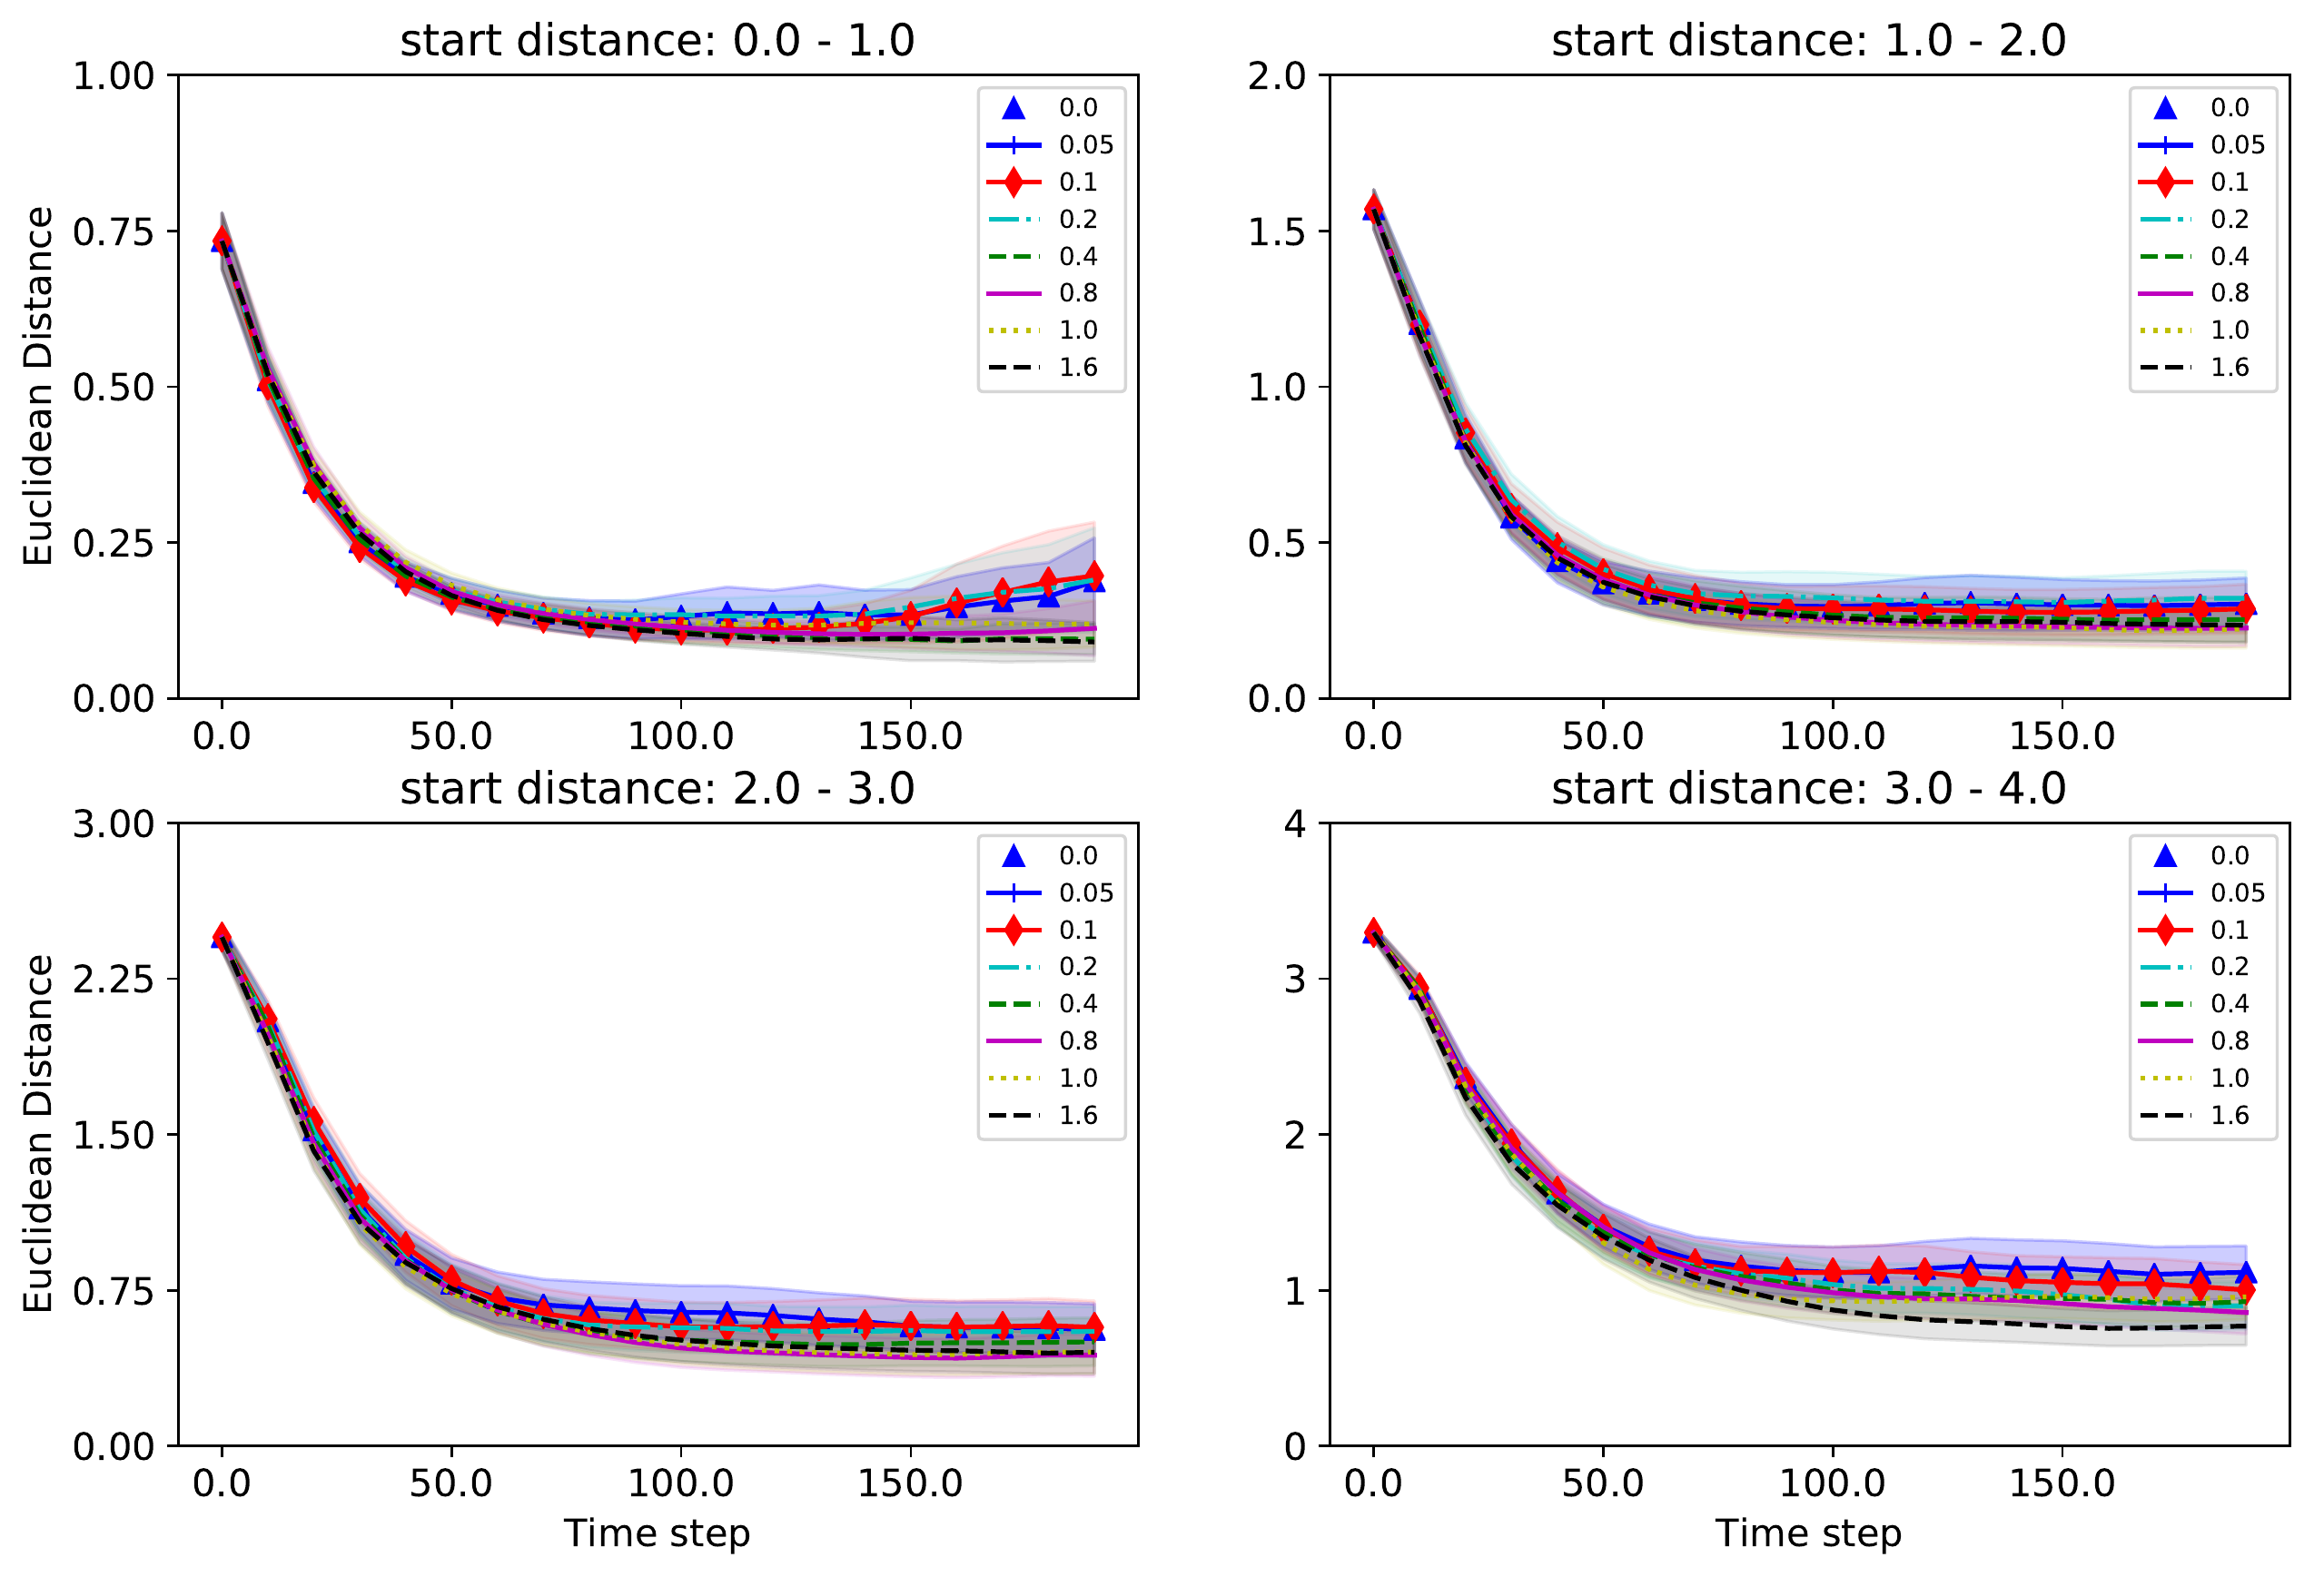}  
  \caption{Multi-point alignment}
  \label{fig:betatuningeuclideandistMultipoint}
\end{subfigure}

\caption{Euclidean distance (meters) to target with varying the weighting term in the Multitask Neural Jacobian. Plotted are the average performances across trajectories separate by initial starting distances. The filled area is the standard error of the mean. For the multi-point case distance is the sum of each point's distance to their respective targets.}
\label{fig:betatuningeuclideandist}
\end{figure}

\begin{table}[]
\centering
\setlength{\tabcolsep}{3 pt}

{\small
\begin{tabular}{c|c|c|c|c|c|c|c|c|c|c|c|}
\cline{2-12}
\multicolumn{1}{l|}{\textbf{}}         & \multicolumn{11}{c|}{\textbf{Initial Euclidean Distance (meters)}}                                                                                                                                                      \\ \cline{2-12} 
\multicolumn{1}{l|}{}                  & \multicolumn{5}{c|}{\textbf{Single Point}}                                                           &           & \multicolumn{5}{c|}{\textbf{Multiple Points}}                                                        \\ \hline
\multicolumn{1}{|c|}{\textbf{$\beta$}} & \textbf{0.0 - 0.5} & \textbf{0.5 - 1.0} & \textbf{1.0 - 1.5} & \textbf{1.5 - 2.0} & \textbf{Overall} &           & \textbf{0.0 - 1.0} & \textbf{1.0 - 2.0} & \textbf{2.0 - 3.0} & \textbf{3.0 - 4.0} & \textbf{Overall} \\ \hline
\multicolumn{1}{|c|}{\textbf{0.0}}     & \textbf{98.96}     & 85.53              & \textbf{74.75}     & 41.84              & \textbf{77.40}   & \textbf{} & 58.56              & 40.19              & 22.63              & 9.09               & 30.23            \\ \hline
\multicolumn{1}{|c|}{\textbf{0.05}}    & 98.94              & 83.26              & 74.64              & 37.60              & 76.02            & \textbf{} & 58.56              & 40.19              & 22.63              & 9.09               & 30.23            \\ \hline
\multicolumn{1}{|c|}{\textbf{0.1}}     & 98.92              & \textbf{86.03}     & 69.66              & \textbf{45.18}     & 75.86            & \textbf{} & 61.21              & 40.58              & 24.20              & 10.19              & 31.41            \\ \hline
\multicolumn{1}{|c|}{\textbf{0.2}}     & 98.97              & 84.97              & 69.86              & 42.94              & 75.30            & \textbf{} & 57.47              & 35.84              & 22.81              & \textbf{10.74}     & 28.88            \\ \hline
\multicolumn{1}{|c|}{\textbf{0.4}}     & 98.00              & 85.58              & 73.23              & 42.48              & 76.77            & \textbf{} & 66.53              & 43.54              & 25.70              & 10.73              & \textbf{33.64}   \\ \hline
\multicolumn{1}{|c|}{\textbf{0.8}}     & 98.82              & 84.78              & 71.07              & 43.08              & 75.72            & \textbf{} & 63.96              & 42.56              & \textbf{26.42}     & 7.40               & 32.92            \\ \hline
\multicolumn{1}{|c|}{\textbf{1.0}}     & 98.82              & 83.38              & 70.53              & 39.07              & 74.52            & \textbf{} & 63.10              & \textbf{44.91}     & 25.78              & 5.58               & 33.17            \\ \hline
\multicolumn{1}{|c|}{\textbf{1.6}}     & 98.44              & 84.70              & 65.85              & 35.82              & 72.67            & \textbf{} & \textbf{69.80}     & 39.61              & 25.29              & 9.04               & 32.12            \\ \hline
\end{tabular}
}
\caption{Percentage of successfully reaching targets for different values of $\beta$ in Multitask Neural Jacobian method. We use the average success percentages for thresholds from 0.0m - 0.1m from target for single-point  and the AUC for 0.0m - 0.25m for multi-point. In bold are the best performance for each distance. In multi-point setting the distance is the sum of distances for all points to their respective targets.}
\label{tab:tuningbetasuccesses}
\end{table}
\subsection{Jacobian Conditioning of Environments}

\begin{table}[]
\begin{tabular}{c|c|c|c|c|}
\cline{2-5}
                                                         & \multicolumn{2}{c|}{Single Point} & \multicolumn{2}{c|}{Multiple Points} \\ \cline{2-5} 
                                                         & mean       & standard deviation   & mean           & standard deviation  \\ \hline
\multicolumn{1}{|c|}{\textbf{Broyden}}                   & 11.658     & 25.373               & 6.070931e+14   & 5.305740e+15        \\ \hline
\multicolumn{1}{|c|}{\textbf{Finite Difference}}         & 15.933     & 0.000                & 3.785613e+16   & 1.600000e+01        \\ \hline
\multicolumn{1}{|c|}{\textbf{KNN Local Linear}}          & 141.677    & 40410.916            & 1.846220e+02   & 3.844440e+02        \\ \hline
\multicolumn{1}{|c|}{\textbf{Multitask Neural Jacobian}} & 3.290      & 1.795                & 1.085200e+01   & 3.987000e+00        \\ \hline
\multicolumn{1}{|c|}{\textbf{Neural Jacobian}}           & 5.101      & 4.067                & 1.520790e+02   & 1.313760e+02        \\ \hline
\multicolumn{1}{|c|}{\textbf{Neural Kinematics}}         & 5.428      & 4.463                & 2.007880e+02   & 1.743080e+02        \\ \hline
\multicolumn{1}{|c|}{\textbf{True Jacobian}}             & 5.025      & 4.456                & 1.877426e+08   & 1.278614e+08        \\ \hline
\end{tabular}
\caption{The average Jacobian condition number for each environment by algorithm. We found that between methods that there was not a significant difference, but between environment the conditioning was much more notable.}
\label{tab:jacobiancond}
\end{table}

In this experiment we looked at the matrix condition number for the Jacobians at each step of control for all algorithms and for each step of control. The condition number gives us an idea of how close to singularities, or linear dependence our matrices are \cite{heath1996scientificcomputing}. Closer to 1 suggest better conditioned matrices that are robust to noise. For this analysis we averaged across all Jacobian calculations in our experiments. These included each step of a trajectory across all collected trajectories. We note this does not give a complete picture of conditioning between algorithms, and is primarily to illustate the challenges between the single point and multi point experiments.  The results are included in Table~\ref{tab:jacobiancond}. Between algorithms we observed some noticeable differences between average Jacobian conditioning for different approximations in the single point case. Across environments, the much large magnitudes of condition numbers in the multi-point environment demonstrates the difficulty of this task, where all algorithms are much more poorly conditioned for the task, including the true Jacobian. 
\subsection{Sensitivity of Number of Neighbours}

In this section we provide results from tuning the number of neighbours in our KNN Neural Jacobian method. We only conducted the experiment on the multi-point environment using the same trajectories in our control experiments. The hyperparameters are almost entirely the same as our other multi-point experiments. One exception is that we use 50 epochs to train over as opposed to the 40 in the original experiment. We increased the number of epochs to allow sufficient time for the model to converge, even if the best performance on the validation set occurred much earlier. We tried values 2, 4, 8, 16, 32, 64 for the neighborhood. We did not try a higher number of neighbors as our current results suggest the number of neighbors is not that sensitive, and with our implementation we stored the dataset in memory so the cost was too much. 
We also tuned over the number of neighbors in the local linear baseline. We include the percentage of successful controls to the target point and the Condition number. We also plotted the Jacobian error, but our results were generally consistent with previous work with the Local linear method. An interesting exception was our results with eight neighbors. We found that our Jacobian estimates exploded. We conjecture that this is because when the number of neighbors is small 

\begin{figure}[ht]
\begin{subfigure}{.5\textwidth}
  \centering
  % include first image
  \includegraphics[width=\linewidth]{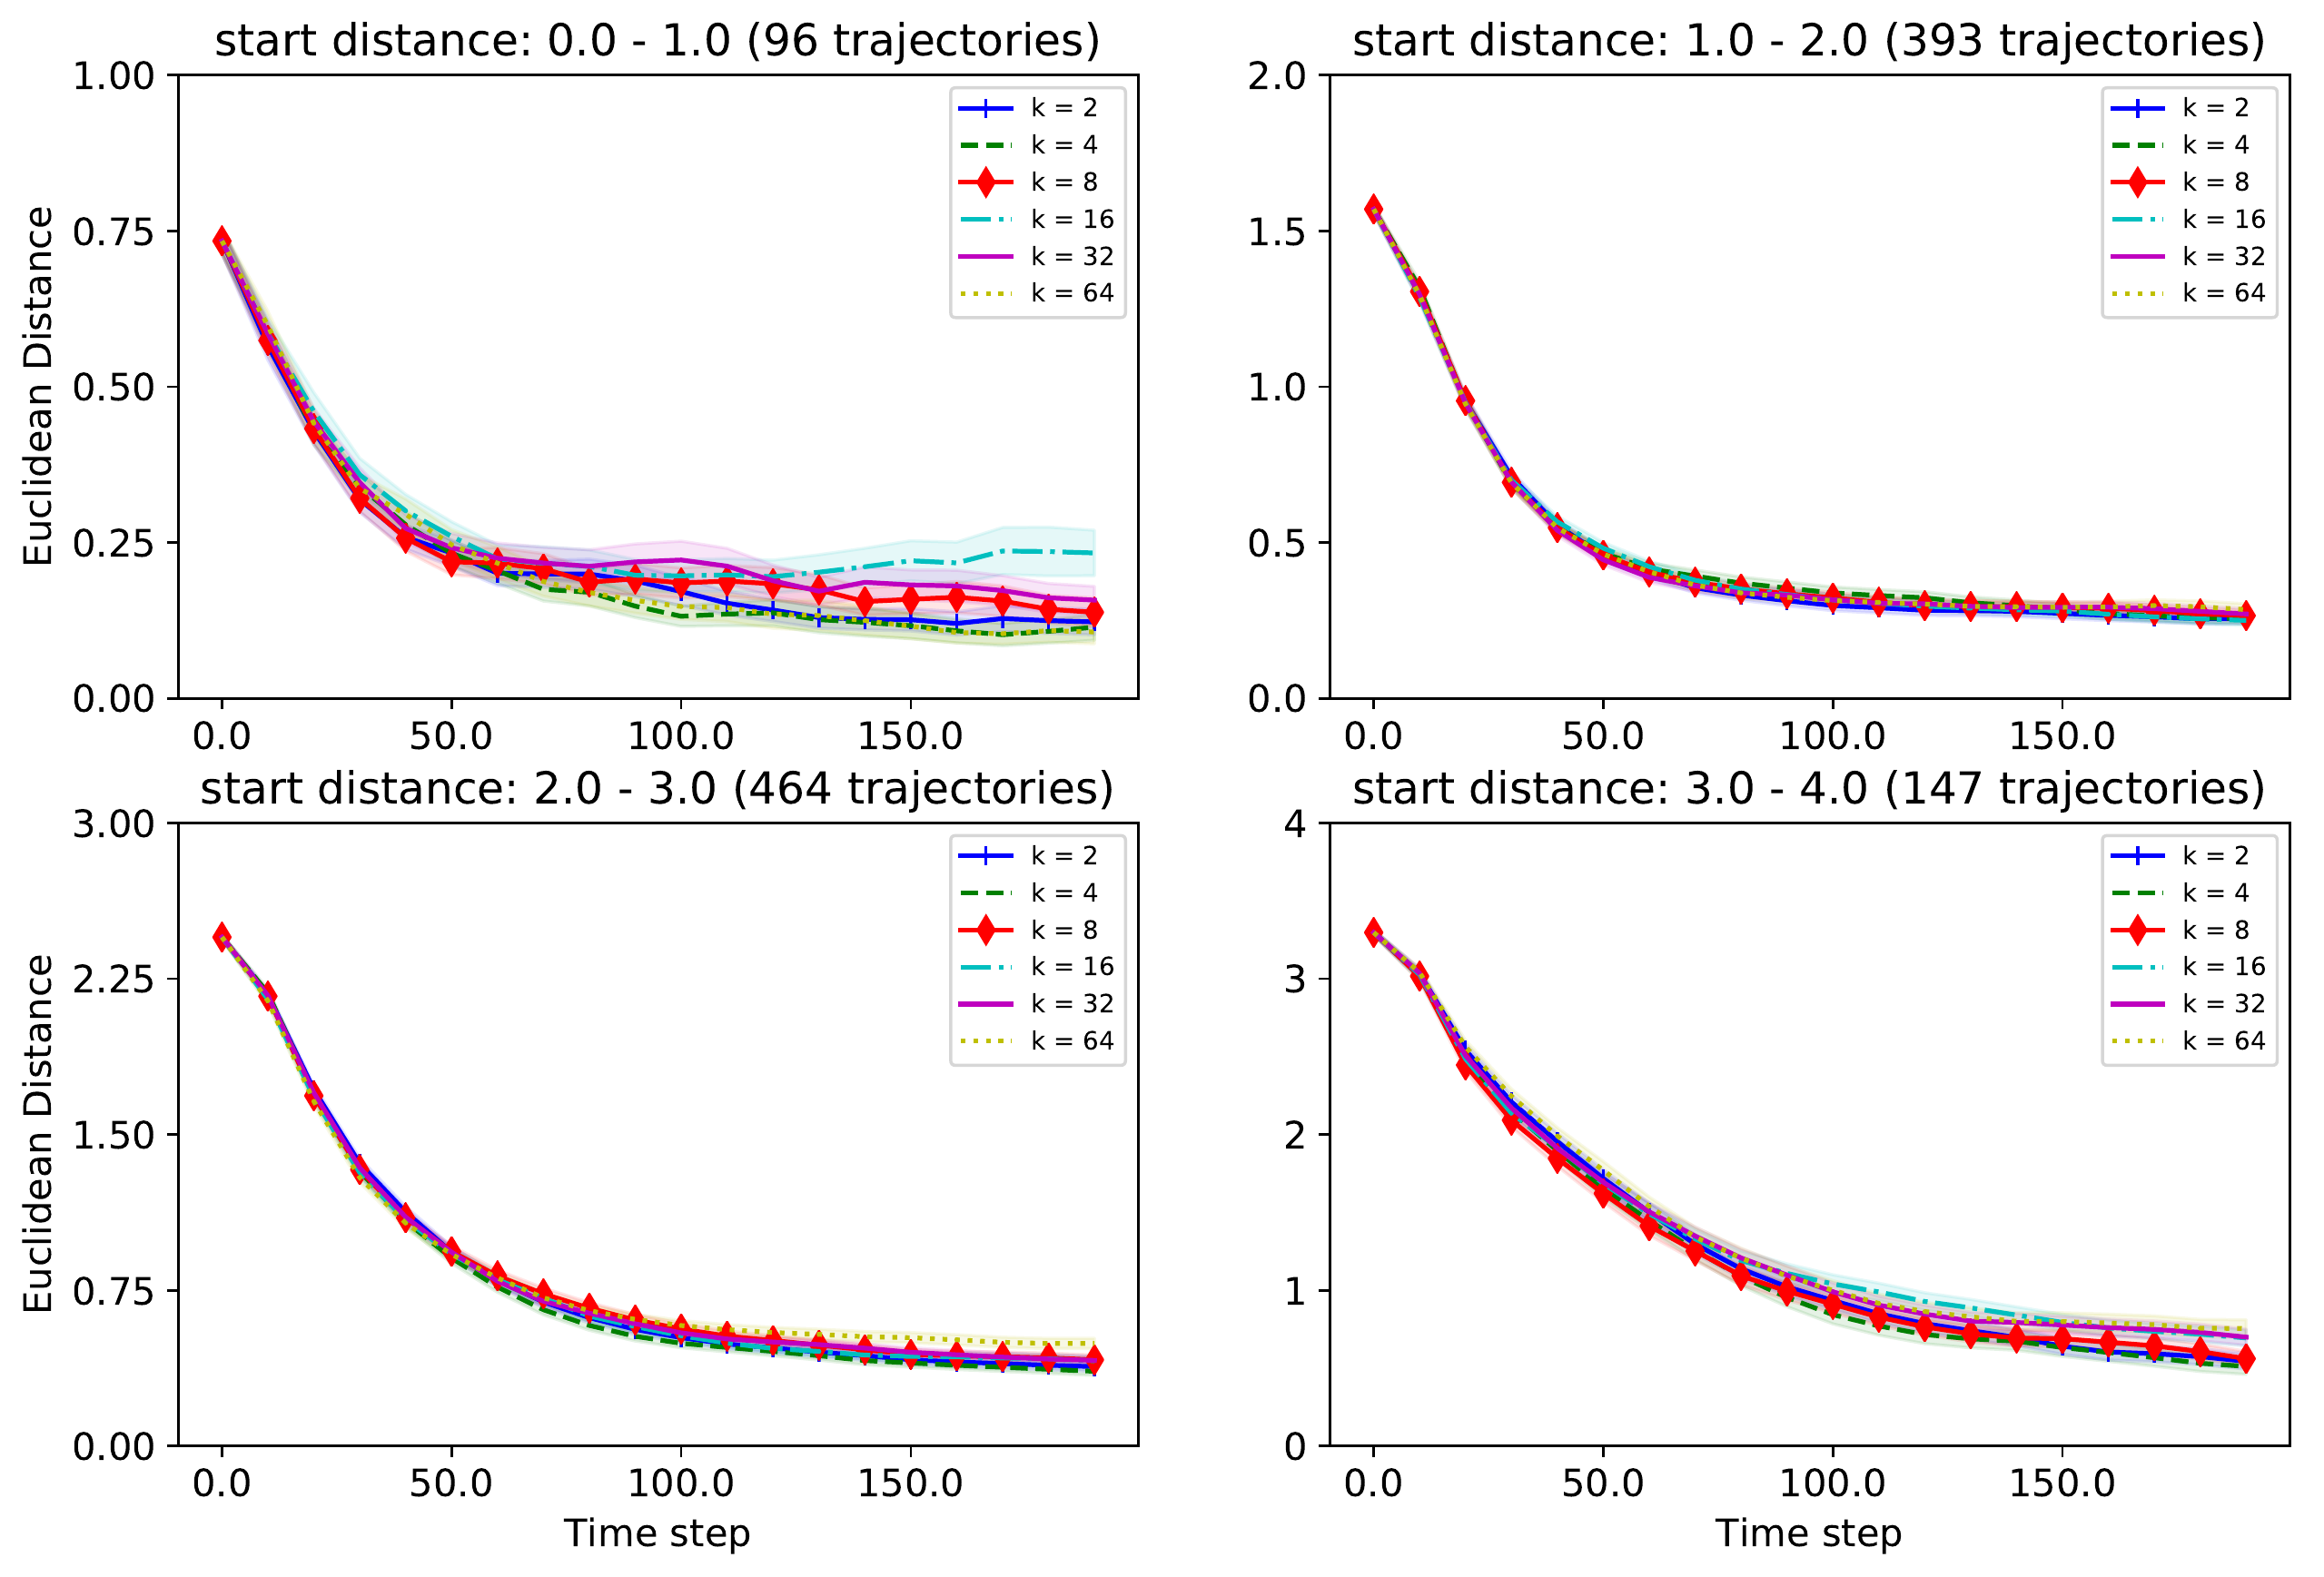}  
  \caption{Vanilla KNN Neural Jacobian}
  \label{fig:betatuningeuclideandistsinglepoint}
\end{subfigure}
\begin{subfigure}{.5\textwidth}
  \centering
  % include second image
  \includegraphics[width=\linewidth]{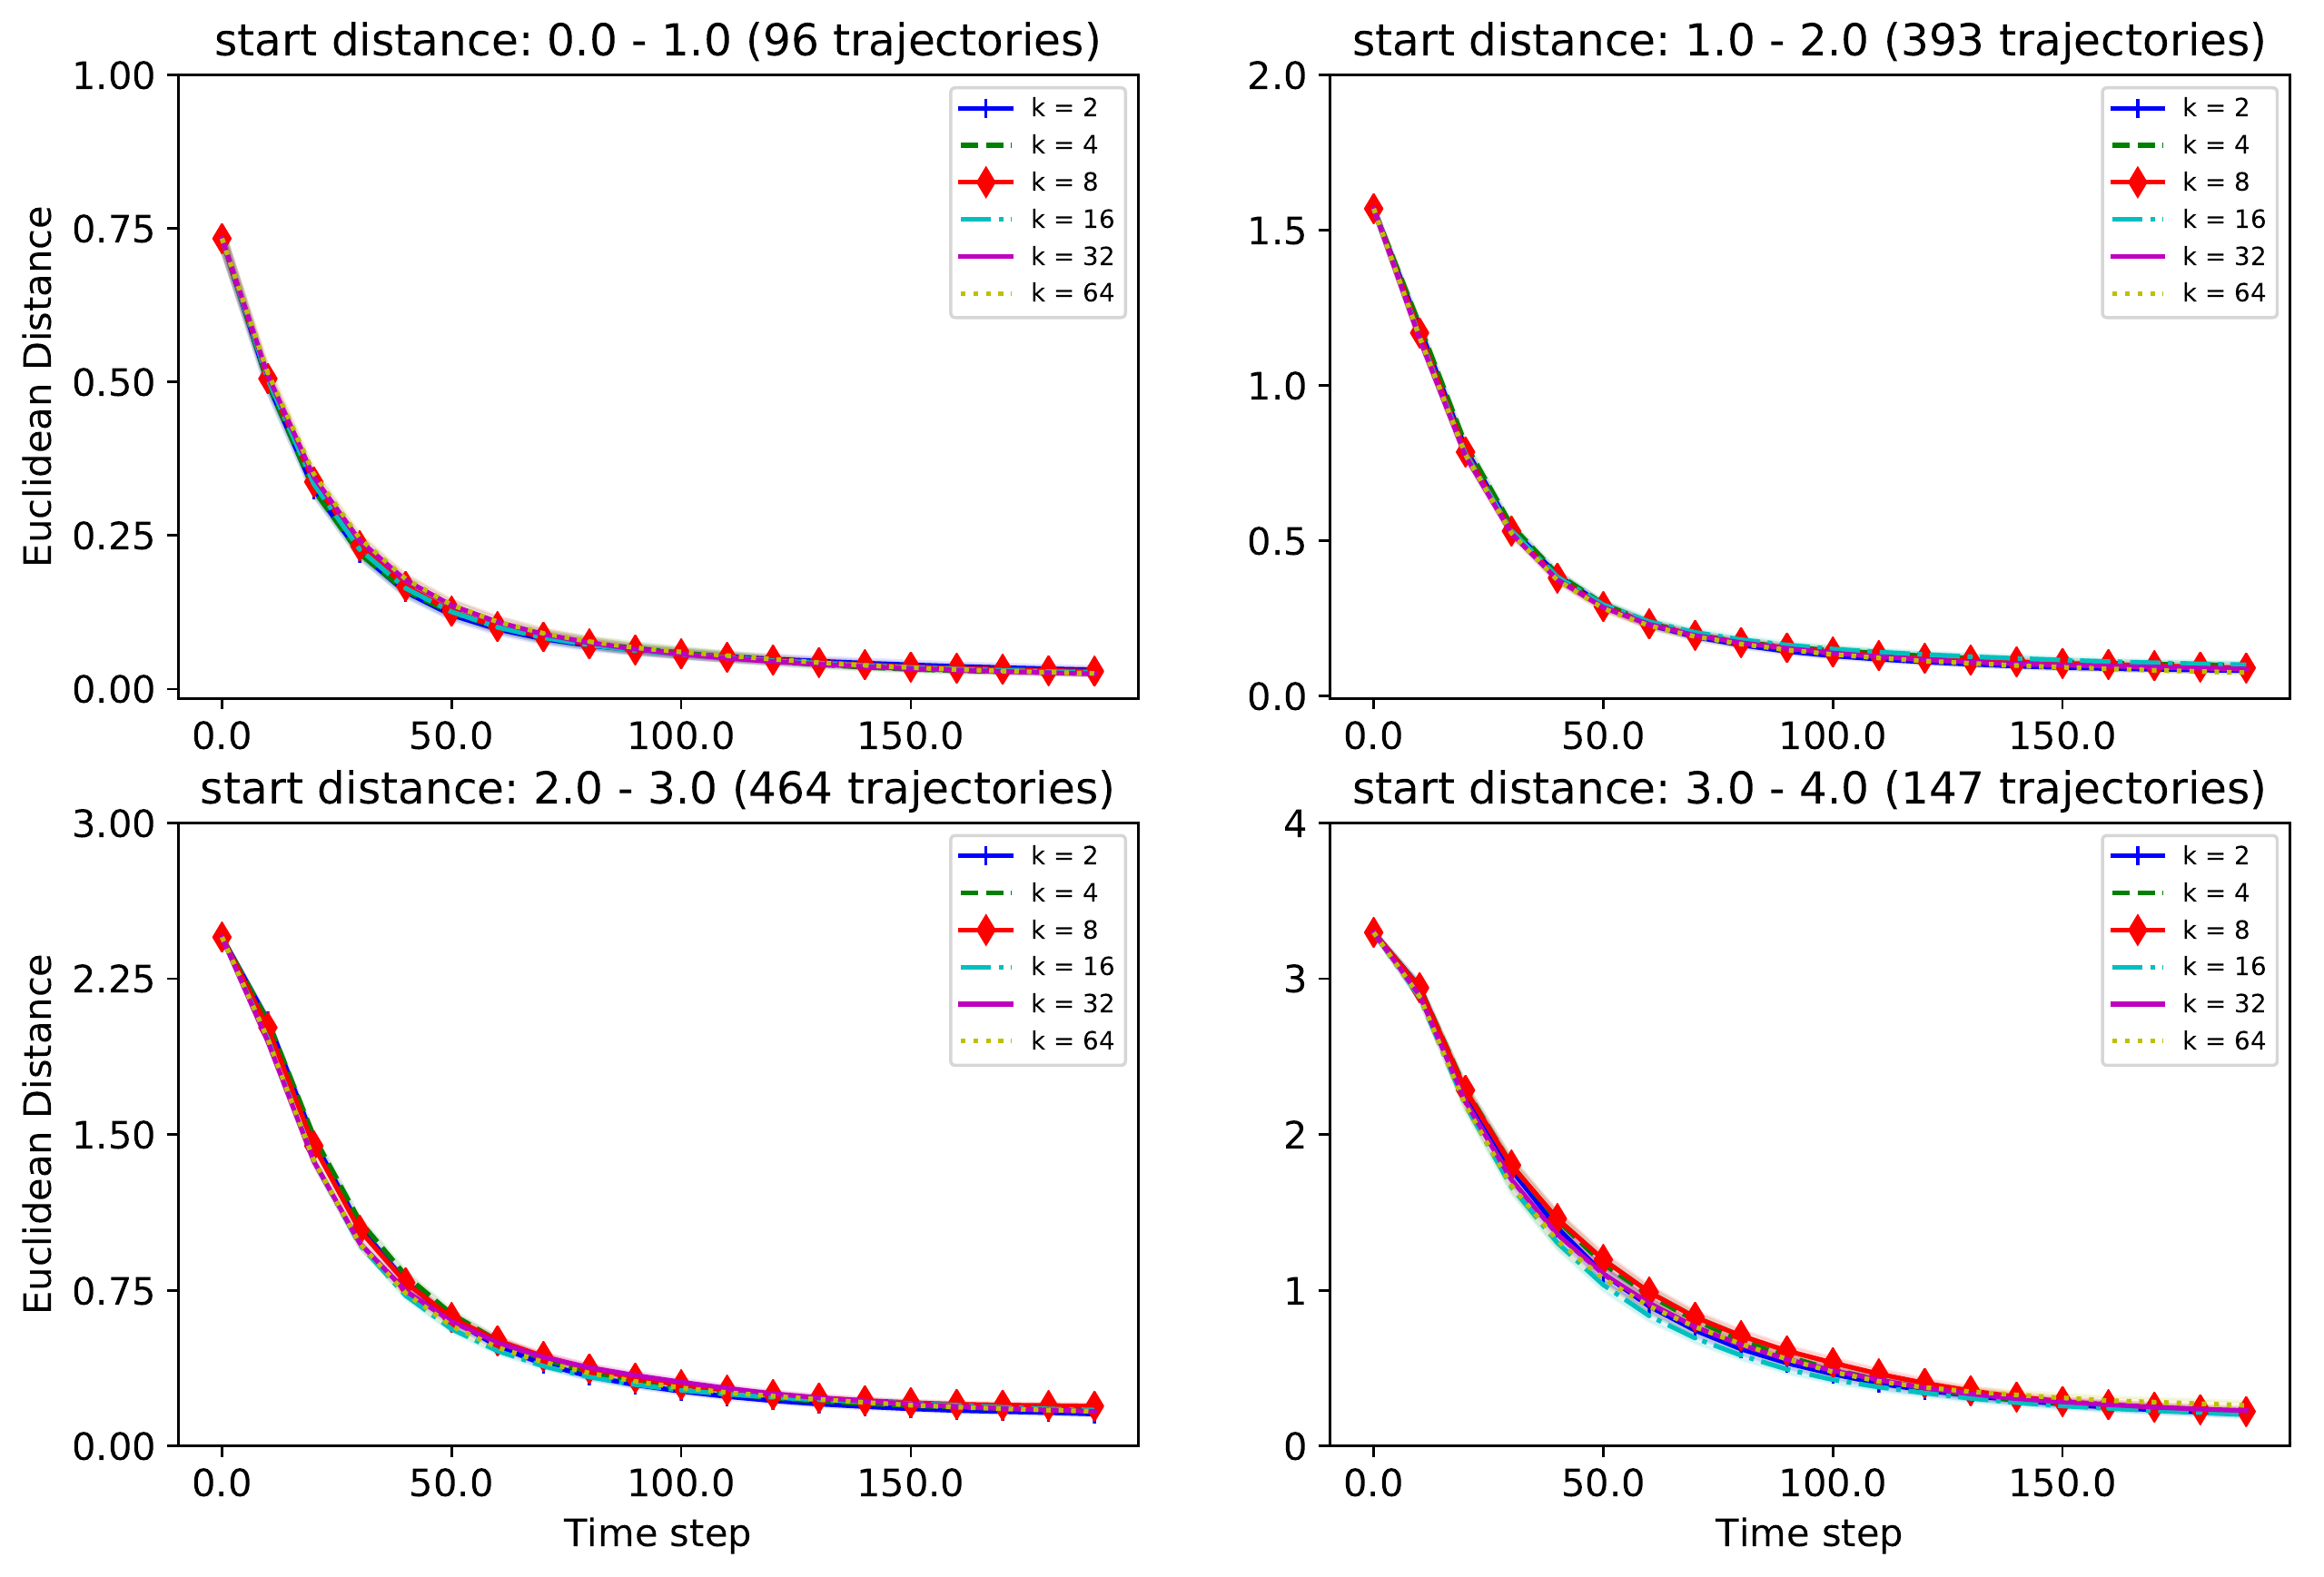}  
  \caption{Multitask KNN Neural Jacobian}
  \label{fig:betatuningeuclideandistMultipoint}
\end{subfigure}

\caption{Performance of different neighborhood sizes for the KNN Neural Jacobian method on the Multiple Point environment.}
\label{fig:knnsensitivityeuclideandist}
\end{figure}

\begin{table}[]
\centering
\setlength{\tabcolsep}{3 pt}

{\small
\begin{tabular}{|c|c|c|c|c|c|c|c|c|c|c|c|}
\hline
           & \multicolumn{5}{c|}{\textbf{KNN Neural Jacobian}}                                                         &           & \multicolumn{5}{c|}{\textbf{Multitask KNN Neural Jacobian}}                                               \\ \hline
\textbf{K} & \textbf{0.0 - 1.0 m} & \textbf{1.0 - 2.0 m} & \textbf{2.0 - 3.0 m} & \textbf{3.0 - 4.0} & \textbf{Overal} & \textbf{} & \textbf{0.0 - 1.0 m} & \textbf{1.0 - 2.0 m} & \textbf{2.0 - 3.0 m} & \textbf{3.0 - 4.0} & \textbf{Overal} \\ \hline
2          & 68.02                & 49.51                & 39.61                & 26.00              & 43.81           &           & 88.30                & 74.29                & 59.30                & 41.70              & 64.83           \\ \hline
4          & 70.94                & 49.26                & 38.87                & 25.25              & 43.56           &           & 89.93                & 70.75                & 56.10                & 38.32              & 61.91           \\ \hline
8          & 65.42                & 47.70                & 37.56                & 24.14              & 41.82           &           & 88.83                & 72.61                & 55.33                & 40.81              & 62.49           \\ \hline
16         & 57.03                & 50.19                & 34.64                & 15.75              & 39.63           &           & 89.55                & 72.09                & 57.20                & 46.54              & 63.92           \\ \hline
32         & 59.88                & 50.21                & 34.42                & 20.46              & 40.42           &           & 90.51                & 74.19                & 58.65                & 42.51              & 64.82           \\ \hline
64         & 71.27                & 48.54                & 32.60                & 18.19              & 39.75           &           & 90.32                & 77.42                & 60.52                & 41.28              & 66.59           \\ \hline
\end{tabular}
}
\label{tab:knnsensitivity}
\caption{Success percentages averaged from 0.0 - 0.25 with increments of 0.001 steps.}
\end{table}
