# Supplementary material for: Analyzing Neural Jacobian Methods in Applications of Visual Servoing and Kinematic Control
Source: arXiv:2106.06083 source file (2021-06-10)
Supplement: Supplementary file 8 [file baseline_methods.tex]

\section{Baseline Methods}
In this section, we describe the details of each of the baseline methods we compared against. This included the true Jacobian, finite difference method~\cite{jagersand96visualservoing}, the Broyden method~ \cite{jagersand96visualservoing}, and the Local Linear method \cite{farahmand2007globaluvs}. As the Broyden method and finite difference method are closely related, they are described together.

\subsection{True Robotic Jacobian}

Here we include relevant equations that describe the true Jacobian for the 2-DOF environment we mapped to the Kinova. With two planar rotation joints the position of the end-effector can be described by the following equations:
\begin{equation}
    x = 
        \begin{bmatrix}
         L_{1} cos(q_{1}) + L_{2} cos(q_{1} + q_{2})\\L_{1}sin(q_{1}) + L_{2} sin(q_{1} + q_{2})
        \end{bmatrix}
\end{equation}.

Using the equation for robotic motion in the main paper, when we  differentiate with respect to time, we get the following Jacobian: 
\begin{equation}
 \dot{x} =
        \begin{pmatrix}
         -L_{1}sin(q_{1}) - L_{2} sin(q_{1} + q_{2}) &
         - L_{2} sin(q_{1} + q_{2})
         \\
         L_{1} cos(q_{1}) + L_{2} cos(q_{1} + q_{2}) &
         L_{2} cos(q_{1} + q_{2})
        \end{pmatrix}
        \begin{pmatrix}
            \dot{q_{1}} \\  \dot{q_{2}}
        \end{pmatrix} 
\end{equation}
Here, $L_{1}$ and $L_{2}$ our the lengths of the robot links. We exclude writing $J^k{-1}$, but note that it can be found analytically using the fact $J$ is a 2-by-2 matrix. For our simulators, we found that analytically writing the Jacobian would be fairly complex for the 7 DOF manipulator, and instead we used a backpropagation library to handle calculating the Jacobian \cite{jax2018github}.

\subsection{k Nearest Neighbor Local Linear Jacobian Estimation}
Previous research on Jacobian approximation has utilized the observation that the Jacobian is a hyperplane at the instantaneous point of evaluation \cite{farahmand2007globaluvs}. This work considered directly fitting such a hyper-plane utilizing the assumption that the equations of robot motion can be approximated as finite differences $\Delta x \approx J(q_{t}) \Delta q$ for time step $t$ in a trajectory, leading to the following objective: 
\begin{equation}
    \min_{J} \sum^{k}_{i=1}\sum^{k}_{j=1}|| \Delta x_{ij} - J\Delta q_{ij} ||_{2}^{2},
\end{equation}
where $\Delta x_{ij}$ and $\Delta q_{ij}$ are the finite difference between the k-nearest neighbor (k-NN) points to the current angles $q_{t}$ we want to calculate the Jacobian. This objective function is then optimized online when controlling the robot, and can be anlytically solved by differentiating with respect to the Jacobian J. This method requires storing all the interactions with the robot to select the k-NN neighbors to be optimized over. In our experiments we used $k=50$ for evaluation based on previous works experimental results \cite{farahmand2007globaluvs}.

\subsection{Broyden Jacobian Estimation}

One classic approach to estimating the Jacobian is by making small, independent movements of each joint from some initial pose \cite{ramirez2018libraryUVS}. In a 2-DOF planar reaching environment, this matrix is found as follows:   
\begin{equation}
    J \approx \hat{J}=
    \begin{pmatrix}
        \frac{x^{t} - x^{0}}{q^{t}_{1} - q^{0}_{1}} & \frac{x'^{t} - x^{0}}{ q^{t}_{2} - q^{0}_{2}}\\[\jot]
        \frac{y^{t} - y^{0}}{q^{t}_{1} - q^{0}_{1}} & \frac{y'^{t} - y^{0}}{ q^{t}_{2} - q^{0}_{2}}\\[\jot]
    \end{pmatrix}.
\end{equation}
Here, $t$ is the position after some amount of movement. Note that, for each columns approximation we assume the same initial position $(x^{0}, y^{0})$. We only include the coordinates for a 2-dimensional point, but the matrix is similar for 3D points as well. For each column of this matrix, we move the joints sufficiently far such that the change in position is non-negligible. To improve the estimate of this Jacobian we can then make Broyden updates of the Jacobian as follows:
\begin{equation}
 \hat{J}_{k+1} = \hat{J}_{k} + \alpha \frac{(\Delta e - \hat{J}_{k}\Delta q) \Delta q^{T}}{||\Delta q||_{2}^{2}}.
\end{equation}
Here $\Delta$ is for changes from the last tracked measurements, and $e = x^{*} - x$. A limitation of the Broyden update is it requires the change in joint angles $\Delta q$ be sufficiently large. In our experiments for the Broyden method, we only take the update if $||\Delta q||_{2}^{2} \geq 0.01$ and used $\alpha=0.1$ when updating the approximation $\hat{J}_{k}$.
