# Supplementary material for: Analyzing Neural Jacobian Methods in Applications of Visual Servoing and Kinematic Control
Source: arXiv:2106.06083 source file (2021-06-10)
Supplement: Supplementary file 9 [file environment_details.tex]

\section{Environment Details}

\begin{table}[]
\centering
\begin{tabular}{c|c|c|c|c|c|c|}
\cline{2-7}
\textbf{}                                            & \textit{\textbf{$x$}} & \textit{\textbf{$\cos(q)$}} & \textit{\textbf{$\sin(q)$}} & \textit{\textbf{$\dot{q}$}} & \textit{\textbf{$x^{*}$}} & \textit{\textbf{$s$}} \\ \hline
\multicolumn{1}{|c|}{\textit{\textbf{Single Point}}} & 3                     & 7                           & 7                           & 7                           & 3                         & 27                    \\ \hline
\multicolumn{1}{|c|}{\textit{\textbf{Multi Point}}}  & 12                    & 7                           & 7                           & 7                           & 12                        & 45                    \\ \hline
\multicolumn{1}{|c|}{\textit{\textbf{Kinova}}}       & 2                     & 2                           & 2                           & 2                           & 2                         & 10                    \\ \hline
\end{tabular}
\caption{Dimensions of different aspects of the robot state $s$ for each environment. This includes end-effector location $x$, joint angles $q$, joint velocities $\dot{q}$, and target location $x^{*}$, where $s$ is the sum of these dimensions. Commands sent to the environments were joint velocities $\dot{q}$.}
\label{tab:statedimensions}
\end{table}
We describe the details for our simulated and robotic environments in this section. All our environments are designed similarly to a reinforcement learning gym \cite{brockman2016OpenAIGYM} where the actions are joint velocities $\dot{q}$ and we receive the robot state as a vector $s$. Each environment consists of the same robotic information, only differing in the dimensions of each feature. We list these dimensions for each environment in Table~\ref{tab:statedimensions}.

In both simulated and robotic environments, we utilize the Kinova's kinematics equations for generating the location of targets. As mentioned in the background section, we used the Denavit-Hartenberg (DH) parameters for the Kinova's kinematics. The DH matrix is as follows:
\begin{equation}
 ^{i-1}T_{i} =
\begin{pmatrix}
 \cos(q_{i}) & -\cos(\alpha_{i})\sin(q_{i}) & \sin(\alpha_{i})\sin(q_{i}) & a_{i}\cos(q_{i})\\
 \sin(q_{i}) & \cos(\alpha_{i})\cos(q_{i}) & -\sin(\alpha_{i})\cos(q_{i}) & a_{i}\sin(q_{i})\\
 0 & \sin(\alpha_{i}) & \cos(\alpha_{i}) & d_{i}\\
 0 & 0 & 0 & 1 
\end{pmatrix}.
\end{equation}
For each transformation $^{i-1}T_{i}$ of the Kinova, the values can be found in Table~\ref{tab:kinovadhvalues}. 

\begin{figure}[ht]
\begin{subfigure}{.5\textwidth}
  \centering
  % include first image
  \includegraphics[width=.7\linewidth]{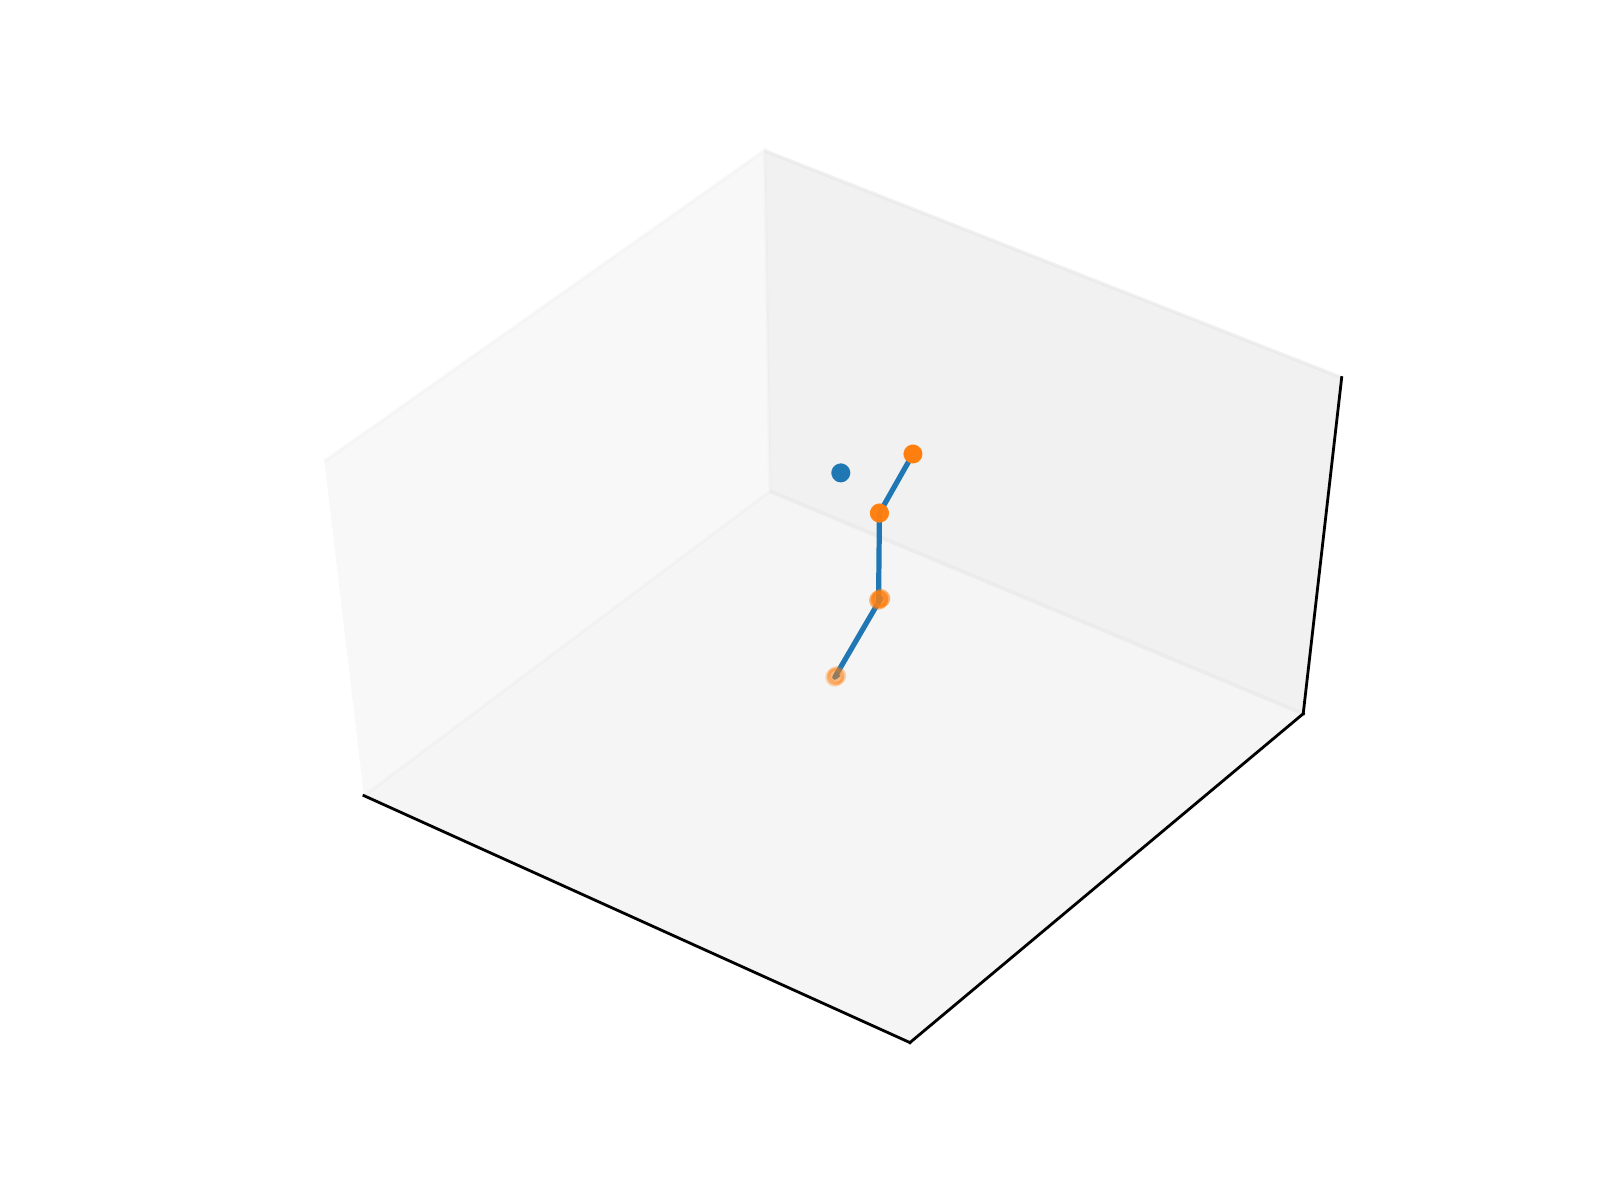}  
  \caption{Point to Point Environment}
  \label{fig:1ptsimulator}
\end{subfigure}
\begin{subfigure}{.5\textwidth}
  \centering
  % include second image
  \includegraphics[width=.7\linewidth]{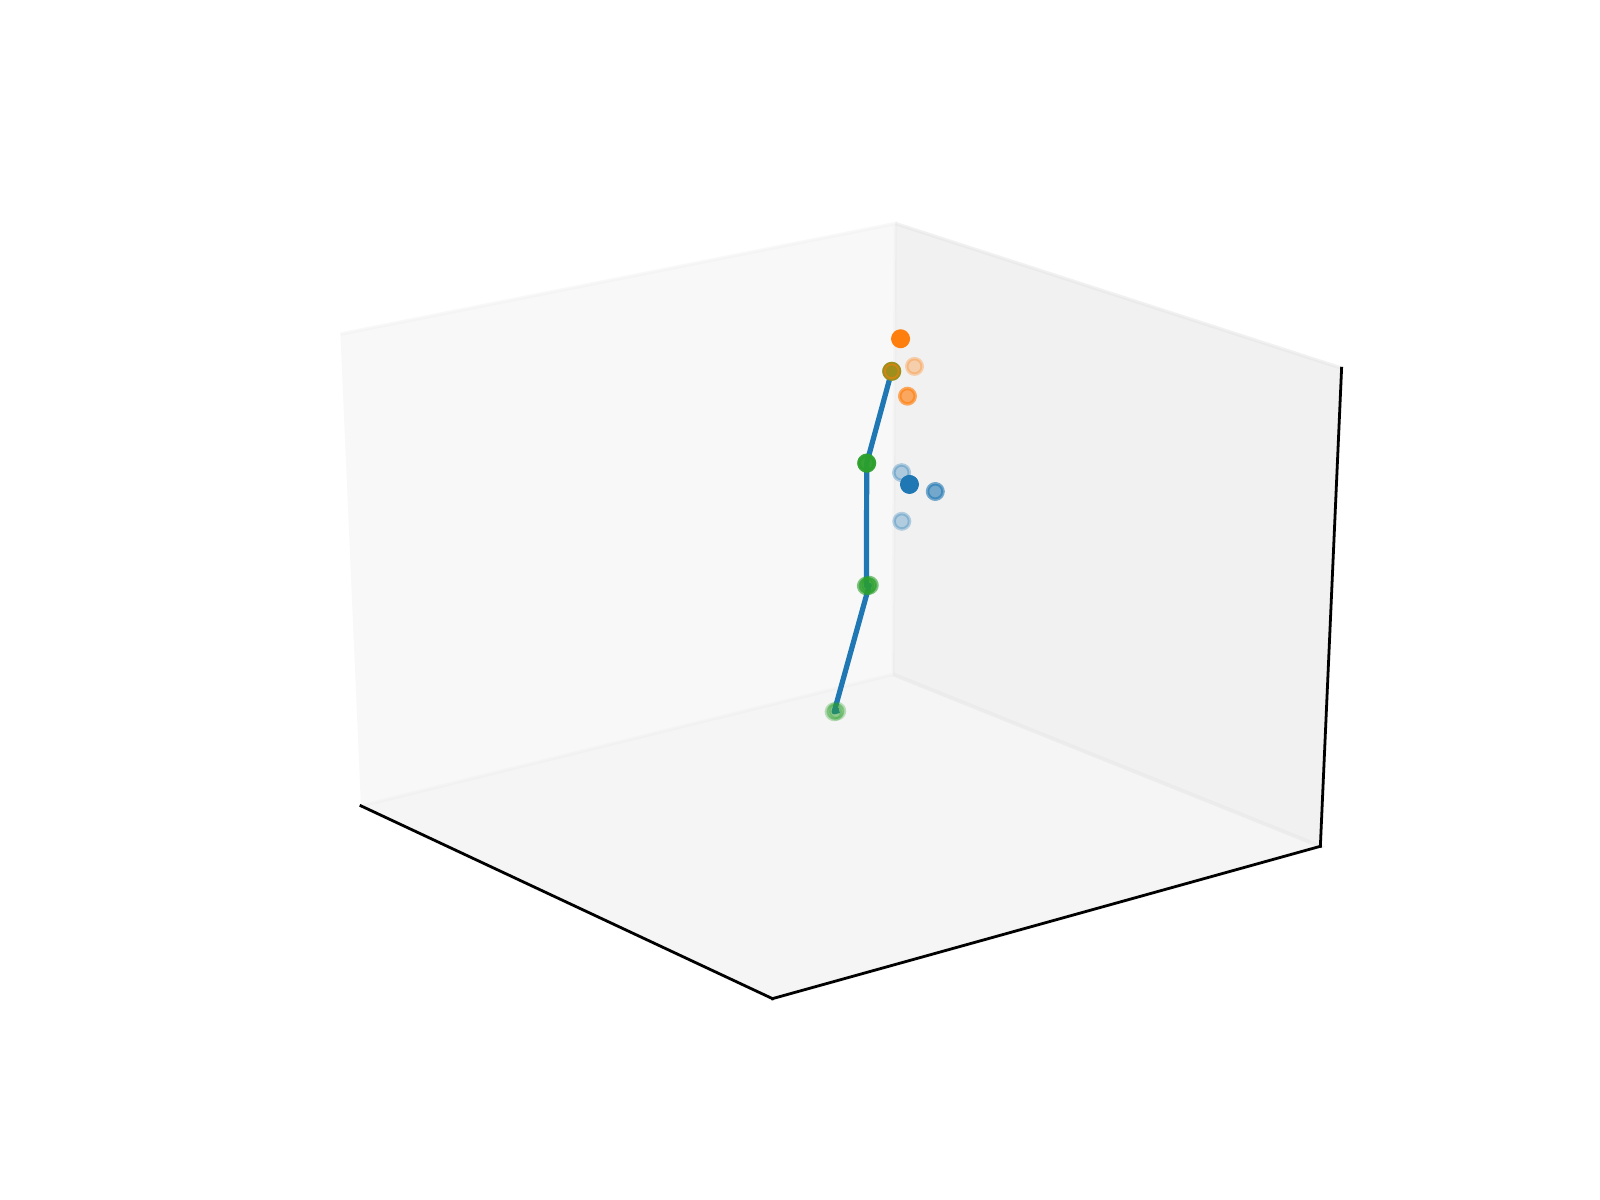}  
  \caption{Position and Orientation Environment}
  \label{fig:4ptsimulator}
\end{subfigure}
\caption{Visualization of kinematic simulators. The objective in both simulators is to align robot points (orange) to match exactly with corresponding target points (blue) }
\label{fig:simulators}
\end{figure}

\paragraph{Simulator Details} Our simulator environments are visualized in Figure~\ref{fig:simulators}, and were implemented with the DH parameter values in Table~\ref{tab:kinovadhvalues}. They only differ in the number of points we wish to move to a target position. In the single point case, we only translate a single homogeneous vector $p=[0,0,0,1]$ with the kinematics equations to represent the end-effector. In the multi-point case we include 3 additional vectors, where each is a scaled unit-vectors of the orientation for the x, y, and z axis. We found using one-tenth of a unit vector the best for visualizing the points representing orientation (e.g. $p_{z}=[0, 0, .1, 1]$ as opposed to $p_{z}=[0, 0, 1, 1]$). When joint velocities are sent, the current joint values are updated as $q_{t+1} = q_{t} + \Delta t \dot{q_{t}}$, where $\Delta t=0.05 \text{(seconds)}$ represents our simulated time. The position of the robot is then updated and a new state vector is sent with the updated information to our controller.

\begin{table}[]
\centering
\begin{tabular}{|c|c|c|c|c|}
\hline
\textbf{i}    & \textbf{$\alpha_{i}$ (radians)} & \textbf{$a_{i}$(m)} & \textbf{$d_{i}$(m)} & \textbf{$q_{i}$ (radians)} \\ \hline
0 (from base) & $\pi$                           & 0.0                 & 0.0                 & 0                               \\ \hline
1             & $\pi / 2$                       & 0.0                 & -(0.1564 + 0.1284)  & $q_{1}$                         \\ \hline
2             & $\pi / 2$                       & 0.0                 & -(0.0054 + 0.0064)  & $q_{2} + \pi$                   \\ \hline
3             & $\pi / 2$                       & 0.0                 & -(0.2104 + 0.2104)  & $q_{3} + \pi$                   \\ \hline
4             & $\pi / 2$                       & 0.0                 & -(0.0064 + 0.0064)  & $q_{4} + \pi$                   \\ \hline
5             & $\pi / 2$                       & 0.0                 & -(0.2084 + 0.1059)  & $q_{5} + \pi$                   \\ \hline
6             & $\pi / 2$                       & 0.0                 & 0.0                 & $q_{6} + \pi$                   \\ \hline
7             & $\pi$                           & 0.0                 & -(0.1059 + 0.0615)  & $q_{7} + \pi$                   \\ \hline
\end{tabular}
\caption{Table of DH parameter values for the Kinova robot \cite{kinova}. We utilize these numbers for calculating the target location, position of our simulators, and for calculating the true Jacobian.}
\label{tab:kinovadhvalues}
\end{table}

\paragraph{Kinova Details}
\begin{figure}
    \centering
    \includegraphics[width=.3\linewidth]{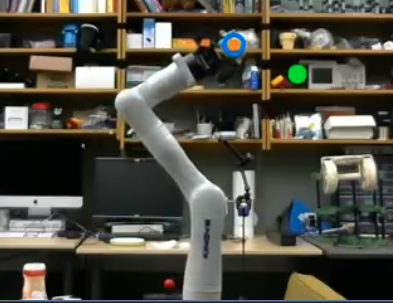}
    \caption{Image of the Kinova Gen 3 light robot used for experiments. Visualization of the tool tip (blue orange circle) and target position (green) in image are to illustrate fundamental idea of the control task. In experiments we work in robot coordinate system.}
    \label{fig:Kinova}
\end{figure}

For our Kinova experiments, we derived the DH parameters for a 2 degree-of-freedom (DOF) planar manipulator. The kinematic transformations can be found in \citet[Chapter 3]{craig1989IntroRobotics} for this planar case. This required transforming the Kinova's coordinate system to align with our planar forward kinematics equations. Specifically, we converted from the Kinova's z-x plane to a x-y coordinate frame, by subtracting an offset of 0.7052 from the Z axis and treated it as our X coordinates while treating the Kinova x coordinate as our y axis. We then interpreted the Kinova's 4th link of length 0.3143 meters as the first link in our 2-DOF robot,  and the Kinova's 6th joint of length 0.1774 meters as the second link. We interacted with the Kinova using the publicly available the Kinova Robotic Operating System (ROS) bindings \cite{ros2018ROS,kinovakortex}. The all features of the robot's state was sensory information from the Kinova. Similarly, joint velocity commands were sent through the ROS bindings. We operated our the Kinova at approximately 20 Hz which corresponded to about 10 seconds for real-time evaluation on the robot per trajectory.
