# Supplementary material for: Analyzing Neural Jacobian Methods in Applications of Visual Servoing and Kinematic Control
Source: arXiv:2106.06083 source file (2021-06-10)
Supplement: Supplementary file 10 [file experiment_details.tex]

\section{Experiment Details}

\begin{table}[]
\centering
{\small
\begin{tabular}{c|c|c|c|}
\cline{2-4}
\textbf{}         & \textbf{Single  Point (Simulation)} & \textbf{Multi-Point (Simulation)} & \multicolumn{1}{l|}{\textbf{Single Point (Kinova)}} \\ \hline
\multicolumn{1}{|l|}{\# of Training Epochs} & 30                                  & 40                                & 45                                                  \\ \hline
\multicolumn{1}{|c|}{\# Hidden Layers}      & 2                                   & 4                                 & 1                                                   \\ \hline
\multicolumn{1}{|c|}{Hidden Layer Size}     & \multicolumn{3}{c|}{100}                                                                                                      \\ \hline
\multicolumn{1}{|c|}{Activation Function}   & \multicolumn{3}{c|}{Relu}                                                                                                     \\ \hline
\end{tabular}
}
\caption{Neural network hyperparameters for each experiment. }
\label{tab:networkparams}
\end{table}

\begin{table}[]
\begin{tabular}{|c|c|c|c|}
\hline
\textbf{Single Point Distances} & \textbf{Counts} & \textbf{Multi-point Distances} & \textbf{Counts} \\ \hline
0.0 - 0.5                       & 106             & 0.0 - 1.0                      & 96              \\ \hline
0.5 - 1.0                       & 414             & 1.0 - 2.0                      & 393             \\ \hline
1.0 - 1.5                       & 455             & 2.0 - 3.0                      & 464             \\ \hline
1.5 - 2.0                       & 125             & 3.0 - 4.0                      & 147             \\ \hline
\end{tabular}
\caption{Trajectory counts for simulation experiments by initial distances to target}
\end{table}

In this section, we provide additional details on our experimental step-up. We list our neural network hyperparameters in Table~\ref{tab:networkparams}. We used the Adam optimizer for all experiments with $\beta_{1}=0.9$, $\beta_{2}=0.999$, and learning rate $\alpha=0.001$. These were the default parameters in the deep learning framework we implemented our methods with \cite{paszke2019pytorch}. In all our experiments we used a mini-batch size of 32 for training all neural methods.

We collected trajectories as training data for each experiment. We ran an Ornstein and Uhlenbeck process \cite{uhlenbeck1930brownianmotion} with the following parameters: $\sigma=1.00$, $\mu=0.00$, $\theta=0.15$, $\theta$ here is not the same as model parameters. In our single point simulation, we used a training dataset of 100,000 (1000 trajectories of 100 time-steps each), and for the multi-point environment we used a training dataset of 200,000 (2000 trajectories of 100 times-steps). We re-used each random seeds training dataset for all models in our experiments. The one exception is the Neural Jacobian models which collected additional trajectories before training because each datum required sub-sequent steps to formulate a training example. 

For evaluation in both simulators, we generated 110 random targets for each of the 10 random seeds for a total of 1100 targets used for reported results. The targets were generated by uniform sampling in the joint angles and transforming them with the Kinova kinematics. This does not correspond with uniform sampling of the Cartesian work-space because of the transformations from the kinematic equations. We allowed each model 200 time-steps to reach the target which corresponded to 10 seconds of simulated time. In our experiments we set the gain value $\lambda=1.0$ which we found worked well for all methods.
 
 On the Kinova, we collected 10,000 training examples (100 trajectories of 100 time-steps) with the same Ornstein and Uhlenbeck process parameters. Unlike the simulator experiments, we re-used the same 10,000 samples for each random seed, meaning the random seed mostly affected initialization for the neural network parameters. We generated 25 random targets for each seed from the Kinova's kinematics bounded between $[-2.0, 2.0]$ for the first control joint and $[-1.5, 1.5]$ of the second joint. We only worked with 2 Joints of the Kinova, and discuss details of this in the next section. Targets were reused between all models considered. During evaluation, we used a gain $\lambda=0.9$ for for evaluation, but collected data with $\lambda = 1.0$.
