# Supplementary material for: Analyzing Neural Jacobian Methods in Applications of Visual Servoing and Kinematic Control
Source: arXiv:2106.06083 source file (2021-06-10)
Supplement: Supplementary file 11 [file violin_plots_to_target.tex]

\section*{Final Error Distribution}

These are just additional plots for our simulation results. Figure~\ref{fig:violint_pt_to_pt} shows the spread of the final euclidean distance to the target. 
\begin{figure}[ht]
    \centering
\includegraphics[width=\linewidth]{diagrams/pt_to_pt_sim_diagrams/pt_to_pt_violion_end_position.pdf}  
  \caption{Violin Plots of Final Positions. Plots Closer to zeros imply trajectories more likely to each target with method.}
    \label{fig:violint_pt_to_pt}
\end{figure}
